# Supplementary material for: Efficient and Effective Similar Subtrajectory Search with Deep Reinforcement Learning
Source: arXiv:2003.02542 source file (2020-07-14)
Supplement: Supplementary file 1 [file appendix.tex]

%\newpage
%{\color{red}
	\section{Quality Analysis of the SizeS Algorithm}
	\label{sec:sizes-proof}
	There usually exists a space, within which the objects move. Therefore, we assume the points of trajectories are all located in a $d_{max} \times d_{max}$ rectangle, where $d_{max}$ is a large number that captures the extent of the space. We use a coordinate system whose origin is at the middle of this rectangle.

	\smallskip\noindent\textbf{Case 1: DTW.}
	Consider a problem input with a query trajectory with $m$ points $T_q = <p_1', p_2', ..., p_m'>$ and a data trajectory with $n = m^2$ points $T = <p_{1,1}, p_{1,2}, ..., p_{1,m}, p_{2,1}, p_{2,2}, ..., p_{2,m}, ..., p_{m,1}, p_{m,2}, p_{m,m}>$. We assume that $m$ is an even number and $l = m / 2$. In addition, we let $d = d_{max} / m$.
	The locations of the points in these trajectories are provided as follows.
	\begin{itemize}
		\item $p_i' = ( - ( l - i + 1/2) \cdot d, 0)$ for $i = 1, 2, ..., l$;
		\item $p_i' = ( (i - l - 1/2) \cdot d, 0)$ for $i = l+1, l+2, ..., m$;
		\item $p_{i,j}$'s ($1\le j \le m$) are evenly located at the circle with its center at $p_i'$ and its radius equal to $\epsilon$, where $\epsilon$ is a very small real number for $i = 1, 2, ..., m$;
	\end{itemize}
	
	Consider the optimal solution. Its DTW distance, denoted by $D_o$, is at most the distance between $T$ and $T_q$, which is equal to $m^2\cdot \epsilon$ (points $p_{i,j}$ for $1\le j\le m$ are aligned with point $p_i'$ for $1\le i\le m$). That is, we have $D_o \le m^2 \cdot \epsilon$.
	
	Consider the approximate solution returned by SizeS.  Suppose that $\xi = 0$. That is, we only consider subtrajectories with the length exactly equal to $m$. We further know that each such sub-trajectory consists of points, either all located at a circle with the center at one of the point of $T_q$ or some located at a circle with the center at a point $p_i'$ and others located at a circle with the center at a point $p_{i+1}'$ ($1\le i < m$). It could be verified that among these subtrajectories, the one with some located at the circle with the center at $p_l'$ and others at $p_{l+1}'$ has the smallest DTW distance from $T_q$ and would be returned. We denote its DTW distance to $T_q$ by $D_a$. It could be verified that $D_a > 2\times (\Sigma_{i=1}^{l-1} ((l-i)\cdot d - \epsilon) + \epsilon)$, where the lower bound of the Euclidean distance from a point of $T_q$ to its aligned point of the returned subtrajectory is (1) $((l-i)\cdot d - \epsilon)$ for $1\le i\le l-1$ and (2) $\epsilon$ for $i = l$; and (3) that of the point symmetric to $p_i'$ (w.r.t. the origin) for $l+1\le i\le m$ due to the symmetry. Therefore, we have
	\begin{align*}
	\frac{D_a}{D_o}
	& \ge \frac{2\times (\Sigma_{i=1}^{l-1} ((l-i)\cdot d - \epsilon) + \epsilon)}{m^2 \cdot \epsilon}\\
	& = \frac{m^2/4\cdot d - m/2\cdot d - m\cdot \epsilon + 4\cdot\epsilon}{m^2\cdot \epsilon} \\
	&= \frac{1/4\cdot d - 1/(2m)\cdot d - \epsilon/m + 4/m^2\cdot \epsilon}{\epsilon}
	\end{align*}
	which approaches infinity when m approaches infinity and $\epsilon$ approaches 0.
	In summary, the solution returned by SizeS could be arbitrarily worse than the optimal one when DTW distance is used.
	
	\smallskip\noindent\textbf{Case 2: Frechet and t2vec.}
	Consider the case when Frechet distance is used. The optimal solution and the approximate solution returned would be the sames as the case when DTW distance is used, but the distances would be different. $D_o$ would be equal to $\epsilon$ and $D_a$ would be at least $((l-1)\cdot d - \epsilon)$. Therefore, we have
	$$
	\frac{D_a}{D_o} \ge \frac{(l-1)\cdot d - \epsilon}{\epsilon}
	$$
	which approaches infinity when $\epsilon$ approaches 0.
	
	Consider the case when t2vec is used. Since it is a learning-based distance - in theory, it may reduce to any possible distance metric such as DTW and Frechet. Thus, the analysis for DTW or Frechet could be carried over for t2vec.
	
	\if 0
	We provide a theoretical guarantee on the rank for SizeS algorithm. SizeS enumerates all subtrajectories with the sizes within the range $[m-\xi, m+\xi]$, where $m$ is the length of query trajectory and $\xi$ is a controllable parameter. During the search process, we know SizeS will traverse $(n-m+1)(2\xi+1)$ subtrajectories and return the best one among them. We can safely assume the worst case is the subtrajectories tried by SizeS are the worst (i.e., smallest similarity) in all $\frac{n(n+1)}{2}$ subtrajectories in $T$. Thus, the rank is bounded by $\frac{n(n+1)}{2}-(n-m+1)(2\xi+1)+1$. The tightness of the bound is controllable by the parameter $\xi$.
	\fi

	\section{Quality Analysis of Spliting-based Algorithms}
	\label{sec:splitting-proof}
	
	\smallskip\noindent\textbf{Case 1: PSS with DTW.}
	Consider a problem input with a data trajectory with $n+3$ points $T=<p_1', p_2', p_1, p_2, ..., p_n, p_3'>$ ($n$ is a positive integer) and a query trajectory $T_q = <p'>$. Let $d = d_{max}/2$. The locations of the points in these trajectories are provided as follows.
	\begin{itemize}
		\item $p_1' = (-d/2, 0)$, $p_2' = (-d, 0)$;
		\item $p_i = (0, 0)$ for $i = 1, 2, ..., n$;
		\item $p_3' = (d, 0)$;
		\item $p' = (0, \epsilon)$, where $\epsilon$ is a very small non-negative real number;
	\end{itemize}
	
	Consider the optimal solution. It could be any subtrajectory $<p_i>$ ($1\le i \le n$) and the corresponding DTW distance is equal to $\epsilon$, which we denote by $D_o$.
	
	Consider the approximate solution returned by PSS. It is the subtrajectory $<p_1'>$, which is explained as follows. When it scans the first point $p_1'$, it would split the trajectory at $p_1'$ and update the best-known subtrajectory to be $<p_1'>$ with the DTW distance equal to $\sqrt{d^2/4 + \epsilon^2}$. It then continues to scan the following points $p_2', p_1, ..., p_n, p_3'$ and would not perform any split operations at these points due to the fact that $p_2'$ and $p_3'$ are farther away from $p'$ than $p_1'$. As a result, $<p_1'>$ would be returned as a solution. We denote the DTW distance of this solution by $D_a$, i.e., $D_a = \sqrt{d^2/4 + \epsilon^2}$.
	
	Consider the approximation ratio (AR). We have
	$$
	\frac{D_a}{D_o} = \frac{\sqrt{d^2/4 + \epsilon^2}}{\epsilon} > \frac{d/2}{\epsilon}
	$$
	which approaches infinity when $\epsilon$ approaches zero.
	
	Consider the mean rank (MR). We know that the rank of the approximate solution $<p_1'>$ is at least $\frac{n(n+1)}{2}+1$ since any subtrajectory of $<p_1, p_2, ..., p_n>$ has a smaller DTW distance than $<p_1'>$ (assuming $\epsilon = 0$). Therefore, the mean rank would approach infinity when $n$ approaches infinity.
	
	Consider the relative rank (RR). Based on the analysis of mean rank, we know that the relative rank of the approximate solution $<p_1'>$ is at least $\frac{\frac{n(n+1)}{2}+1}{\frac{(n+3)(n+4)}{2}}$, which approaches 1 when $n$ approaches infinity.
	
	In conclusion, the solution returned by PSS could be arbitrarily worse than the optimal one in terms of AR, MR, and RR, when the DTW distance is used.
	
	\smallskip\noindent\textbf{Case 2: Other Algorithms and Similarity Measurements}
	Consider the other algorithms, i.e., POS and POS-D. It could be verified that they would run exactly in the same way as PSS on the problem input provided in the Case 1. Therefore, the conclusion would be carried over. Consider the other measurements, namely, Frechet and t2vec. For Frechet, it could be verified that the optimal solution and the approximate solution returned by the algorithms are the same as those in the Case 1 and their Frechet distances and DTW distances to $T_q$ are equal since both solutions and $T_q$ involve one single point. As a result, the conclusion for DTW distance could be carried over for Frechet distance. For t2vec, since it is a learning-based distance - in theory, it may reduce to any possible distance metric such as DTW and Frechet. Thus, the analysis for DTW in the Case 1 could be carried over for t2vec.
	
%}

\if 0
\section*{B. Arbitrary worse for splitting-based algorithms (PSS, POS and POS-D)}
\label{splitting-proof}
We prove the splitting-based algorithms are arbitrary worse by constructing the following cases for the approximation ratio and rank, respectively.
\subsection*{B.1 Approximation ratio analysis}
We consider two adjacent positions in a trajectory are bounded by a distance $d_{bound}$ and construct the case as follows:
\begin{equation*}
\begin{aligned}
&T=<p_1,p_2,\underbrace{...}_{k \text{ points}},p_*,\underbrace{...}_{k \text{ points}},p_n>, \text{and } T_q=<p_*>,
\end{aligned}
\end{equation*}
where we instantiate the similarity with trajectory distance (e.g., DTW or Frechet by default) denoted by $D(\cdot,\cdot)$ and $dist(\cdot,\cdot)$ denotes the distance between the points (typically the Euclidean distance). Let $D(<p_1>, T_q) = d_1$, $dist(p_2, p_*) = d_2$ and $dist(p_n, p_*) = d_3$, we construct $d_1 < d_2$ and $d_1 < d_3$ and then we prove it is arbitrary worse for approximation ratio under the construction.

Run the splitting-based algorithms (PSS, POS and POS-D), we find a splitting is happened on $p_1$ due to the initial condition of these algorithms. Then, we choose to maintain the subtrajectory $<p_1>$ with the distance $d_1$ because it is smaller. We continue to scan the trajectory $T$, and we find no splitting will happen because we cannot find a smaller distance than $d_1$ from prefix $<p_2,...,p_i>$ and suffix $<p_i,...,p_n>$ for $2\leq i \leq n$ due to the boundary condition (recall the distance definition) of DTW or Frechet. Finally, these algorithms output subtrajectory $<p_1>$ with distance $d_1$ as results. Under the construction $d_1<d_2$, we can let the three points $p_1$, $p_2$ and $p_*$ form a triangle. Then, we have
\begin{equation*}
\begin{aligned}
&dist(p_1,p_*)+dist(p_1,p_2)>dist(p_2, p_*)\\
&d_1>d_2-dist(p_1,p_2)>d_2-d_{bound}\\
\end{aligned}
\end{equation*}
We know there is $k$ points between $p_2$ and $p_*$. we may assume $d_2=(k+1)*d_{bound}$, i.e., these points are collinear with the adjacent distance $d_{bound}$. Then, we further have
\begin{equation*}
\begin{aligned}
&d_1>(k+1)*d_{bound}-d_{bound}=k*d_{bound}\\
\end{aligned}
\end{equation*}
We know $d_1$ increases as $k$ increases; however, the distance for the optimal solution is 0 because $T_q=<p_*>$ is a portion of $T$. Thus, the difference between the optimal distance and the approximate distance approaches arbitrary worse.

\subsection*{B.2 Rank analysis}
\label{splitting-proof-rank}
We construct the following case for rank analysis.
\begin{equation*}
\begin{aligned}
&T=<p_1,p_2,\underbrace{p_*,...,p_*}_{k \text{ points}},p_n>, \text{and } T_q=<p_*>.
\end{aligned}
\end{equation*}
Here, we assume an object stays at position $p_*$ and GPS collects $k$ same points $p_*$ in the trajectory $T$. Similarly, we let $D(<p_1>, T_q) = d_1$, $dist(p_2, p_*) = d_2$ and $dist(p_n, p_*) = d_3$ and construct $d_1 < d_2$, $d_1 < d_3$. Based on the above analysis, we know splitting-based algorithms return the subtrajectory $<p_1>$ with the distance $d_1$, and there are $\frac{k(k+1)}{2}$ subtrajectories formed by the $k$ points with trajectory distance 0. Thus, the rank for these splitting-based algorithms is larger than $\frac{k(k+1)}{2}$ at least, and it increases as $k$ increases. The rank is also arbitrary worse.

\section*{C. Arbitrary worse for learning-based algorithms (RLS, RLS-Skip)}
We proof learning-based algorithms (RLS, RLS-Skip) is also arbitrary worse based on approximation ratio and rank analysis, respectively.
\subsection*{C.1 Approximation ratio analysis}
We construct the following case:
\begin{equation*}
\begin{aligned}
T=<p_1,\underbrace{...}_{k \text{ points}},p_*,\underbrace{...}_{k \text{ points}},p_n>, \text{and } T_q=<p_*>,
\end{aligned}
\end{equation*}
We use the same notations as defined in the proof above. Let $dist(p_1, p_*) = d_1$ and $dist(p_n, p_*) = d_2$. We know learning-based algorithms can output arbitrary actions because it is a data-driven method. We consider the case of all actions are 0, which means no splitting will be happened during the MDP, and it will try $2*n$ subtrajectories that is prefix $<p_1, ... , p_i>$ and suffix $<p_i, ... , p_n>$ for $1 \leq i\leq n$. Similarly, we instantiate the trajectory similarity by DTW or Frechet distance, and we discuss the following two situations:
\begin{enumerate}
	\item If the returned subtrajectory from prefix $<p_1,..., p_i>$, we know $D(<p_1,..., p_i>, T_q) \geq dist(p_1, p_*)=d_1$ by DTW or Frechet definition. We know there are $k$ points between $p_1$ and $p_*$. We may assume $d_1 = (k + 1)*d_{bound}$ by constructing these points collinear with the adjacent distance $d_{bound}$. Then, $d_1$ will increase as $k$ increases; however, the distance outputted by the optimal solution is 0. Thus, the proof holds based on prefix analysis.
	\item Similarly, if the returned subtrajectory from suffix $<p_i,...,p_n>$, we know $D(<p_i,..., p_n>, T_q) \geq dist(p_n, p_*)=d_2$, and we can let the points between $p_*$ and $p_n$ collinear with the adjacent distance $d_{bound}$. Then, $d_2 = (k + 1)*d_{bound}$, and the distance difference between the optimal and the approximate is also arbitrary worse as $k$ increases.
\end{enumerate}
\subsection*{C.2 Rank analysis}
Similar to rank analysis above. We construct the following case and let all actions are 0 outputted by learning-based algorithms.
\begin{equation*}
\begin{aligned}
&T=<p_1,\underbrace{p_*,...,p_*}_{k \text{ points}},p_n>, \text{and } T_q=<p_*>.
\end{aligned}
\end{equation*}
We know there are $\frac{k(k+1)}{2}$ subtrajectories formed by the $k$ same points $p_*$ with the trajectory distance 0. However, the returned distance of learning-based algorithms is either larger than $d_1$ or $d_2$ outputted by prefix or suffix, respectively. Thus, the rank of learning-based algorithms is larger than $\frac{k(k+1)}{2}$ at least, and it increases as $k$ increases. The proof for arbitrary worse based on rank holds.
\fi

\section{Adaption of UCR}
\label{section:ucr-and-spring}
%\smallskip\noindent\textbf{Adaption of UCR.}
\if 0
UCR Suite~\cite{rakthanmanon2012searching} studied a related but different problem that we consider.
The target of UCR Suite is to exactly search a subsequence that has the same length as the query in a given long sequence, which usually contains a large number of elements even reaches trillion levels.
Thus, the paper proposed a suite of techniques to prune unpromising subsequences before the exact distance computations (i.e., DTW). We conclude the following techniques in UCR Suite based on \cite{mueen2016extracting,rakthanmanon2012searching,rakthanmanon2013addressing} and present how to adapt them to trajectory data.
\fi
%\smallskip\noindent\textbf{Adaption of UCR.}
UCR~\cite{rakthanmanon2012searching} was originally developed for searching subsequences of a time series, which are the most similar to a query time series and the similarity is based on the DTW distance. Specifically, UCR enumerates all subsequences that are of the same length of the query time series and employs a rich set of techniques for pruning many of the subsequences.
%Spring is designed for the problem of finding a subsequence of a data time series, which is the most similar to a query time series.
We use UCR for our ``similar subtrajectory search'' problem by adapting UCR's pruning techniques for trajectories. UCR involves seven techniques used for pruning, organized in two groups.
Let $T = <p_1, p_2, ..., p_n>$ be a data trajectory and $T_q = <q_1, q_2, ..., q_m>$ be a query trajectory. Suppose we are considering a subtrajectory of $T$, denoted by $T'=<p_1, p_2, ..., p_m>$ without loss of generality. We describe the adaptions of the techniques involved in UCR, which are used to prune $T'$ from being considered if possible as follows.
\\
Group 1: Known Optimizations
\begin{itemize}
  \item Early Abandoning of $LB_{Keogh}$.
  This is to compute a lower bound called $LB_{Keogh}$ of the DTW distance between $T'$ and $T_q$, denoted by $LB_{Keogh}(T', T_q)$, and prune $T'$ if the lower bound is larger than the best-known DTW distance. Specifically, let (1) $R\in[0,1]$ be a real number, (2)
  $q_{i-\lfloor R\cdot m\rfloor: i+\lfloor R\cdot m\rfloor}$ be the set involving $\lfloor R\cdot m\rfloor$ points before $q_i$, $\lfloor R\cdot m\rfloor$ points after $q_i$, and point $p_i$, and (3) $MBR(\cdot)$ be the minimum bounding box of a set of points.
  We compute $LB_{Keogh}(T', T_q)$ as follows.
  \begin{small}
  	\begin{equation*}
  	LB_{Keogh}(T', T_q)= \sum_{i=1}^{m} \left\{
  	\begin{aligned}
  	& d(p_i, MBR(q_{i-\lfloor R\cdot m\rfloor: i+\lfloor R\cdot m\rfloor})) \\
  	& \text{ if $p_i$ outside $MBR(q_{i-\lfloor R\cdot m\rfloor: i+\lfloor R\cdot m\rfloor})$}\\
  	& 0 \text{ otherwise}
  	\end{aligned}
  	\right.
  	\end{equation*}
  \end{small}
  where $d(p_i, MBR(\cdot))$ denotes shortest distance between $p_i$ and $MBR(\cdot)$.
  \if 0
  We adapt $LB_{Keogh}$ for trajectory data. Due to trajectory is a sequence of time-stamped locations, we use an upper curve and a lower curve to envelop trajectory from Y-axis and a left curve and a right curve to envelop trajectory from X-axis. Similarly, we use the Sakoe-Chiba band $r$ to define allowed range of warping for the four envelops followed the idea of $LB_{Keogh}$, that is:
  \begin{equation*}
  \begin{aligned}
    &UP_{i} = \max(p_{y_{i-r}:y_{i+r}}), LO_{i} = \min(p_{y_{i-r}:y_{i+r}})\\
    &LE_{i} = \min(p_{x_{i-r}:x_{i+r}}), RI_{i} = \max(p_{x_{i-r}:x_{i+r}})
  \end{aligned}
  \end{equation*}
  Note that when the ratio of Sakoe-Chiba band is set to 100\% (i.e., $r=100\%\times|Q|$), DTW becomes unconstrained and the four envelops become a Minimum Bounding Rectangle (MBR) of trajectory. Further, we adapt $LB_{Keogh}$ definition as follows:
  \begin{small}
  \begin{equation*}
  LB_{Keogh}(Q,C)= \sum_{i=1}^{n} \left\{
  \begin{aligned}
  & \min(d(c_i,UP_i),d(c_i,LO_i), d(c_i,LE_i),\\
  &d(c_i,RI_i)) \text{ if $c_i$ outside envelops}\\
  & 0 \text{ otherwise}
  \end{aligned}
  \right.
  \end{equation*}
  \end{small}
  where trajectory $Q$ is enclosed in the bounding envelopes, and $d(\cdot,\cdot)$ denotes the distance (typically Euclidean distance). The time complexity of $LB_{Keogh}$ is $O(n)$, which is a cheap-to-compute lower bound to prune off unpromising candidates for DTW computation when it is larger than $best$\_$so$\_$far$.
  \fi

  \item Early Abandoning of DTW. During the process of computing the DTW distance between $T'$ and $T_q$, when the accumulated DTW distance exceeds the best-known DTW distance, we abandon the computation.

  \item Earlier Early Abandoning of DTW using $LB_{Keogh}$.
  \if 0
  After defined the $LB_{Keogh}$ for trajectory data, we follow a tighter lower bound, that is $DTW(Q_{1:K},C_{1:K}) + LB_{Keogh}(Q_{K+1:n},C_{K+1:n})$ as a new lower bound to the true DTW distance (i.e., $DTW(Q_{1:n},C_{1:n}))$ when we incrementally compute a partial DTW from 1 to $K$ with the summation of the other partial $LB_{Keogh}$ from $K+1$ to $n$. Then, We can stop DTW calculation if the lower bound exceeds the $best$\_$so$\_$far$ distance at any time.
  \fi
  For $i = 1, 2, ..., m$, if the sum of the DTW distance between $T_q[1:i]$ and any prefix of $T'[1:i]$ (or between $T'[1:i]$ and any prefix of $T_q[1:i]$) and the $LB_{Keogh}$ bound between $T_q[i:m]$ and $T'[i:m]$ is larger than the best-known DTW distance, we prune $T'$. Note that DTW distances used in this pruning are maintained in the process of computing the DTW distance between $T'$ and $T_q$.
\end{itemize}
Group 2: Novel Optimizations in UCR Suite.
\begin{itemize}
  \item Just-in-time Z-normalizations. We do not adapt the Z-normalization technique since it is designed for one-dimensional data and cannot be used for trajectory data that is two-dimensional.
  \item Reordering Early Abandoning.
  %In UCR, it orders points by expected contribution based on the absolute values of the Z-normalized $T$ for the $LB_{Keogh}$ calculation rather than simply accumulating the distance from left to right. Similarly,
  % We determine the ordering by sorting the distances from the mean on Y-axis. The intuition behind this idea is that a trajectory point may contribute a larger distance if it deviates further.
  We consider the points of $T_q$ in a descending order of their distances to the y-axis for computing the bound of $LB_{Keogh}$.

  \item Reversing $LB_{Keogh}$.
  %We also envelop candidate trajectory $C$ and calculate the lower bound denoted by $LB_{Keogh}EC$.
  We reverse the roles of $T'$ and $T_q$ and compute another $LB_{Koegh}$ bound. We then use the larger one among the two $LB_{Koegh}$ bounds to act as a tighter $LB_{Keogh}$ bound when necessary.

  \item Cascading Lower Bounds.
  We first compute the $LB_{Kim}FL$ bound, which is another simple lower bound of the DTW distance between $T'$ and $T_q$, denoted by $LB_{Kim}FL(T', T_q)$. Specifically, $LB_{Kim}FL(T', T_q)$ is defined as  $(d(T_q[1], T'[1]) + d(T_q[m], T'[m]))$. The time complexity of this step is simply $O(1)$. If this bound does not help to prune $T'$, we cascade the techniques of early abandoning of $LB_{Keogh}$, early abandoning of DTW, and earlier early abandoning of DTW using $LB_{Keogh}$. Finally, if $T'$ has still not been pruned, we compute the DTW distance between $T'$ and $T_q$.
\end{itemize}
We note that UCR is designed specifically for the DTW distance and cannot be used for the problem when the Frechet or t2vec distance is used.

%\begin{table}
%\centering
%\scriptsize
%%\vspace{-2mm}
%\caption{Comparison with UCR Suite.}
%\begin{tabular}{|c|c|c|c|c|}
%\hline
%Algorithms & AR & MR & RR &  Time (s)\\ \hline
%UCR Suite  &1.737 &490.947 &59.5\% &1807\\
%RLS  &1.039 &45.521 &4.7\% &890\\
%RLS-Skip+ &1.136 &145.624 &14.3\% &96\\\hline
%\end{tabular}
%%\vspace{-4mm}
%\label{para_steps}
%\end{table}
\if 0
\begin{figure}[!th]
\centering
\begin{tabular}{c c}
  \begin{minipage}{4cm}%5.5
	\includegraphics[width=4.2cm]{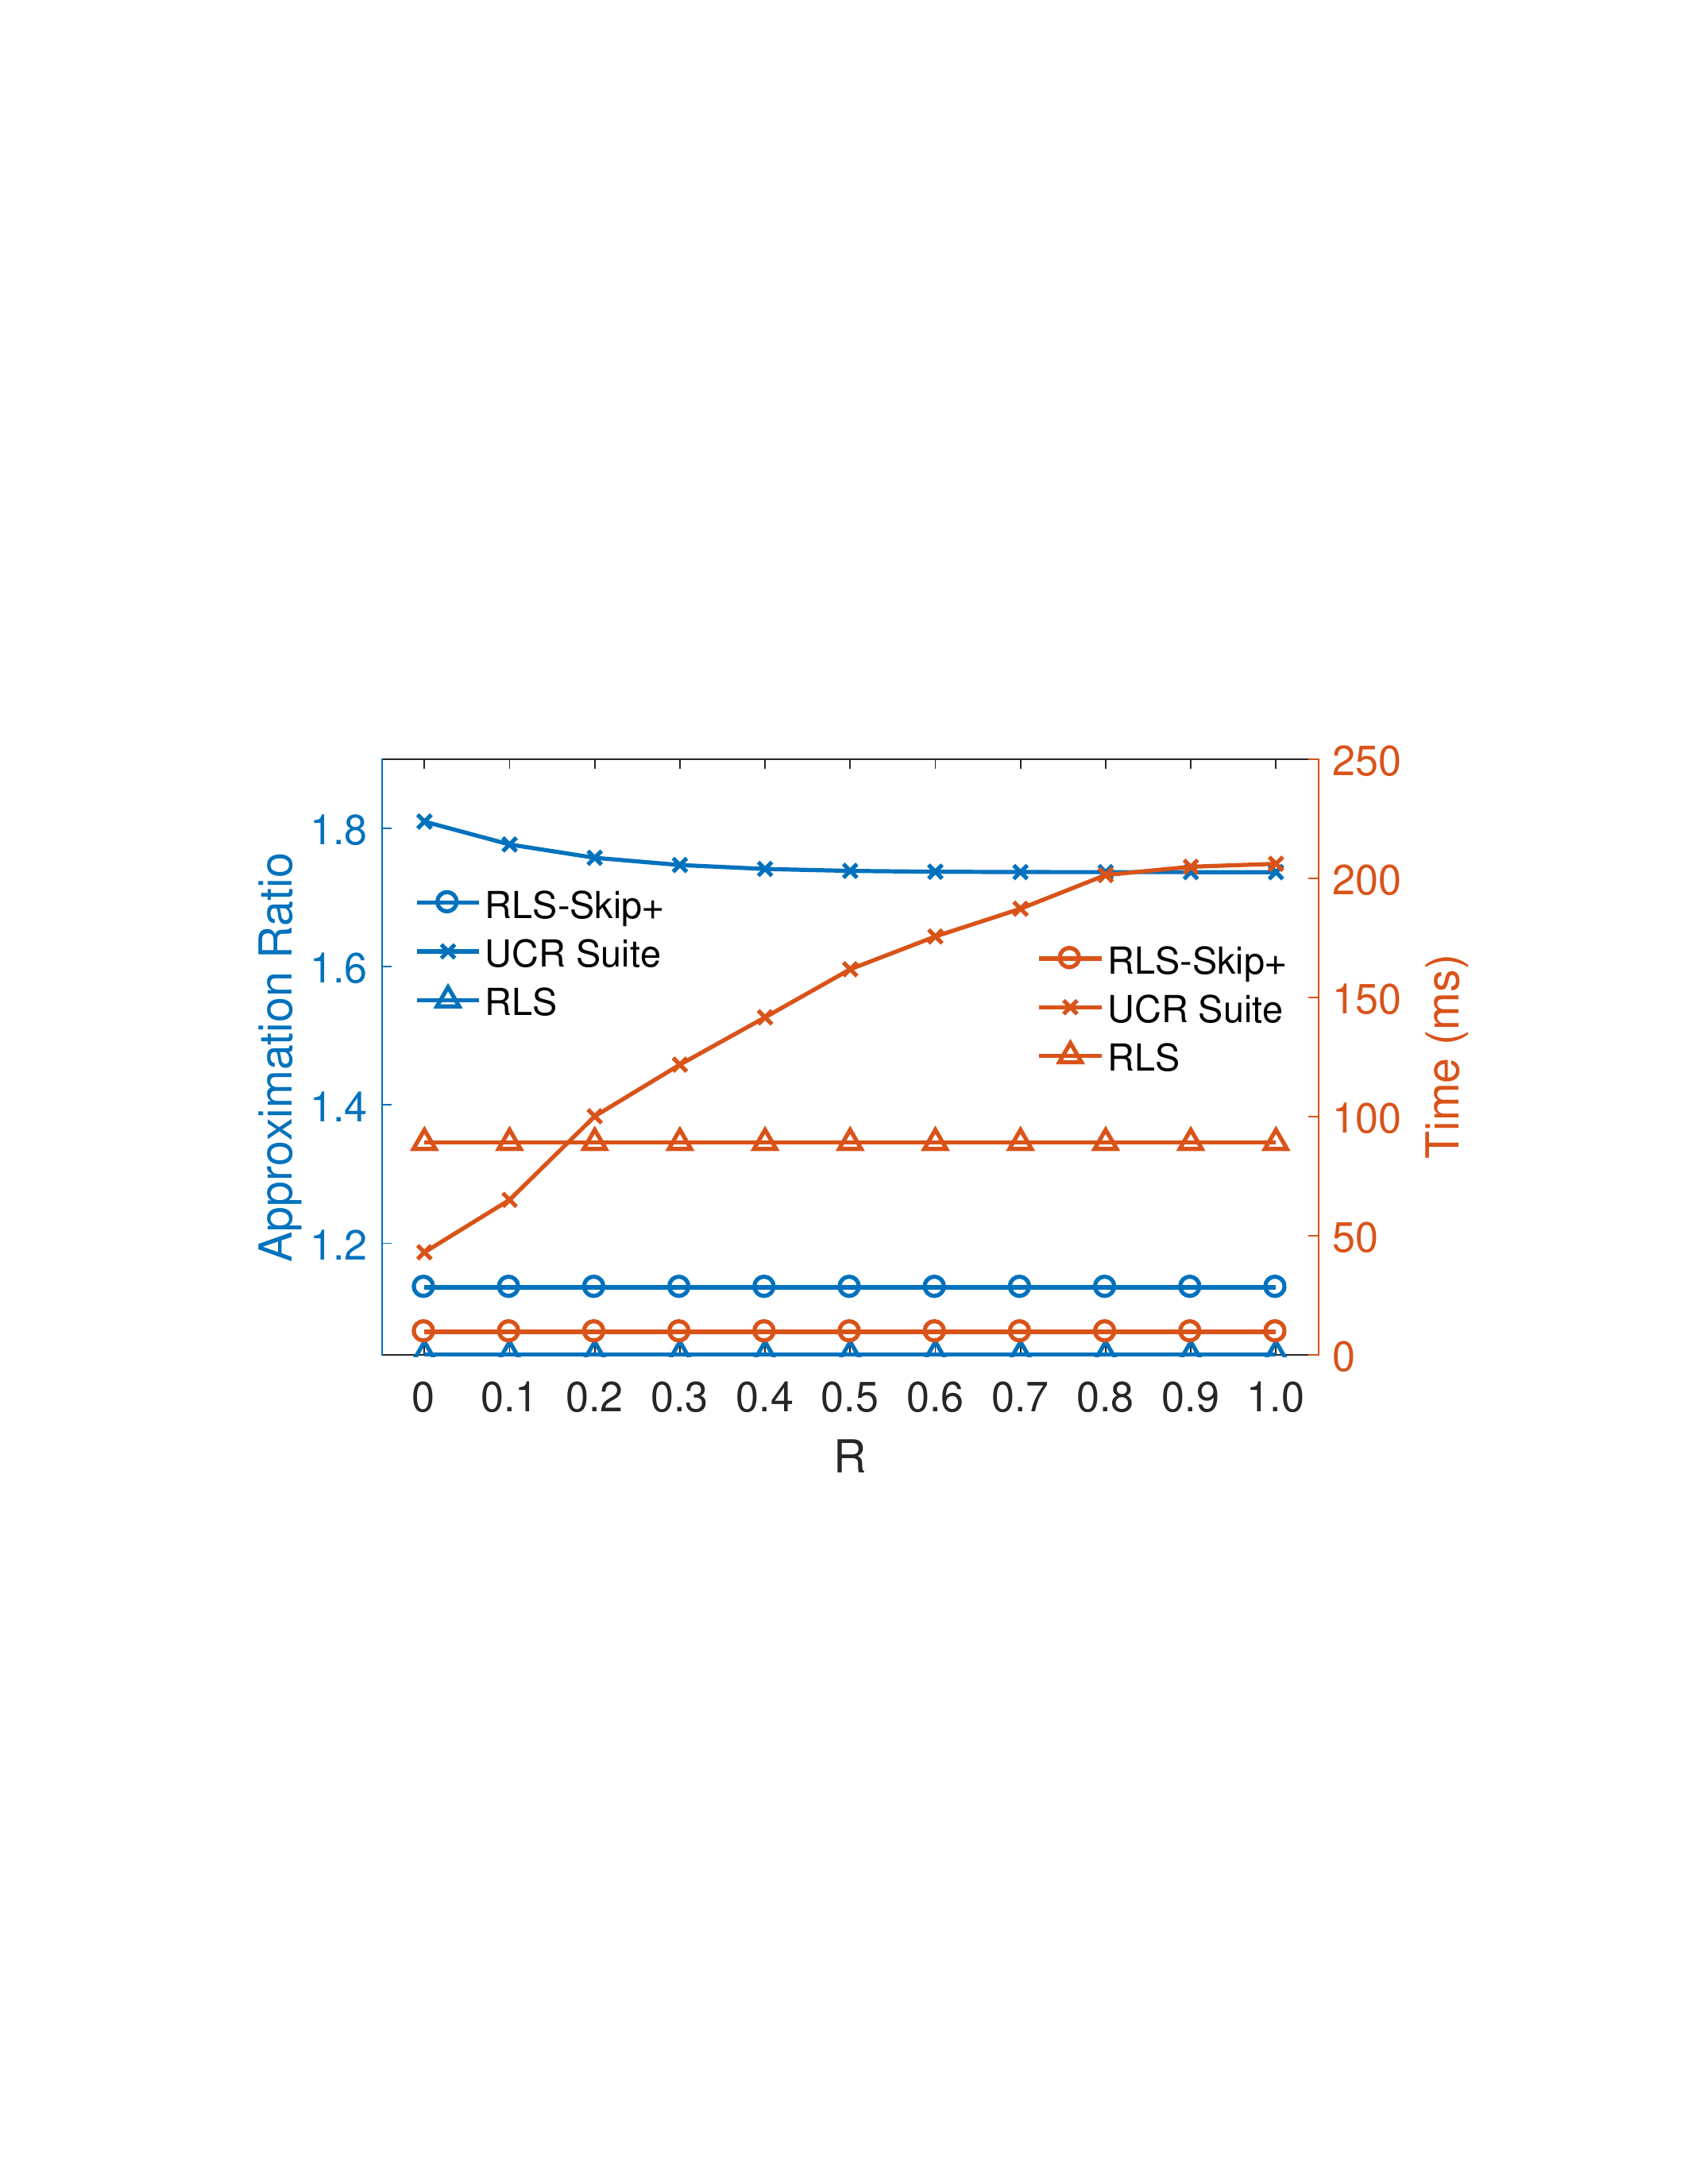}
  \end{minipage}
  &
  \begin{minipage}{4cm}%5.5
	\includegraphics[width=4.2cm]{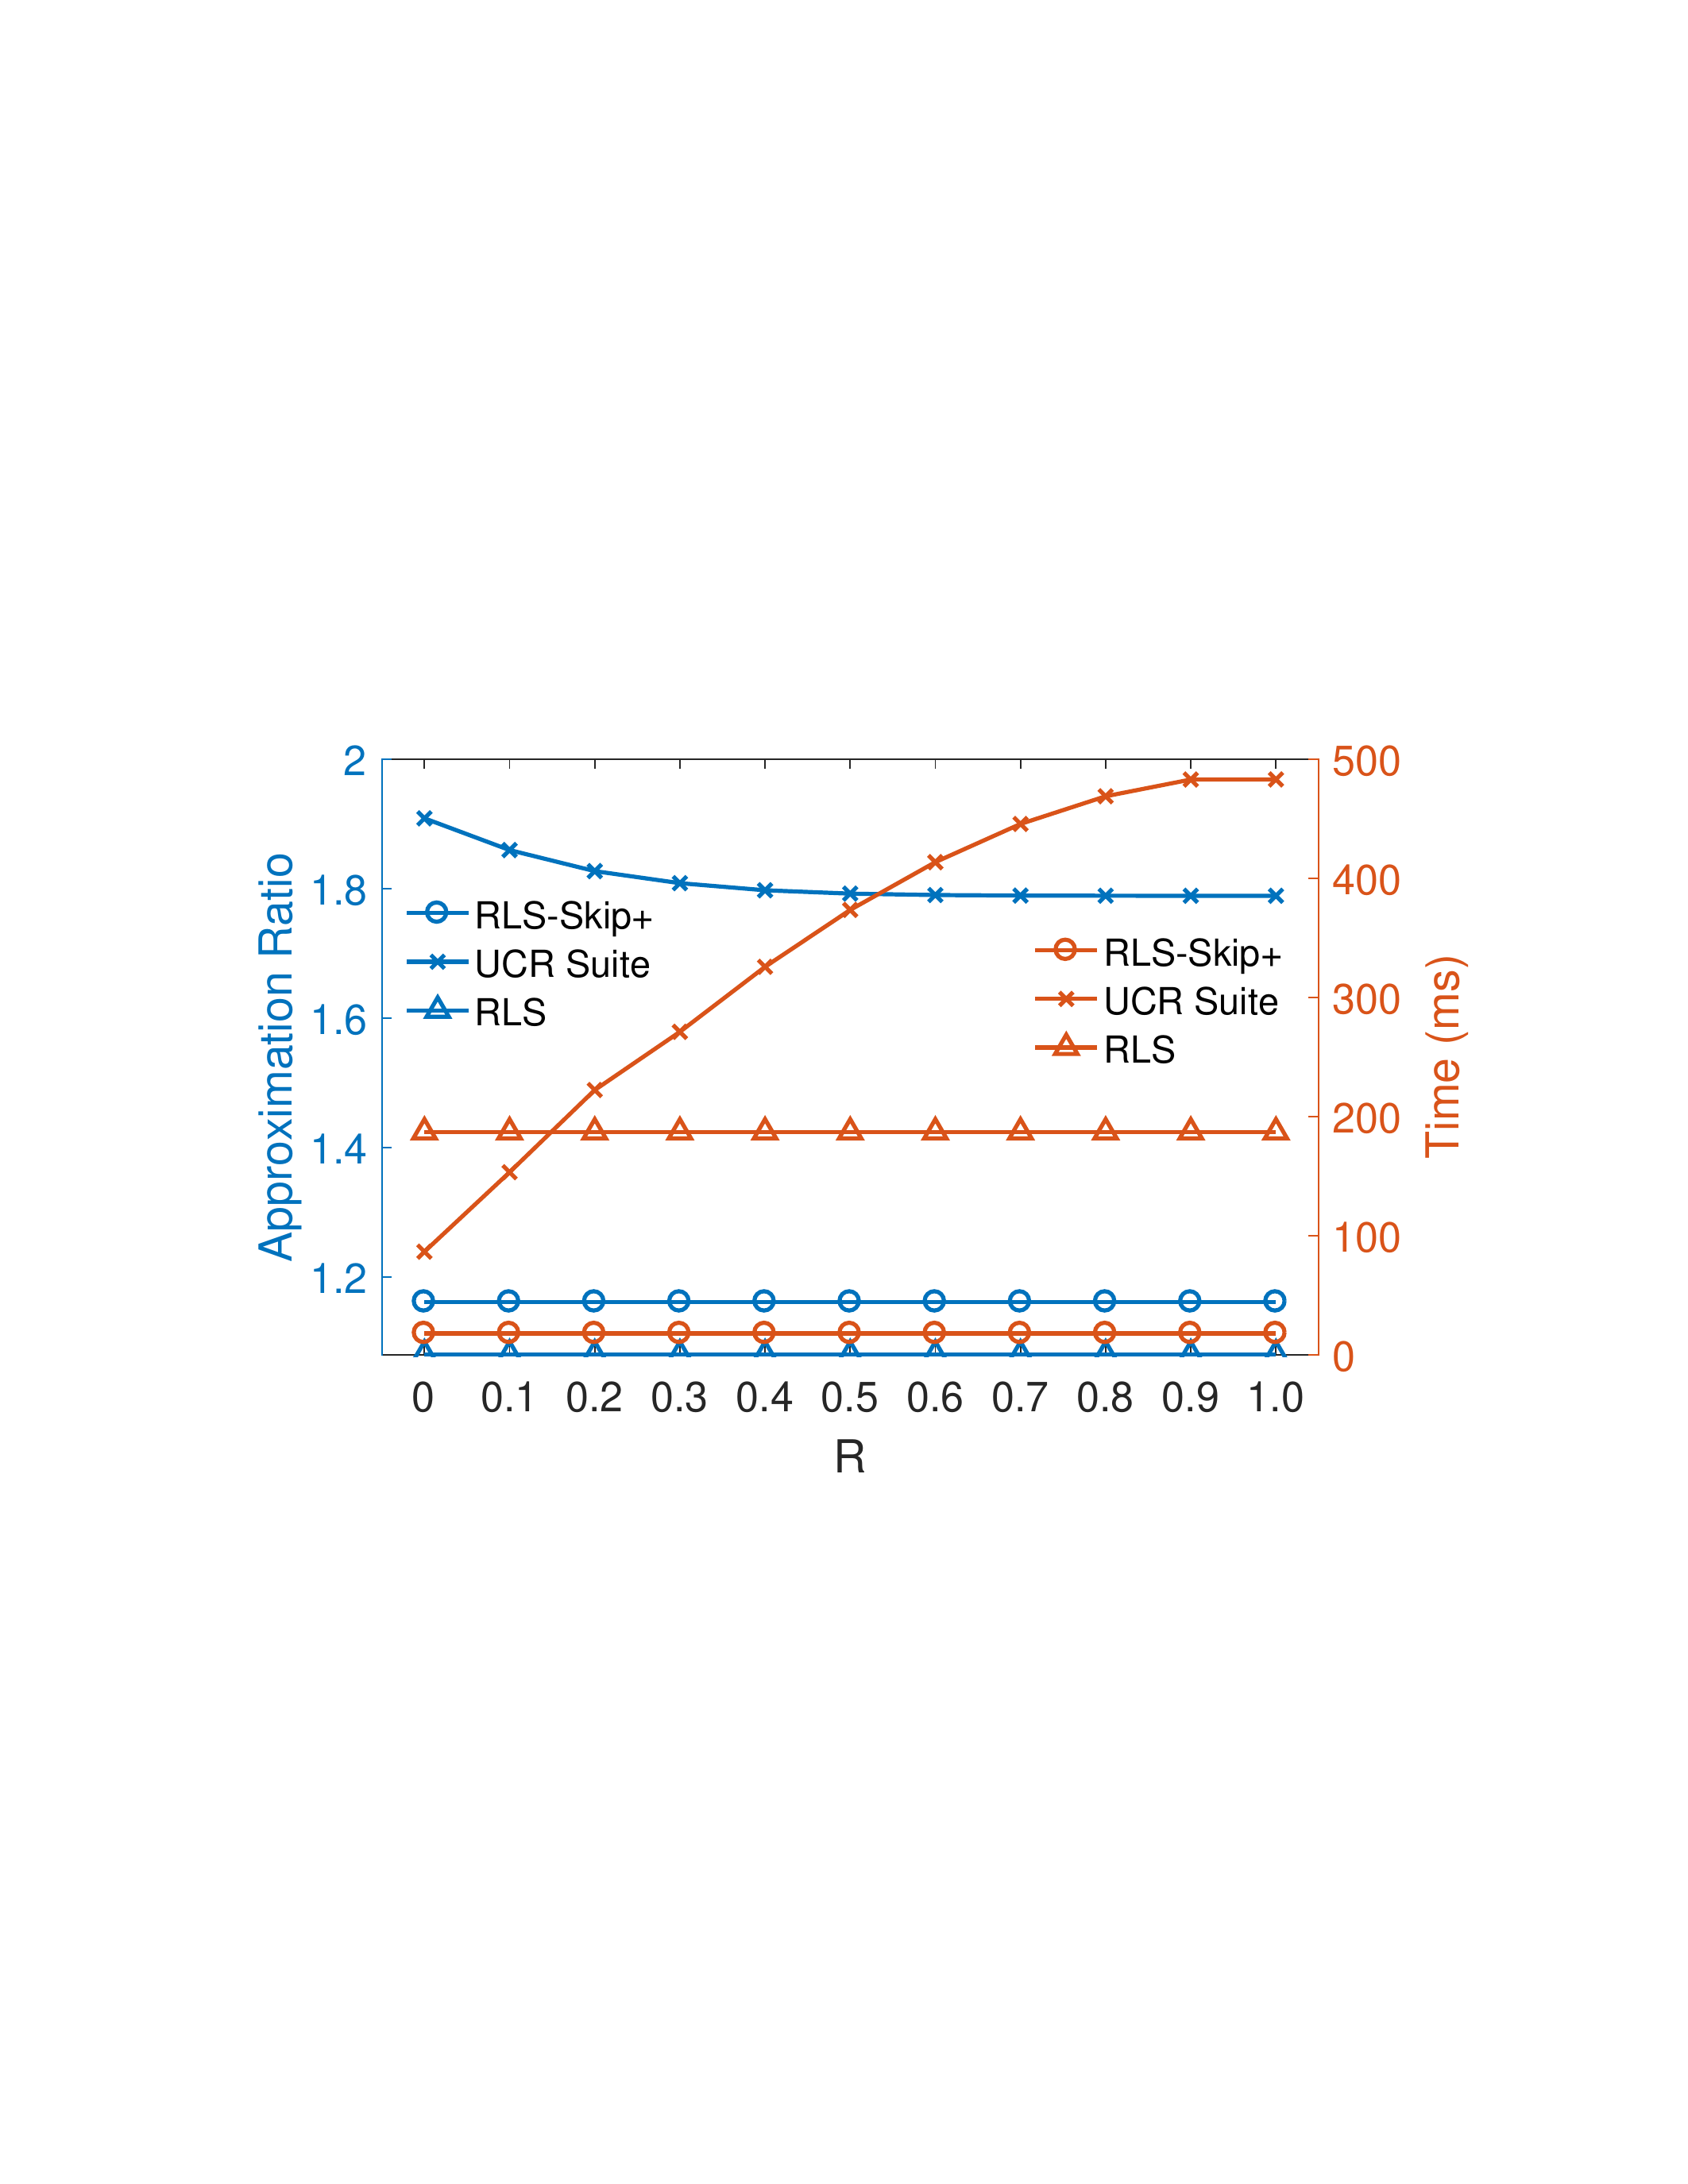}
  \end{minipage}
  \\
  \scriptsize{(a) Porto}
  &
  \scriptsize{(b) Harbin}
  \end{tabular}
\caption{Comparison with UCR Suite.}
\label{ucr_result}
%\vspace*{-2mm}
\end{figure}

\begin{figure}[!th]
\centering
\begin{tabular}{c c}
  \begin{minipage}{4cm}%5.5
	\includegraphics[width=4.2cm]{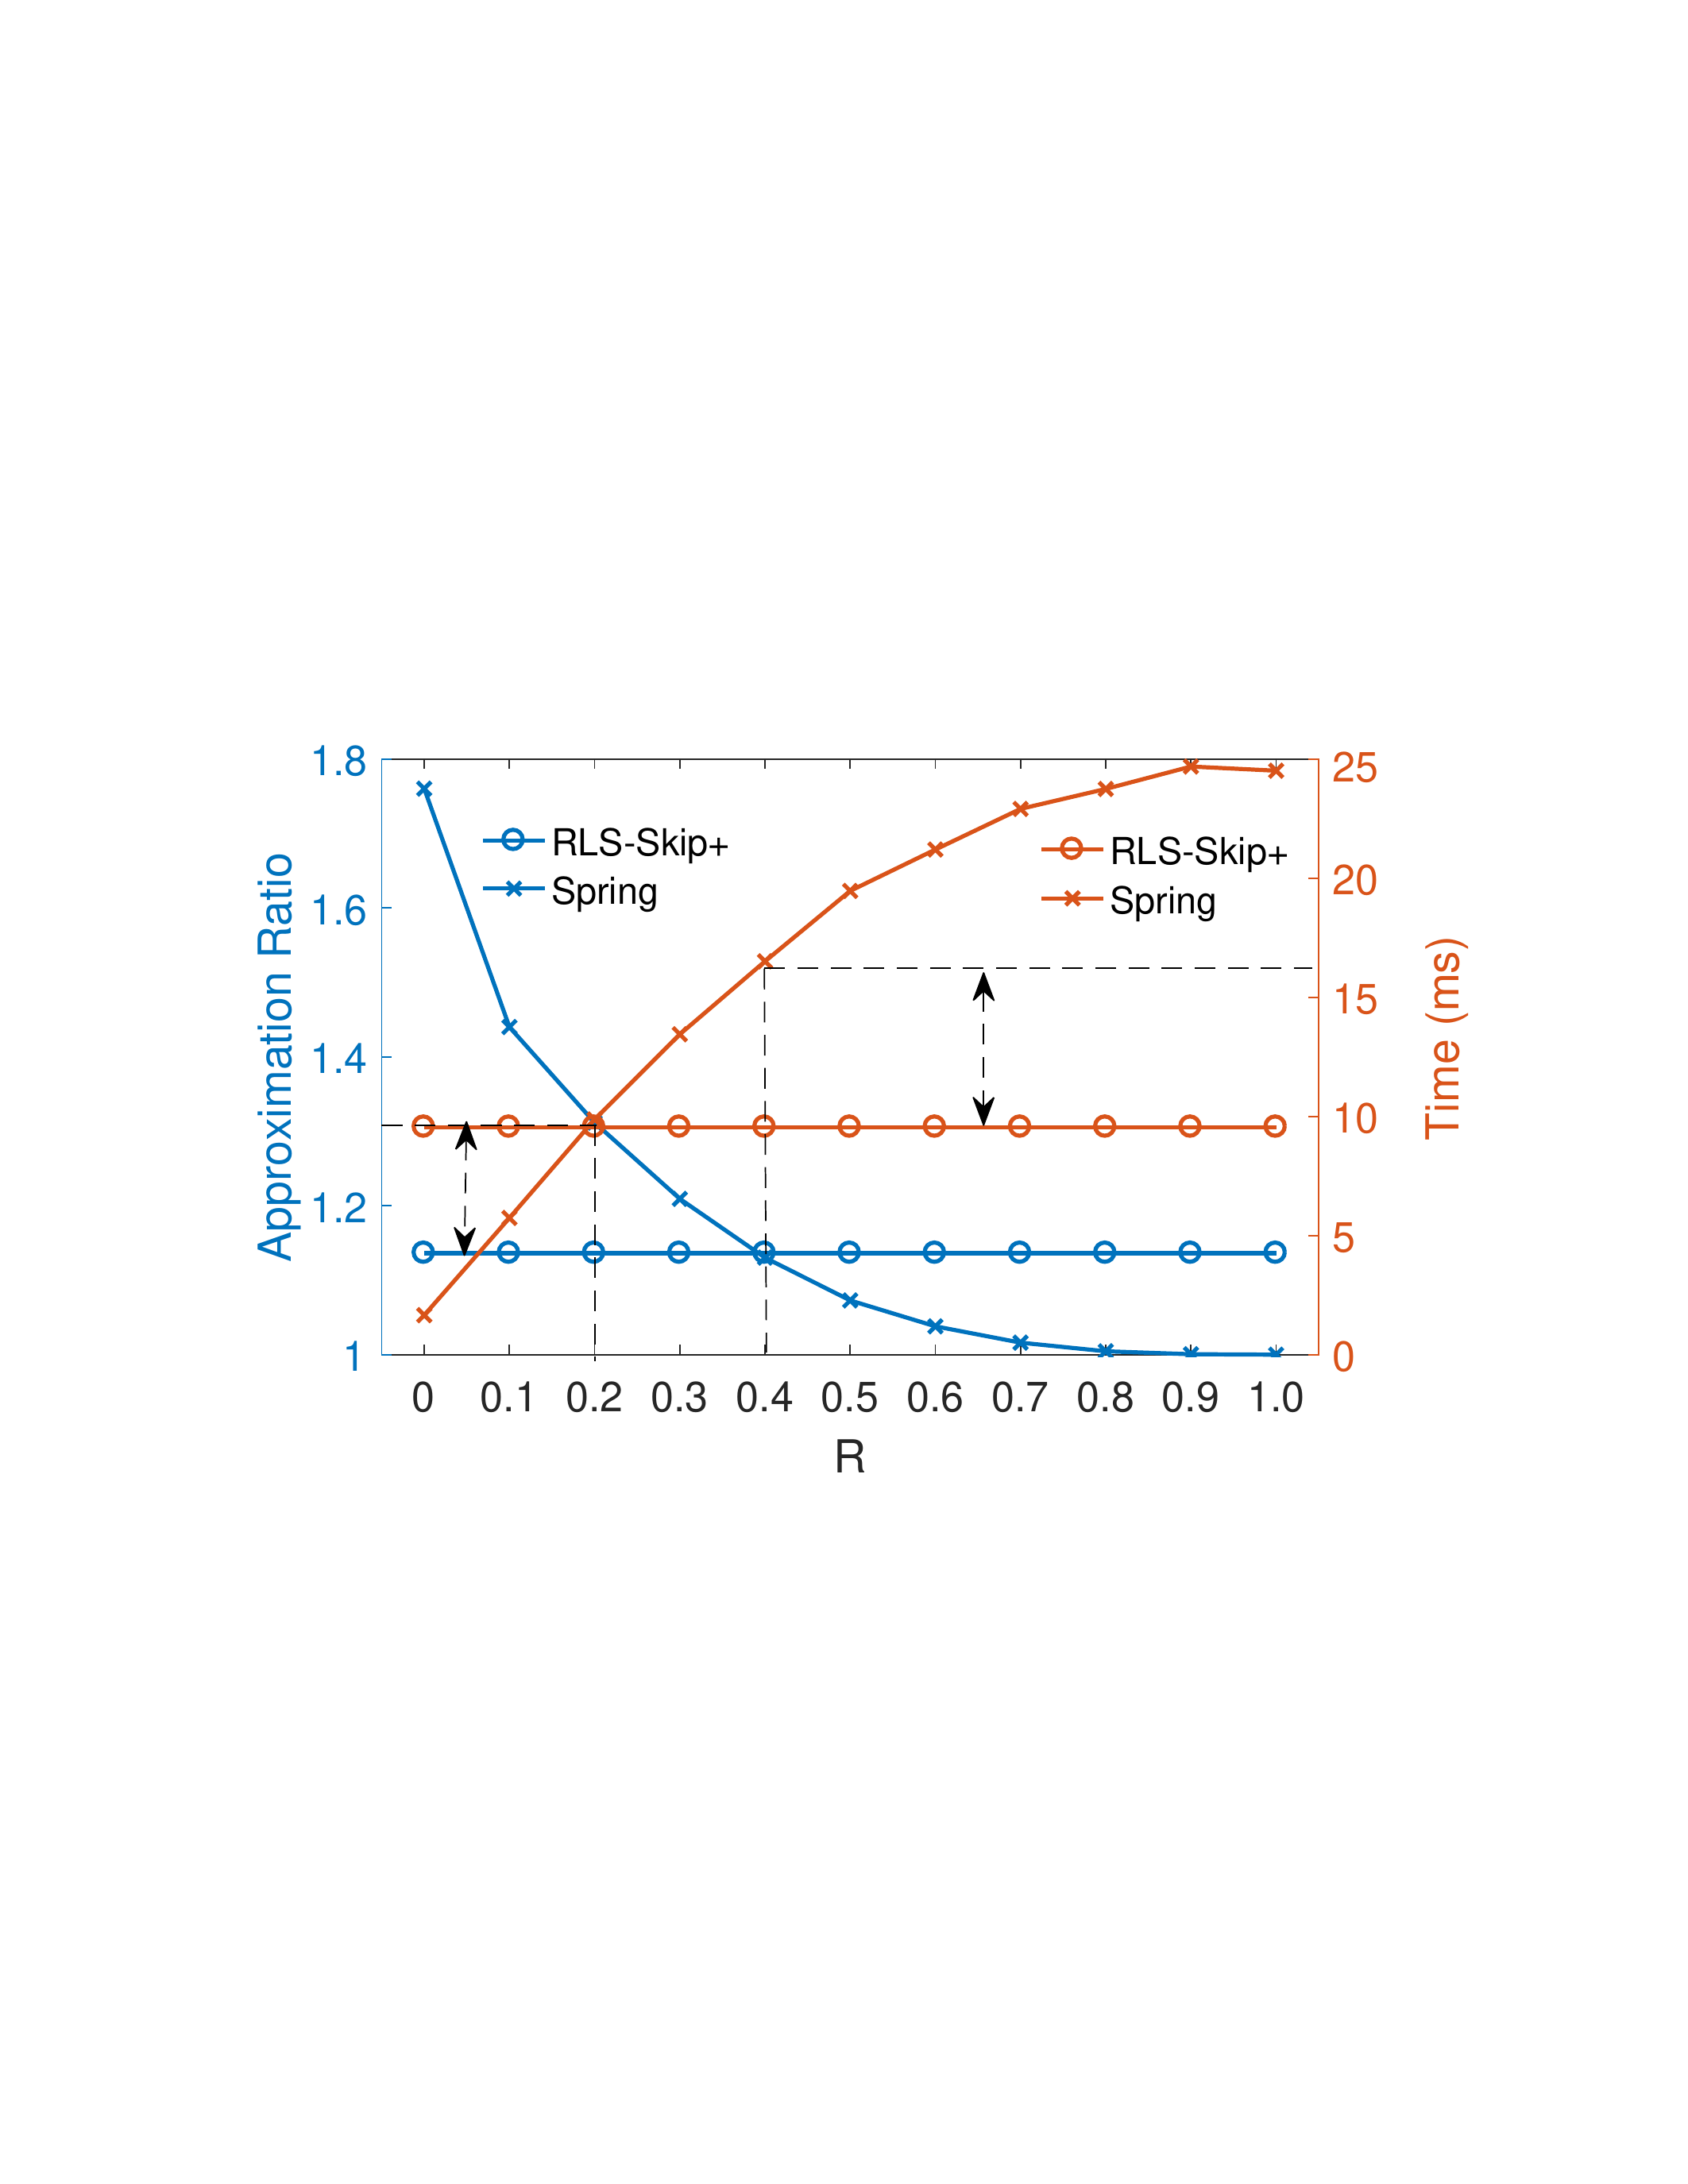}
  \end{minipage}
  &
  \begin{minipage}{4cm}
	\includegraphics[width=4.2cm]{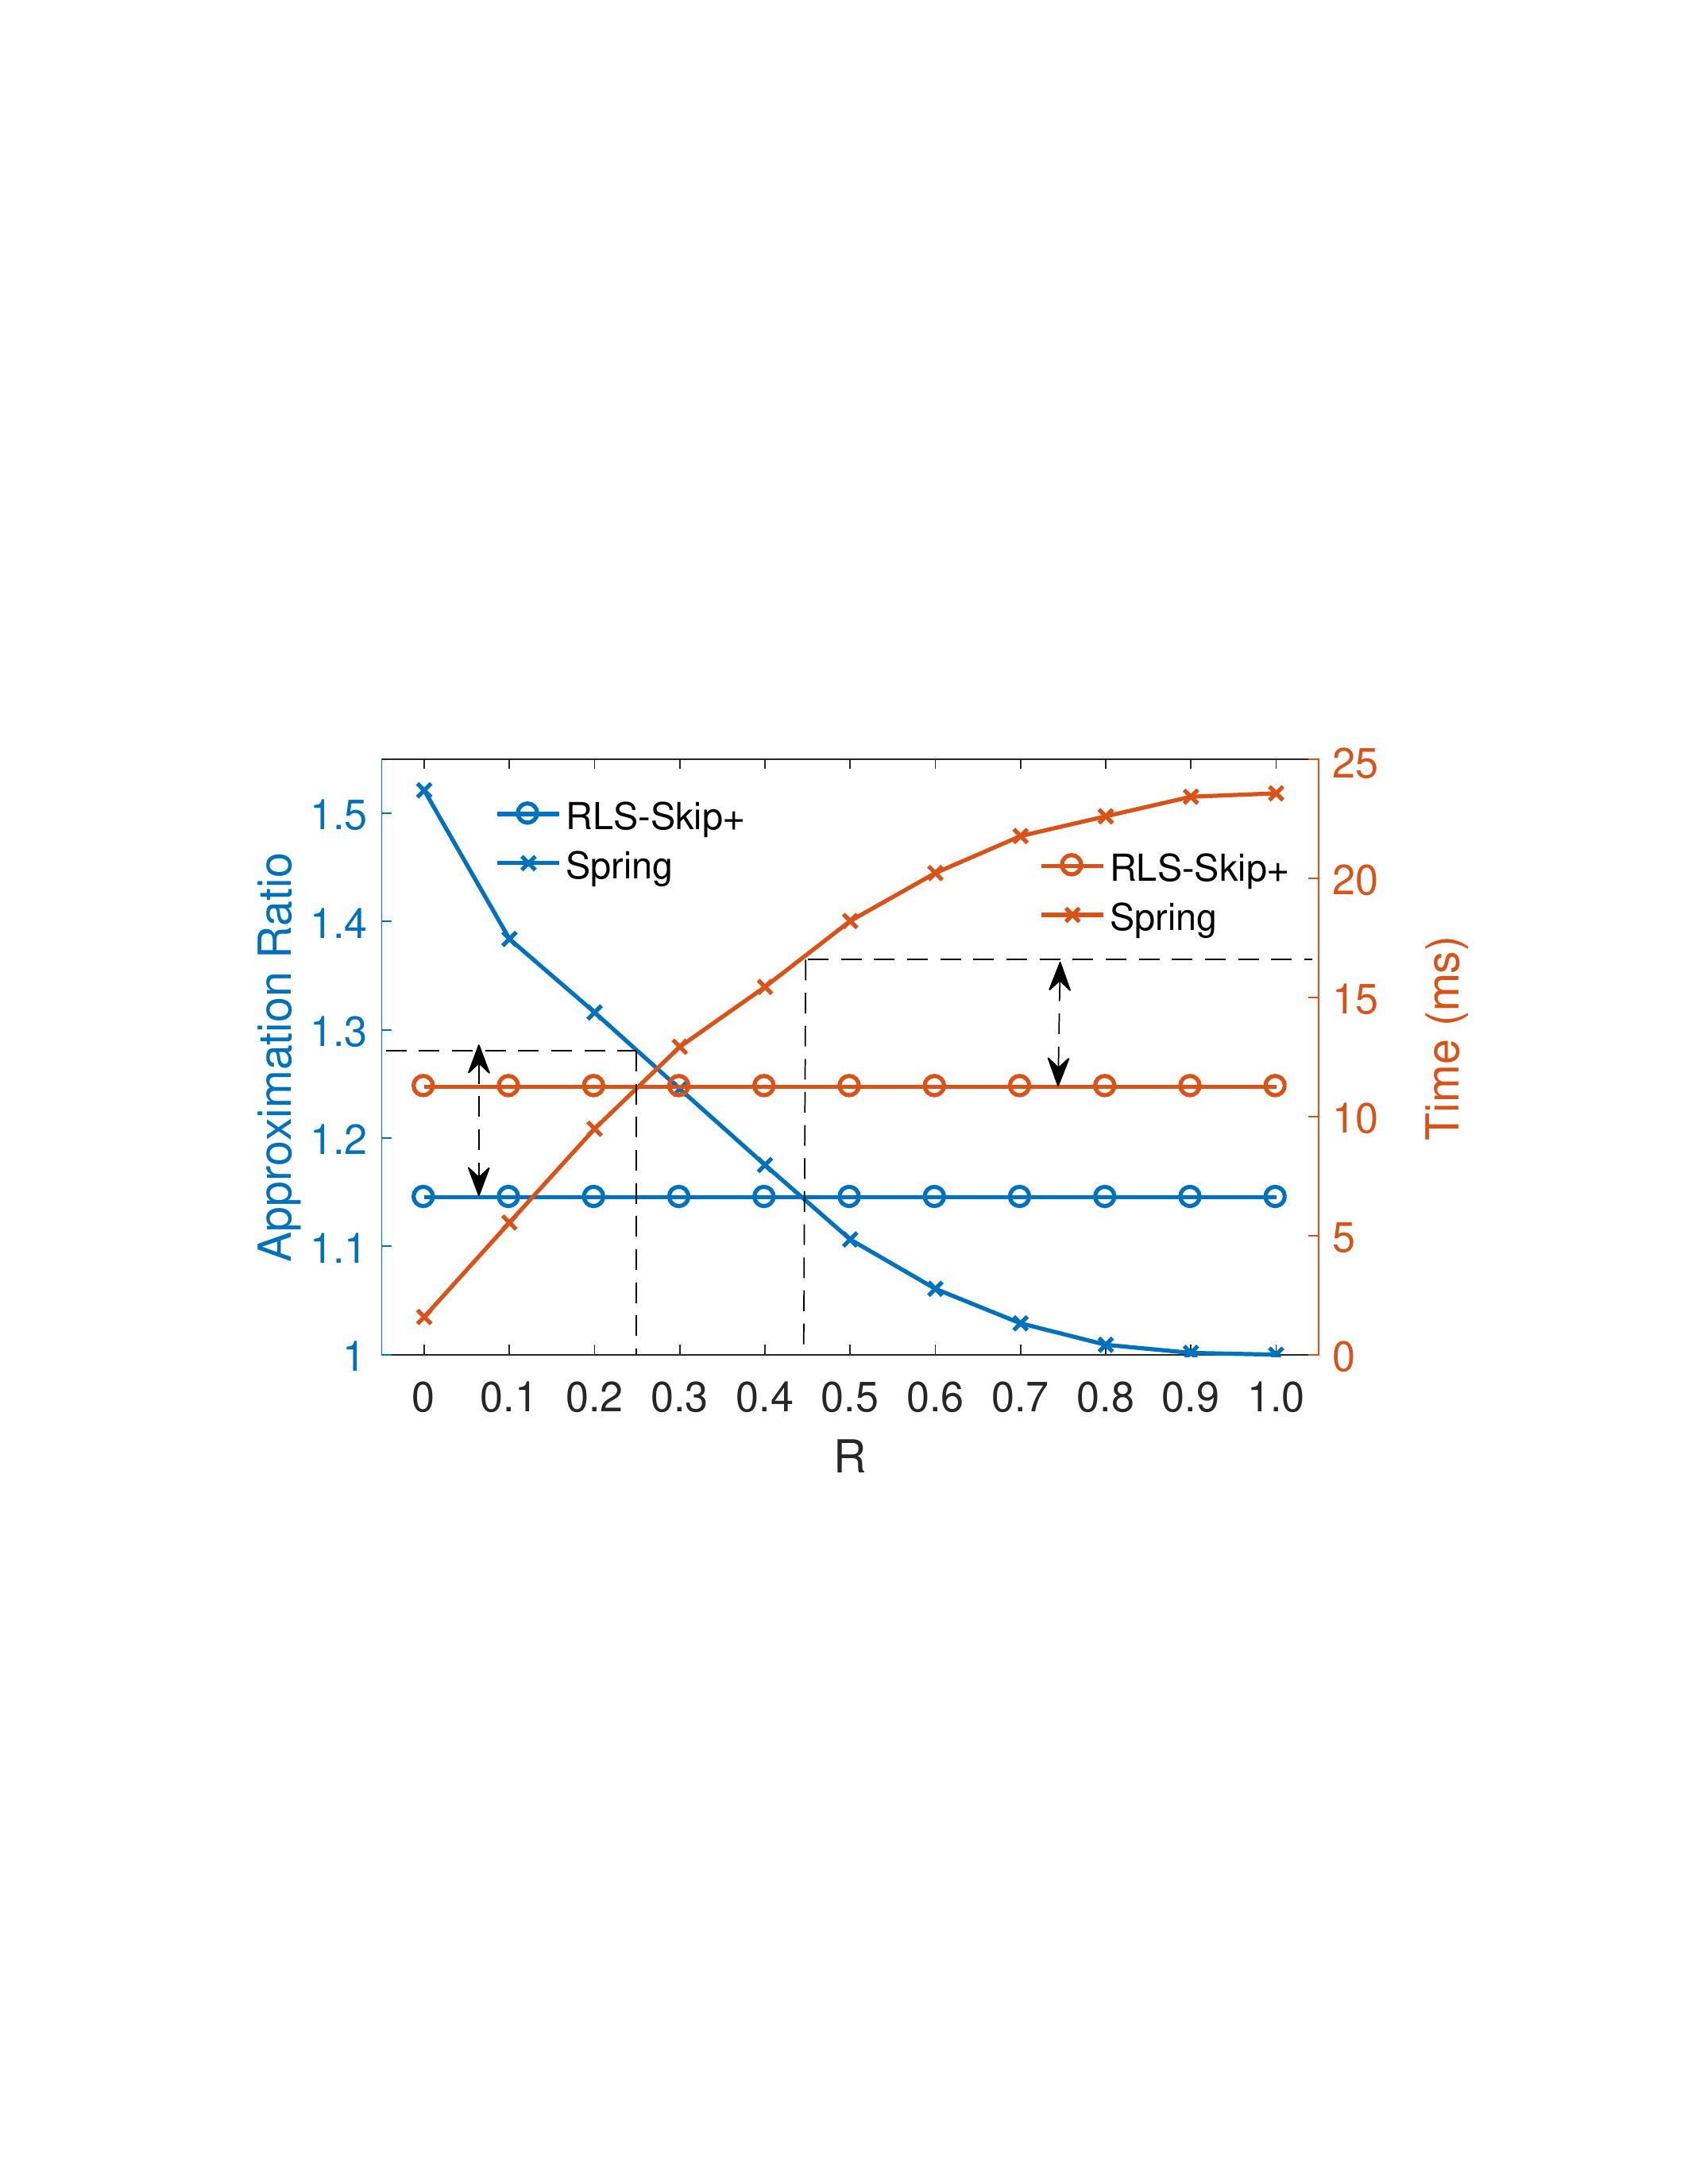}
  \end{minipage}
  \\
  \scriptsize{(a) Porto (DTW)}
  &
  \scriptsize{(b) Porto (Frechet)}
  \\
  \begin{minipage}{4cm}%5.5
	\includegraphics[width=4.2cm]{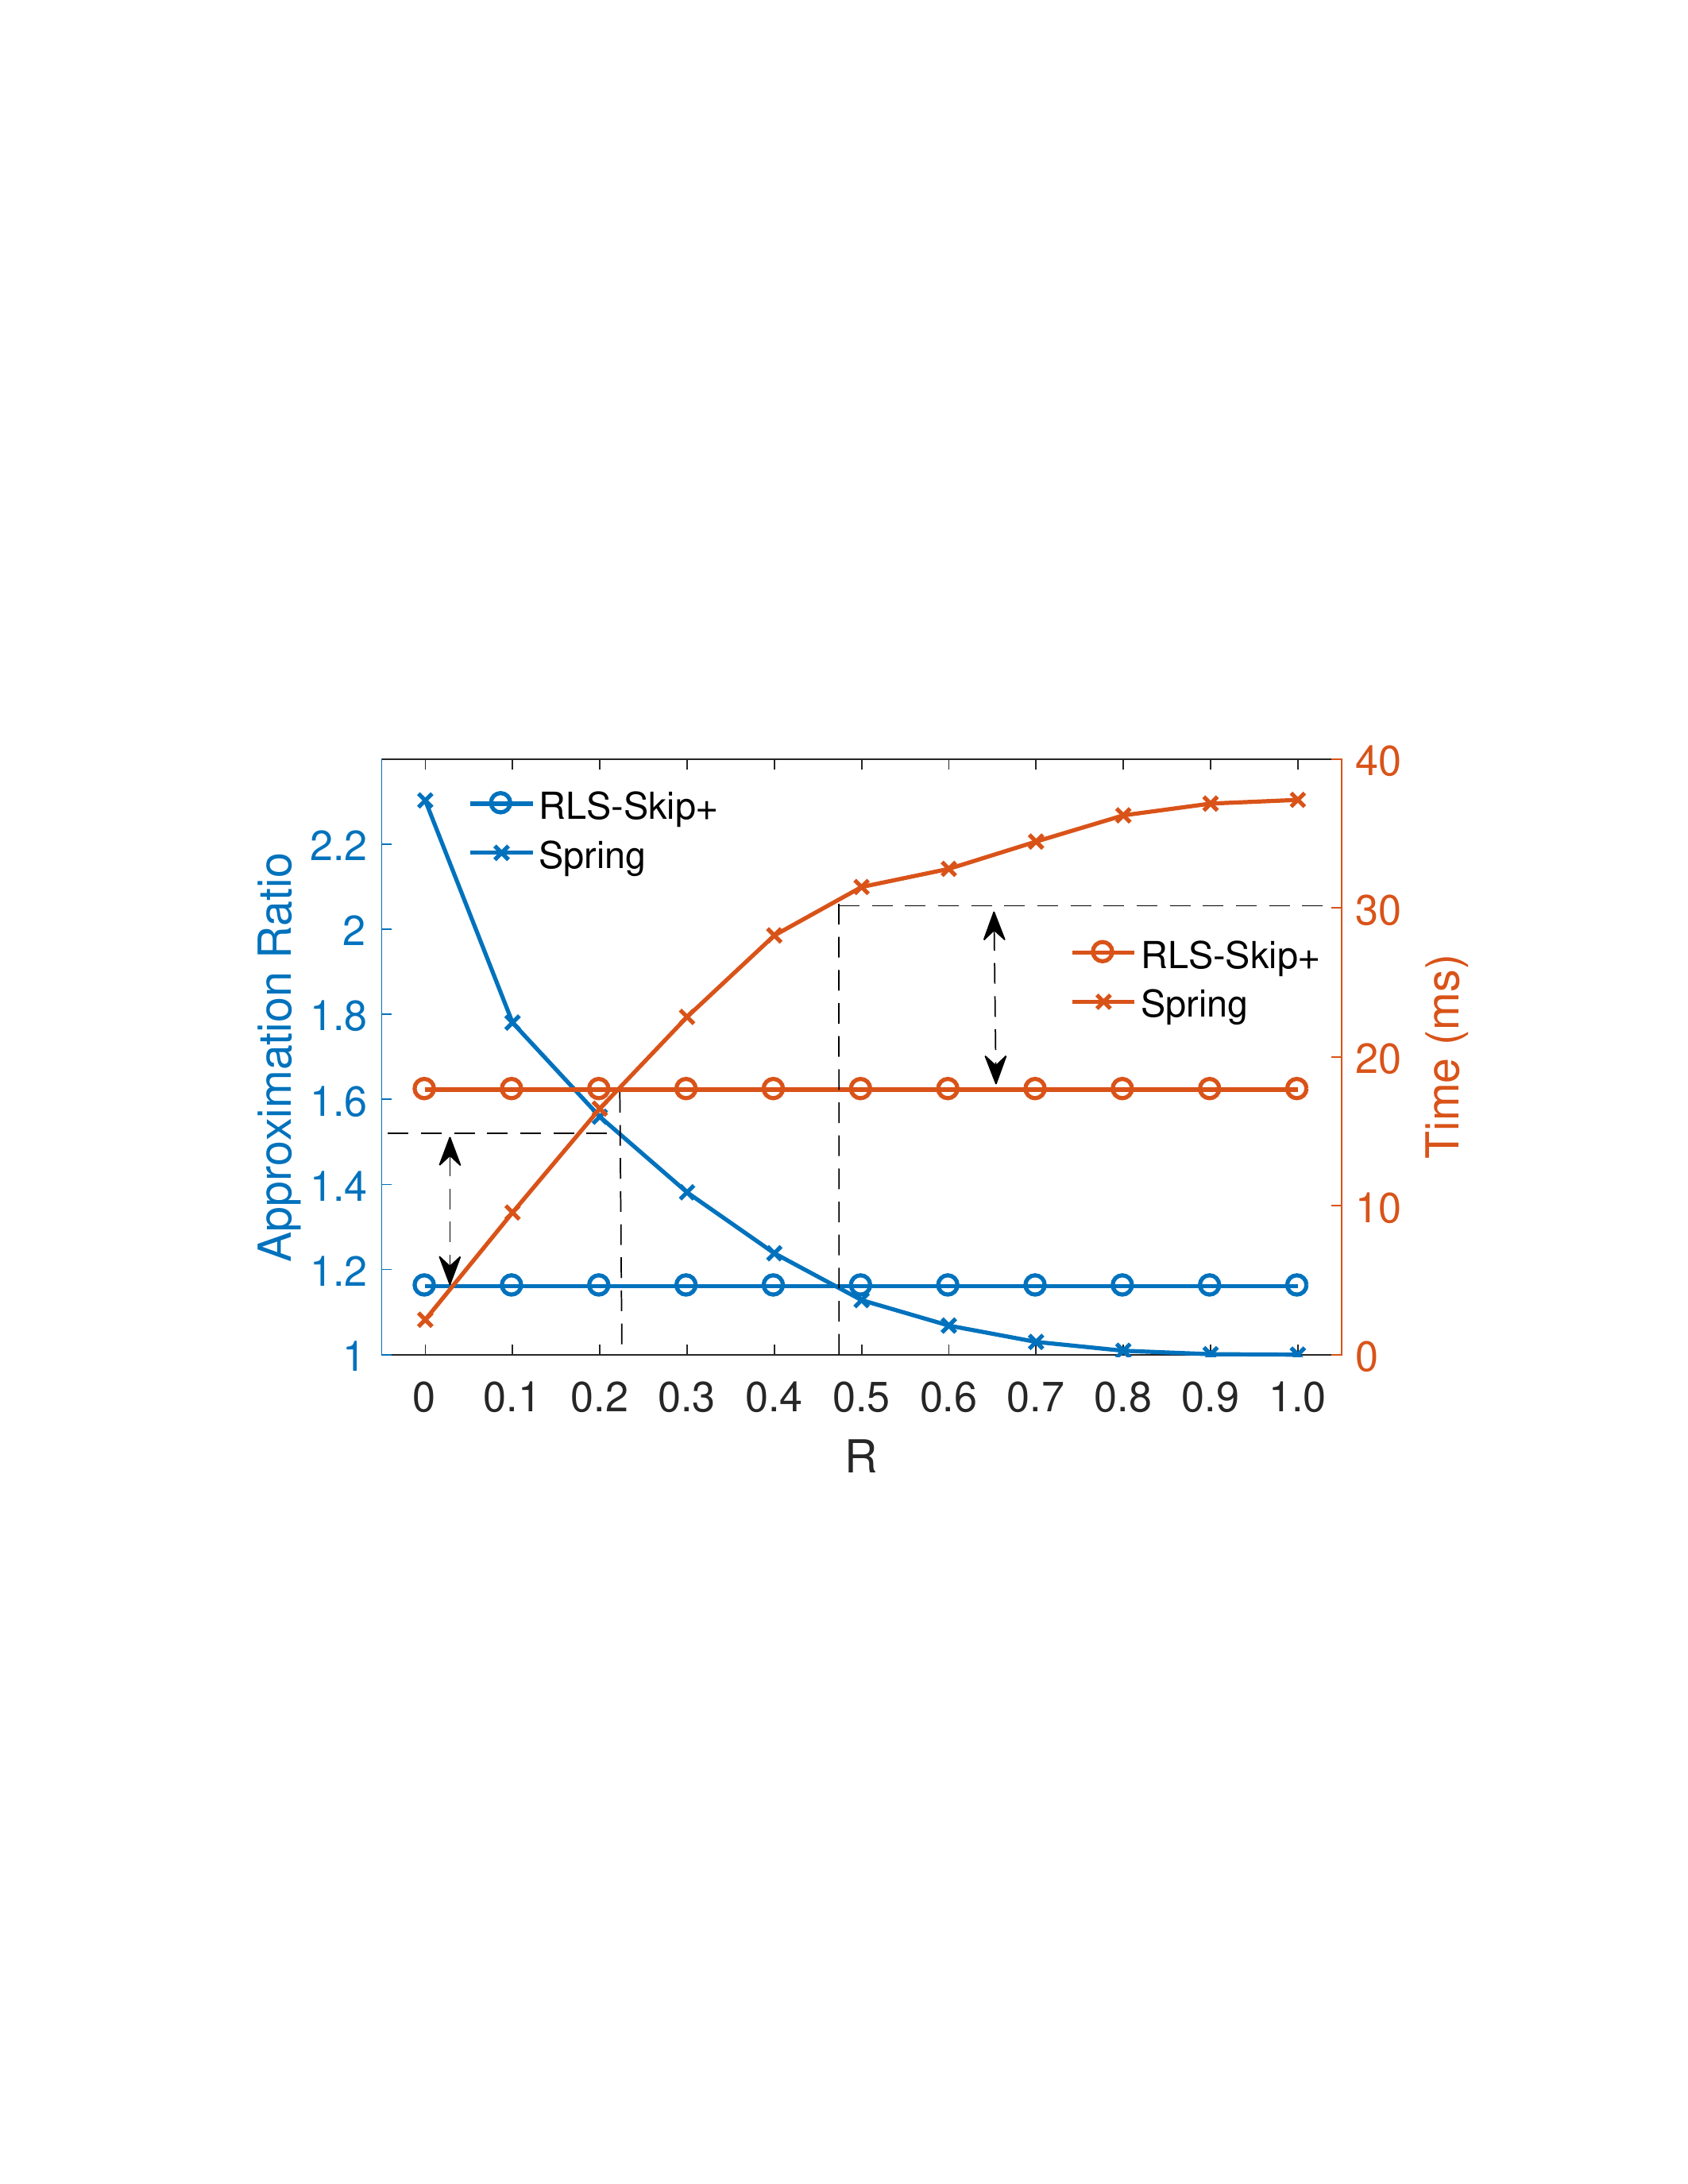}
  \end{minipage}
  &
  \begin{minipage}{4cm}%5.5
	\includegraphics[width=4.2cm]{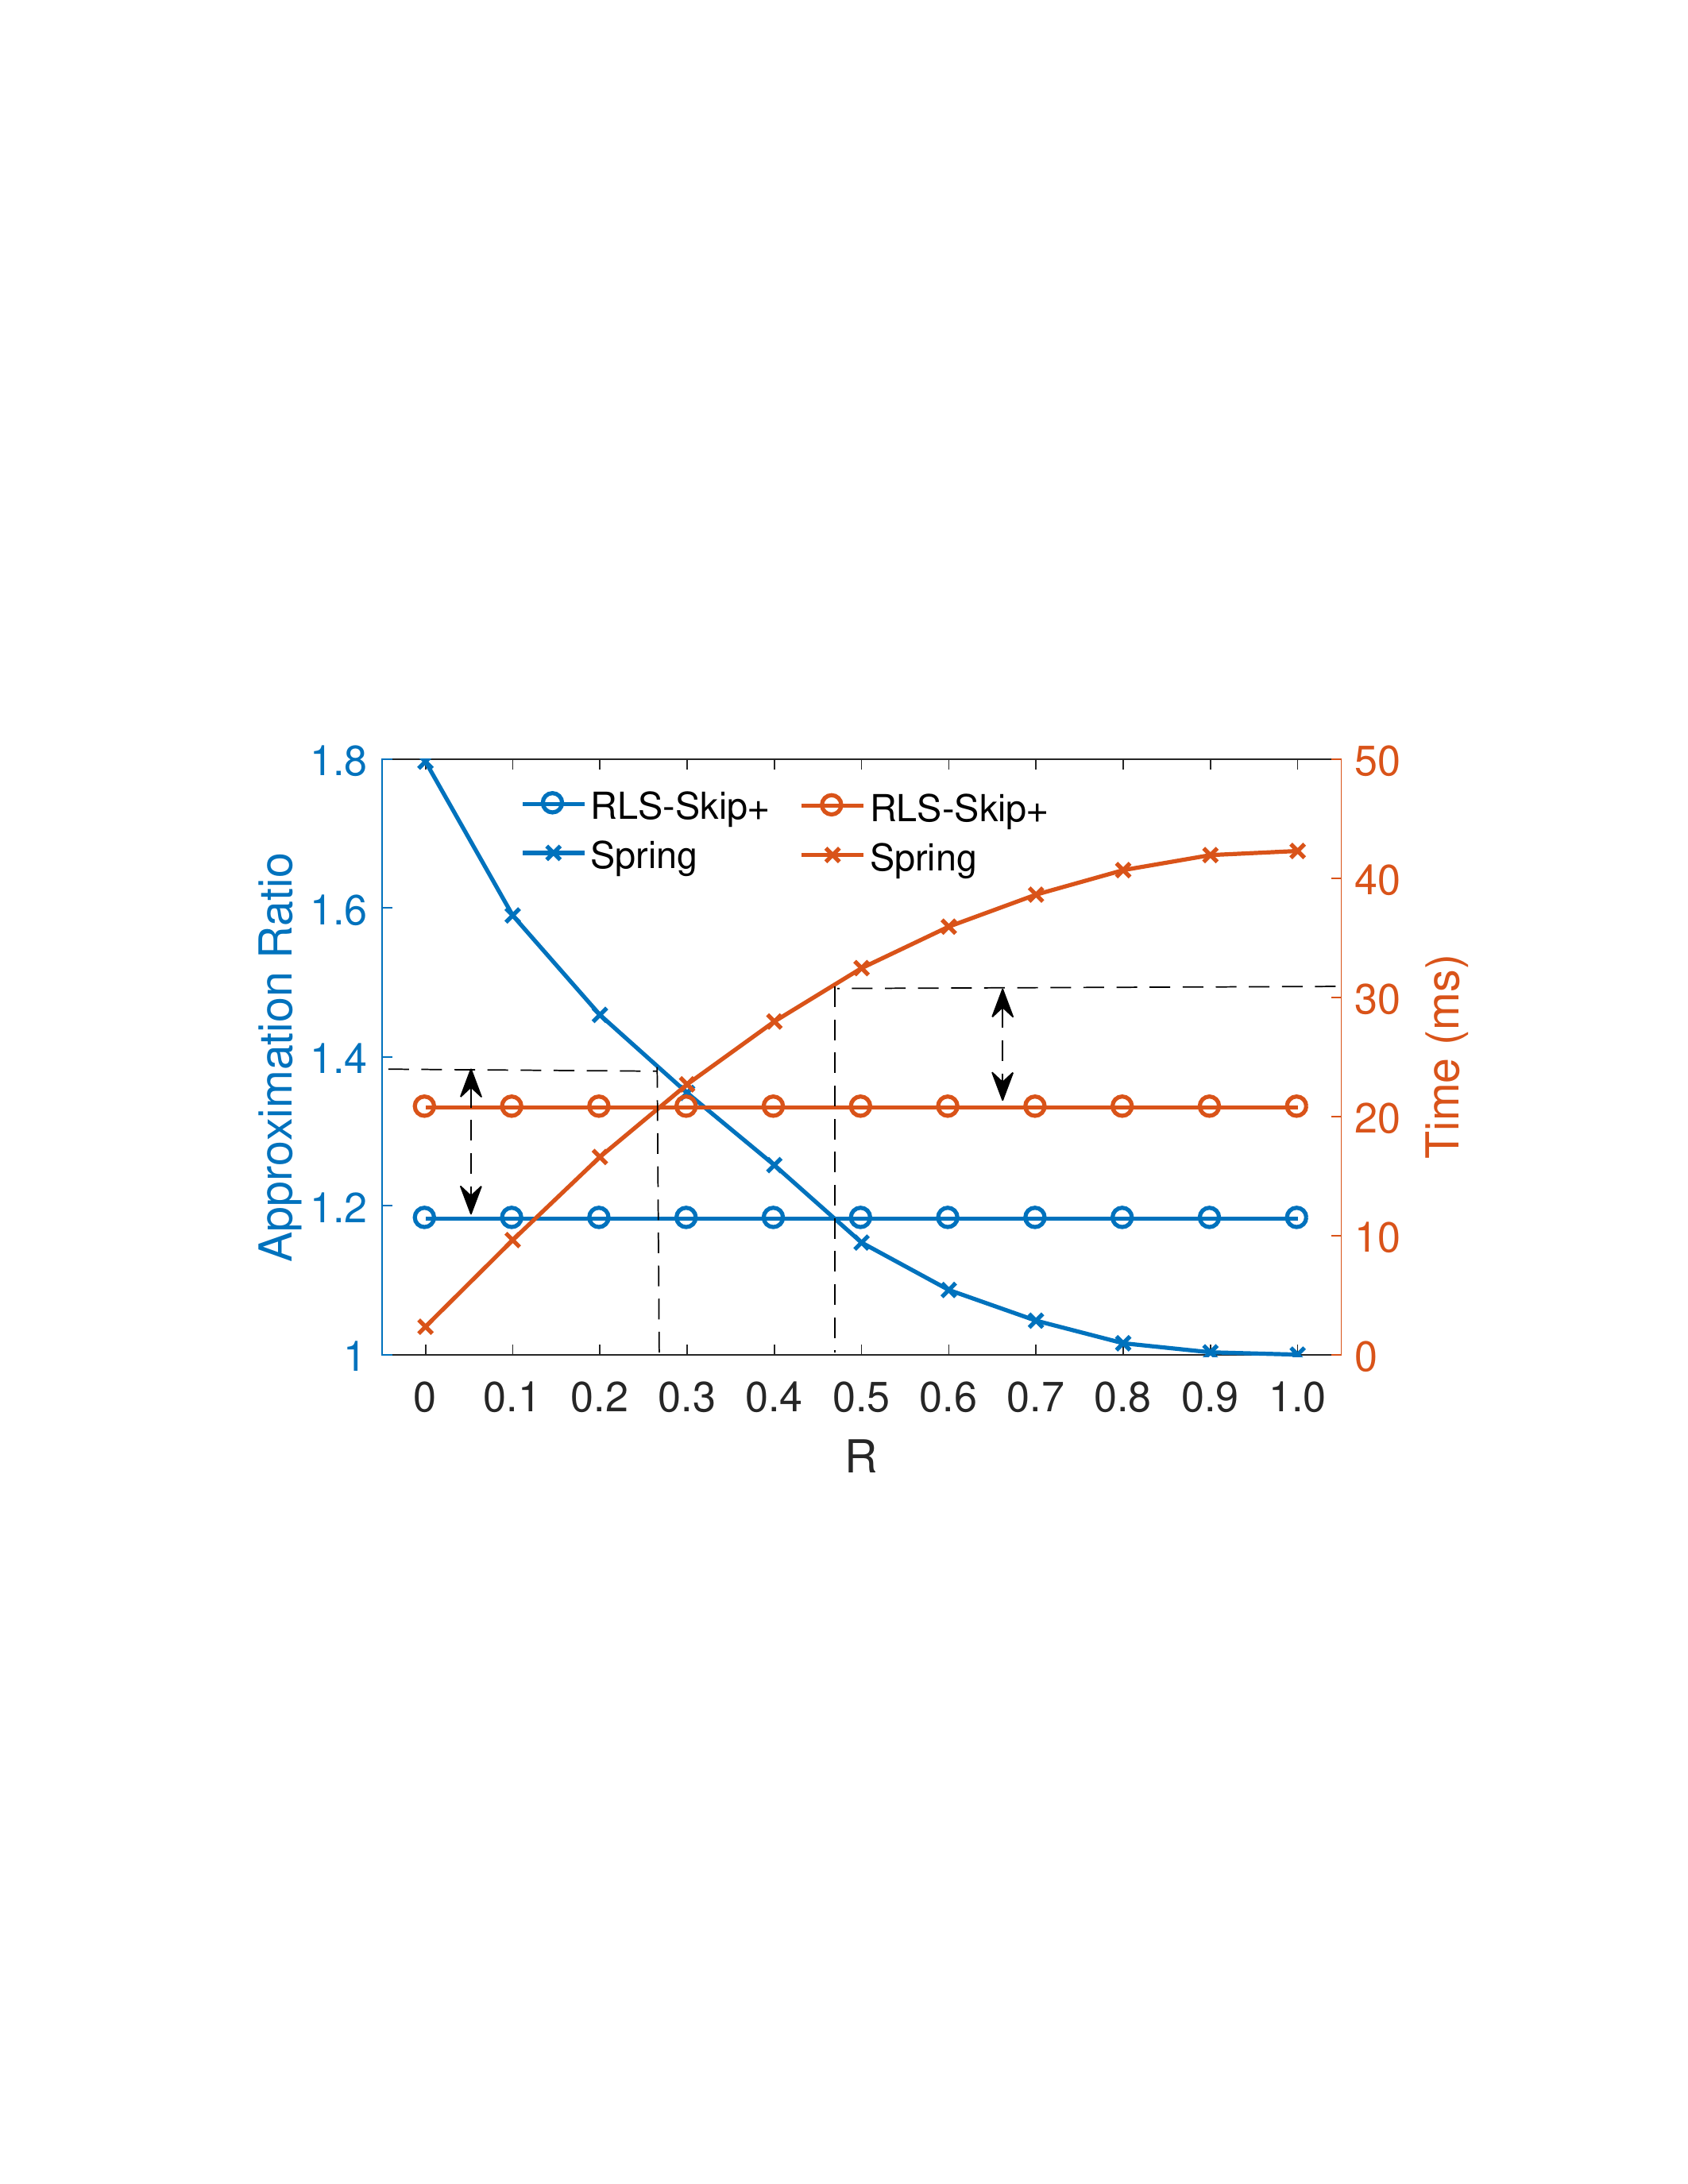}
  \end{minipage}
  \\
  \scriptsize{(c) Harbin (DTW)}
  &
  \scriptsize{(d) Harbin (Frechet)}
  \end{tabular}
\caption{Comparison with Spring method.}
\label{spring_result}
%\vspace*{-2mm}
\end{figure}
\fi
%\begin{figure}[!th]
%\centering
%\begin{tabular}{c c}
%  \begin{minipage}{4cm}%5.5
%	\includegraphics[width=4.2cm]{spring_dtw_full}
%  \end{minipage}
%  &
%  \begin{minipage}{4cm}
%	\includegraphics[width=4.2cm]{spring_fre_full}
%  \end{minipage}
%  \\
%  \scriptsize{(a) DTW}
%  &
%  \scriptsize{(b) Frechet}
%  \end{tabular}
%  %\setlength{\belowcaptionskip}{1pt}
%\caption{Comparison with Spring method.}
%\label{spring_result}
%%\vspace*{-2mm}
%\end{figure}
\if  0
We report both effectiveness and efficiency results based on varying  Sakoe-Chiba band for UCR Suite in Figure~\ref{ucr_result}. Additionally, we include two learning-based algorithms for comparison. The first one is RLS, it provides the best effectiveness among all proposed approximate algorithms. The second is called RLS-Skip+, which is another variant of learning-based algorithms by dropping suffix similarity in the state, and it provides the best efficiency. In terms of the effectiveness, we can easily observe that UCR Suite is not competitive. This is because the length of the most similar subtrajectory is various and may not has the same length as the query trajectory as we discussed the SizeS algorithm above. Regarding the efficiency, as expected, as band $R$ grows the running time increases because a big band value indicates a larger calculation cost for DTW. We can also observe the UCR Suite is much slower than RLS-Skip+ or even RLS. This is possibly because these pruning techniques may not give significant benefits for trajectory data, and the computation of lower bounds will spend some extra time if a pruning cannot work for a DTW calculation.
\fi

\if 0
\smallskip\noindent\textbf{Adaption of Spring.}
Spring~\cite{sakurai2007stream} corresponds to the dynamic programming process for computing the DTW distance between the data time series and the query time series, where the latter is padded with a fictitious point that could be aligned with any point of the data time series with distance equal to 0.
When the DTW distance is used, the Spring algorithm could be directly used for our ``similar subtrajectory search'' problem. We refer to~\cite{sakurai2007stream} for the details of this algorithm.
When the Frechet distance is used, the Spring algorithm could be adapted by simply changing the dynamic programming equation from that of DTW (Equation~(\ref{dtw_sm})) to that of Frechet (Equation~(\ref{fre_sm})).
We note that Spring algorithm cannot be used or adapted for the t2vec distance since t2vec is not based on a dynamic programming process as DTW or Frechet.
\fi
\if 0
Besides, we compare with another baseline called Spring~\cite{sakurai2007stream}, which is specifically designed for exact subsequence search based on DTW or Frechet distance. We vary the Sakoe-Chiba band for the distance computation and report the effectiveness and efficiency results in Figure~\ref{spring_result}. As expected, as the band grows the effectiveness of Spring becomes
better and approaches the exact results while its running time increases. We label two intersections in these figures for ease of reference. For example, in Figure~\ref{spring_result}(a), RLS-Skip+ and Spring achieve the same efficiency at $R$ around 0.2, but our effectiveness is better. Similarly, when both of them achieve the same effectiveness at $R$ around 0.4, RLS-Skip+ is faster, and the speedups can up to around 2.5 times. On the other hand, to our best knowledge, the technique of Spring cannot generalize to other similarity measurements such as t2vec; however, our method is generic enough to support any of these existing measurements. Thus, it can be widely used for more trajectory tasks.
\fi

\section{Additional Experimental Results}
\begin{figure*}[!t]
	\hspace*{-.5cm}
	\centering
	\begin{tabular}{c c c c c c}
		\begin{minipage}{2.6cm}
			\includegraphics[width=2.85cm]{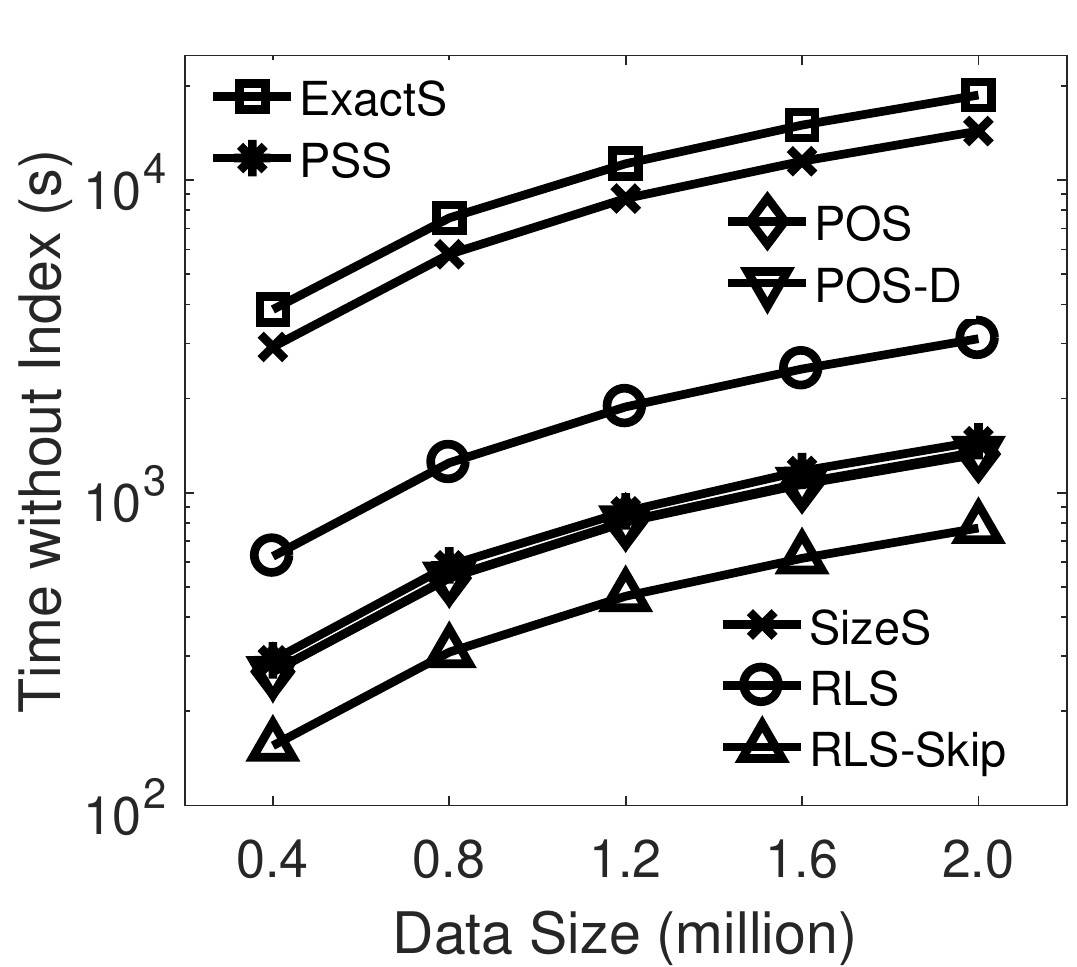}
		\end{minipage}
		&
		\begin{minipage}{2.6cm}
			\includegraphics[width=2.85cm]{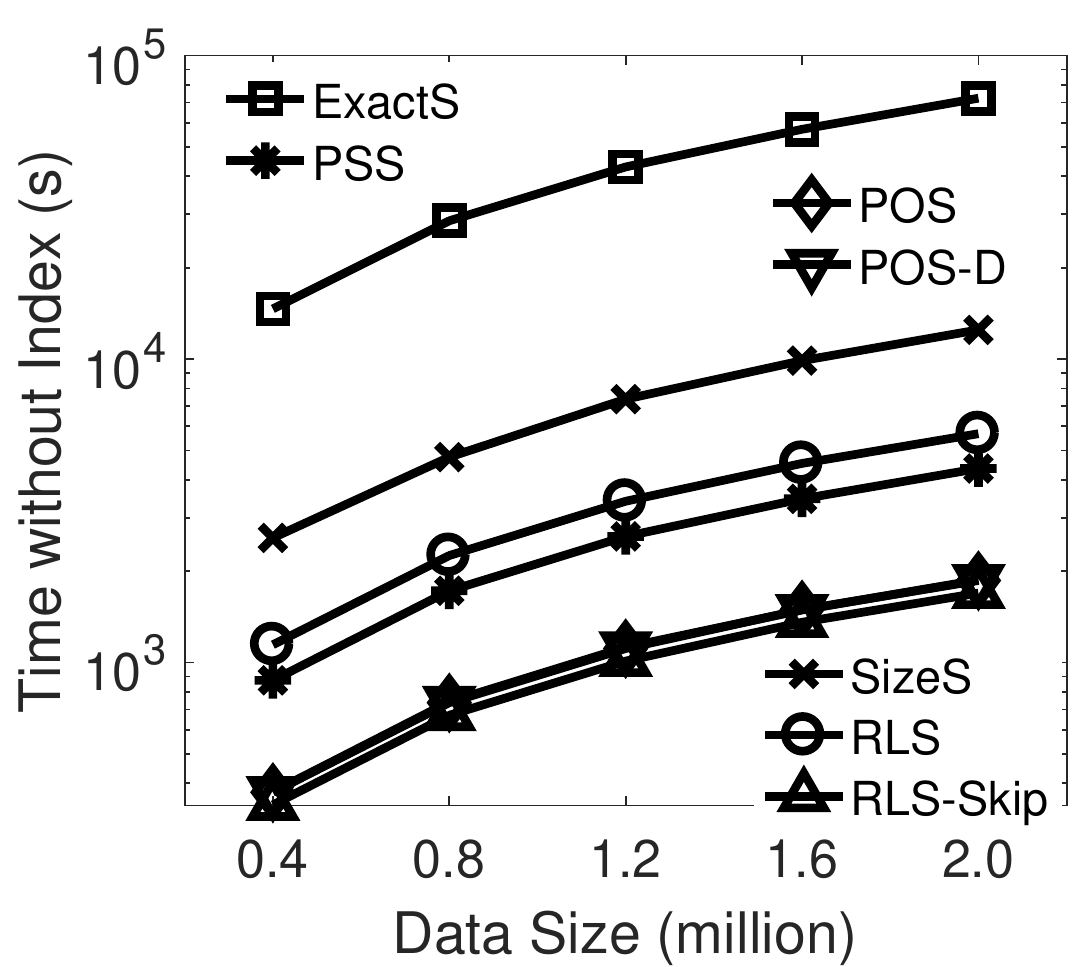}
		\end{minipage}
		&
		\begin{minipage}{2.6cm}
			\includegraphics[width=2.85cm]{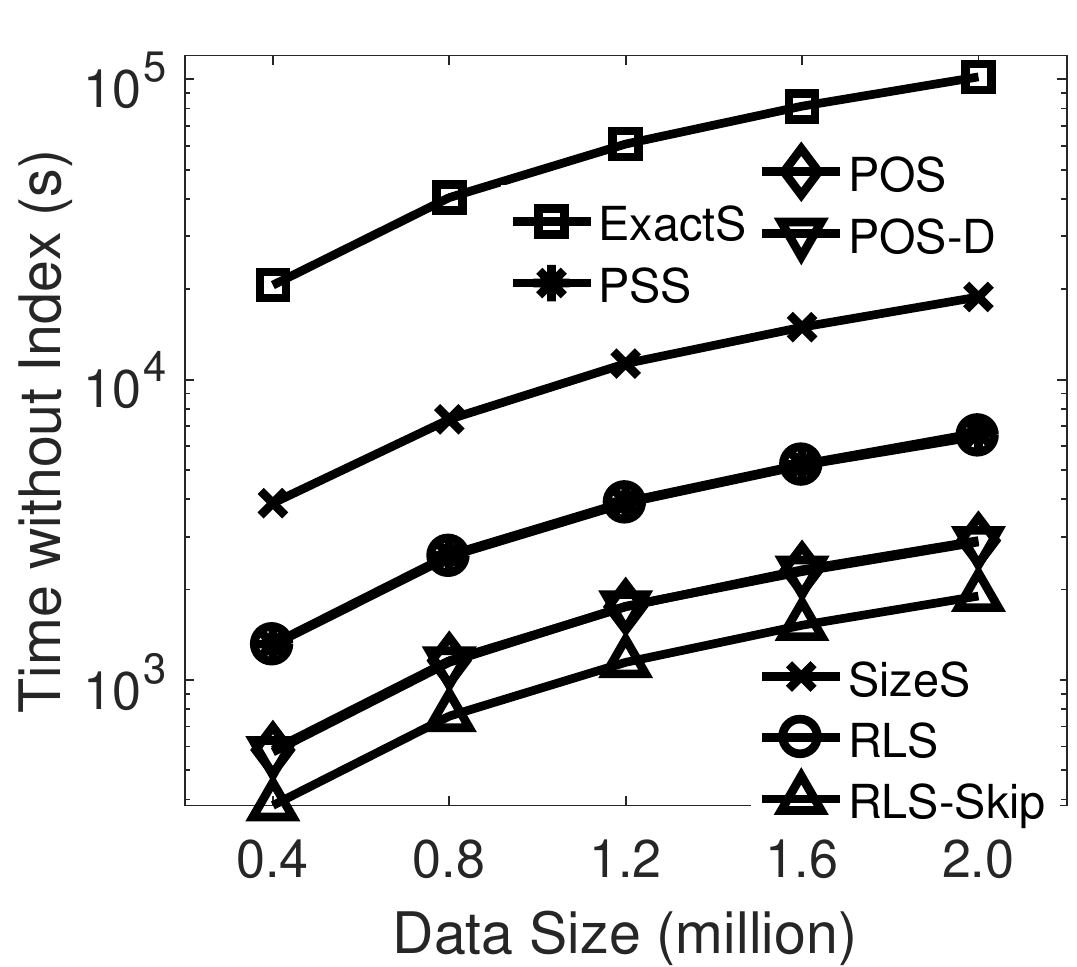}
		\end{minipage}
        &
        \begin{minipage}{2.6cm}
			\includegraphics[width=2.85cm]{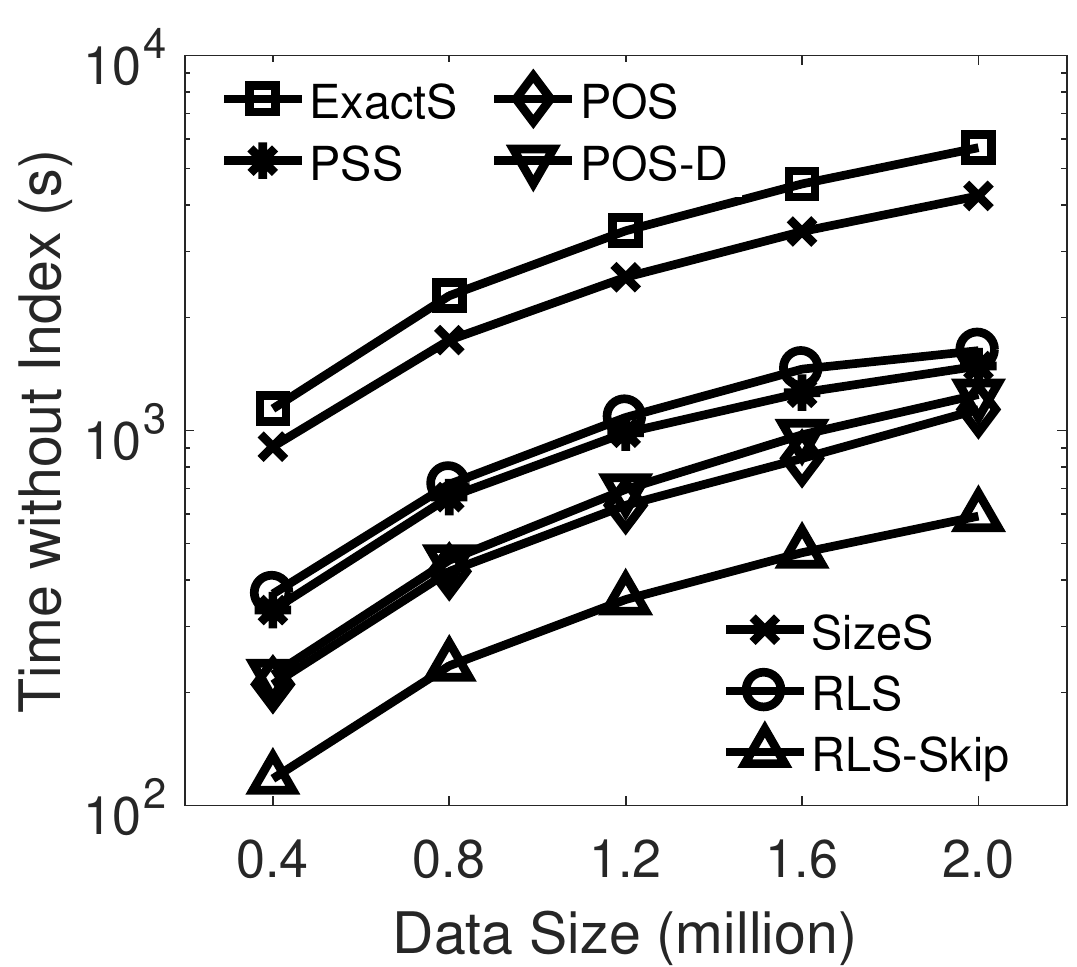}
		\end{minipage}
		&
		\begin{minipage}{2.6cm}
			\includegraphics[width=2.85cm]{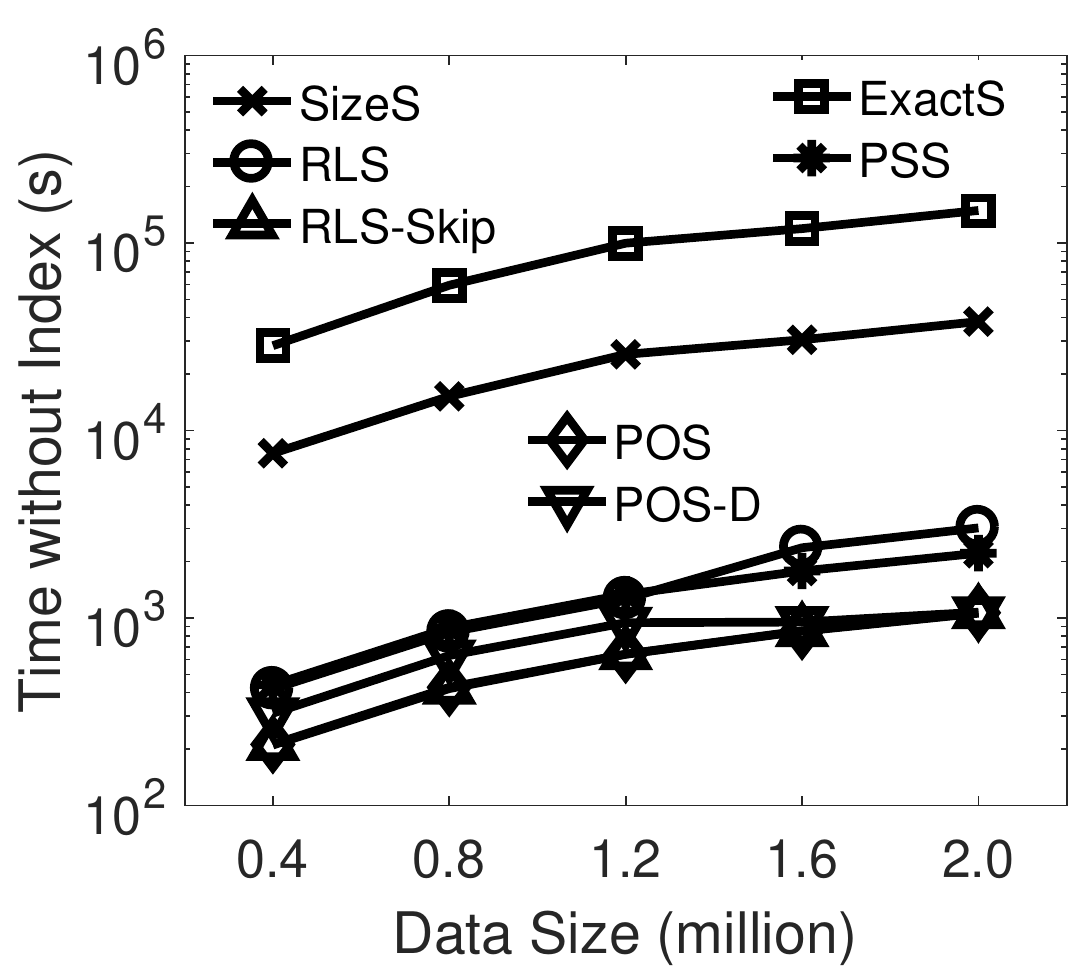}
		\end{minipage}
		&
		\begin{minipage}{2.6cm}
			\includegraphics[width=2.85cm]{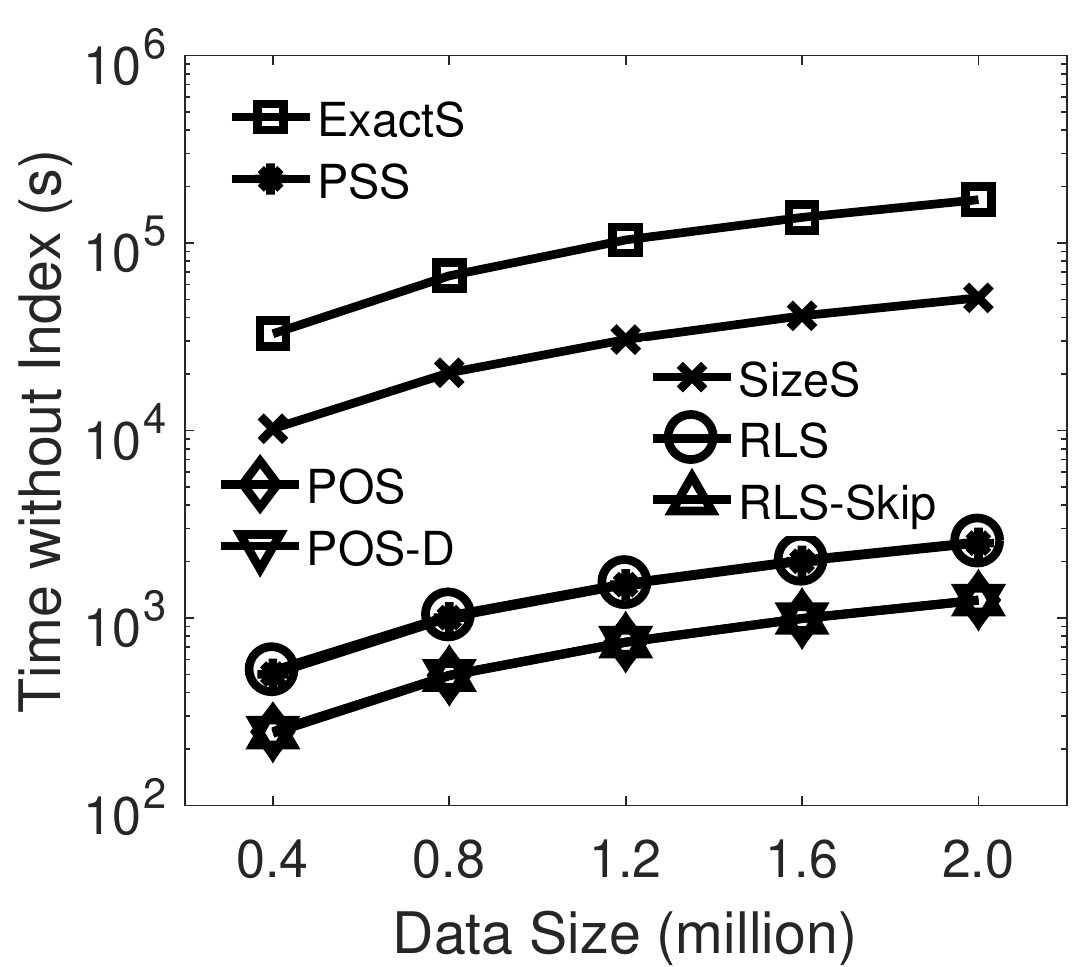}
		\end{minipage}
		\\
		\scriptsize (a) Harbin (t2vec)
        &
		\scriptsize (b) Harbin (DTW)
		&
		\scriptsize (c) Harbin (Frechet)
        &
		\scriptsize (d) Sports (t2vec)
        &
		\scriptsize (e) Sports (DTW)
		&
		\scriptsize (f) Sports (Frechet)
		\\
		\begin{minipage}{2.6cm}
			\includegraphics[width=2.85cm]{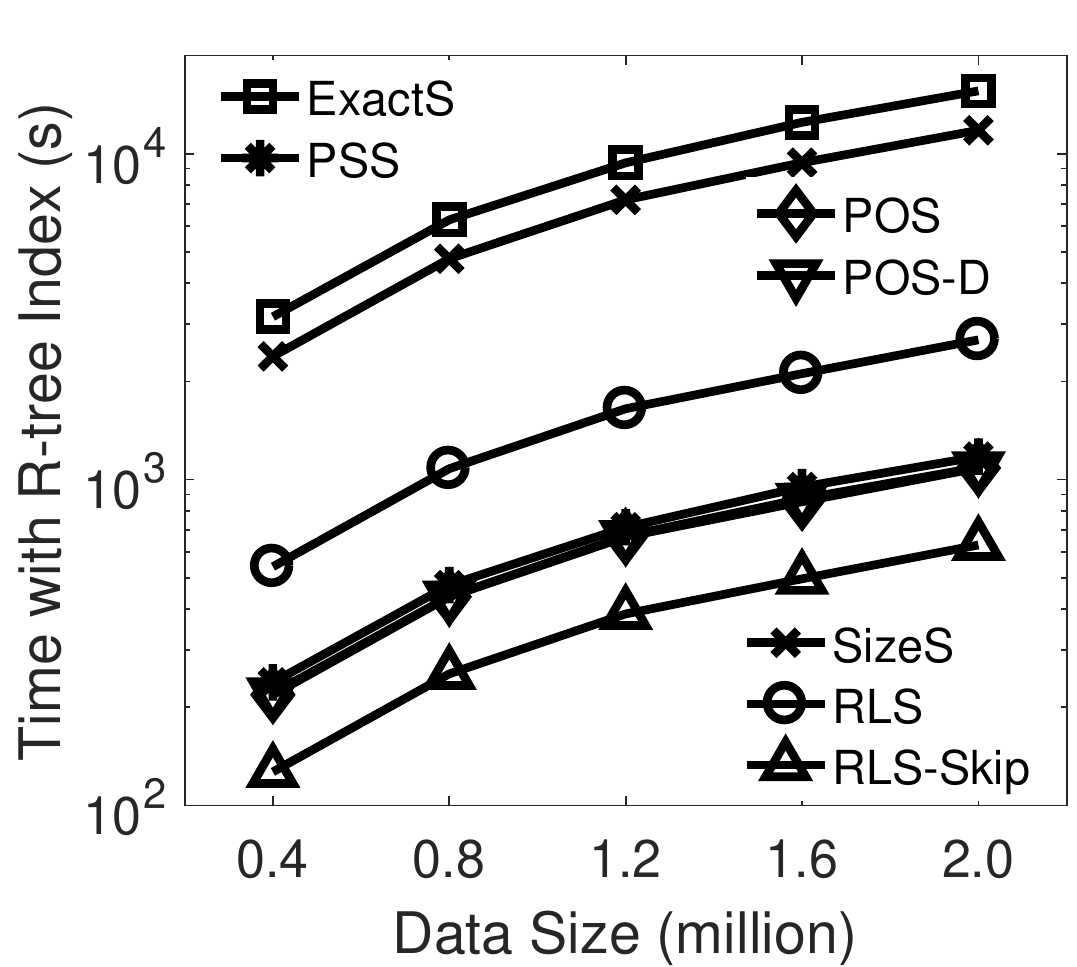}
		\end{minipage}
		&
		\begin{minipage}{2.6cm}
			\includegraphics[width=2.85cm]{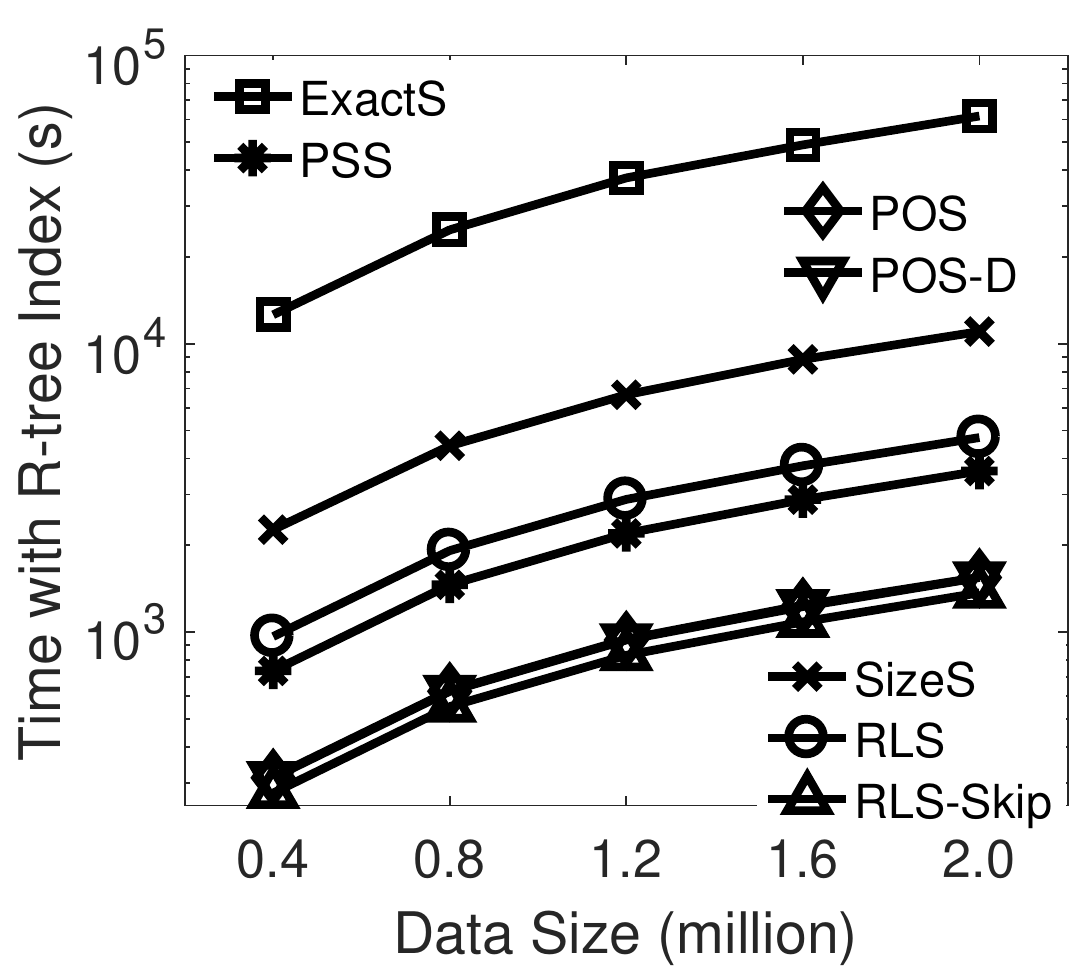}
		\end{minipage}
		&
		\begin{minipage}{2.6cm}
			\includegraphics[width=2.85cm]{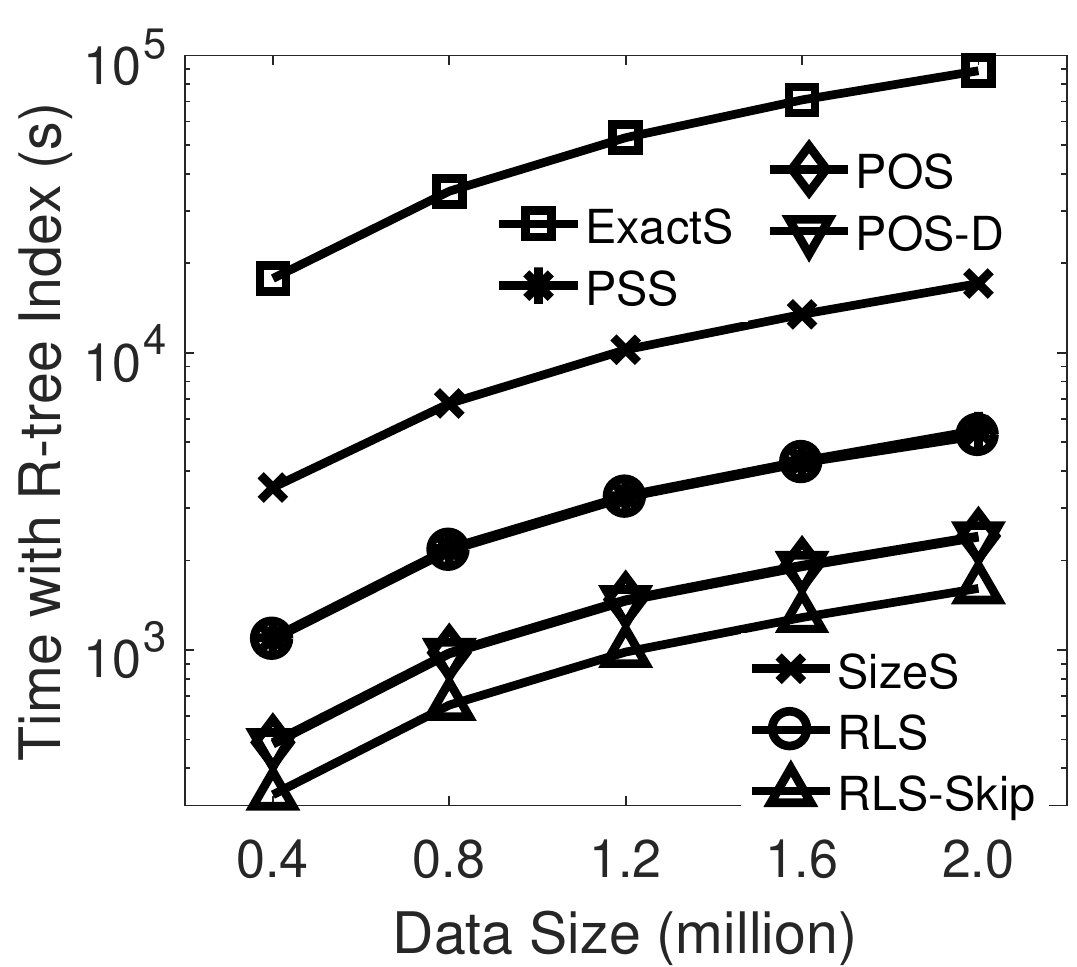}
		\end{minipage}
        &
        \begin{minipage}{2.6cm}
			\includegraphics[width=2.85cm]{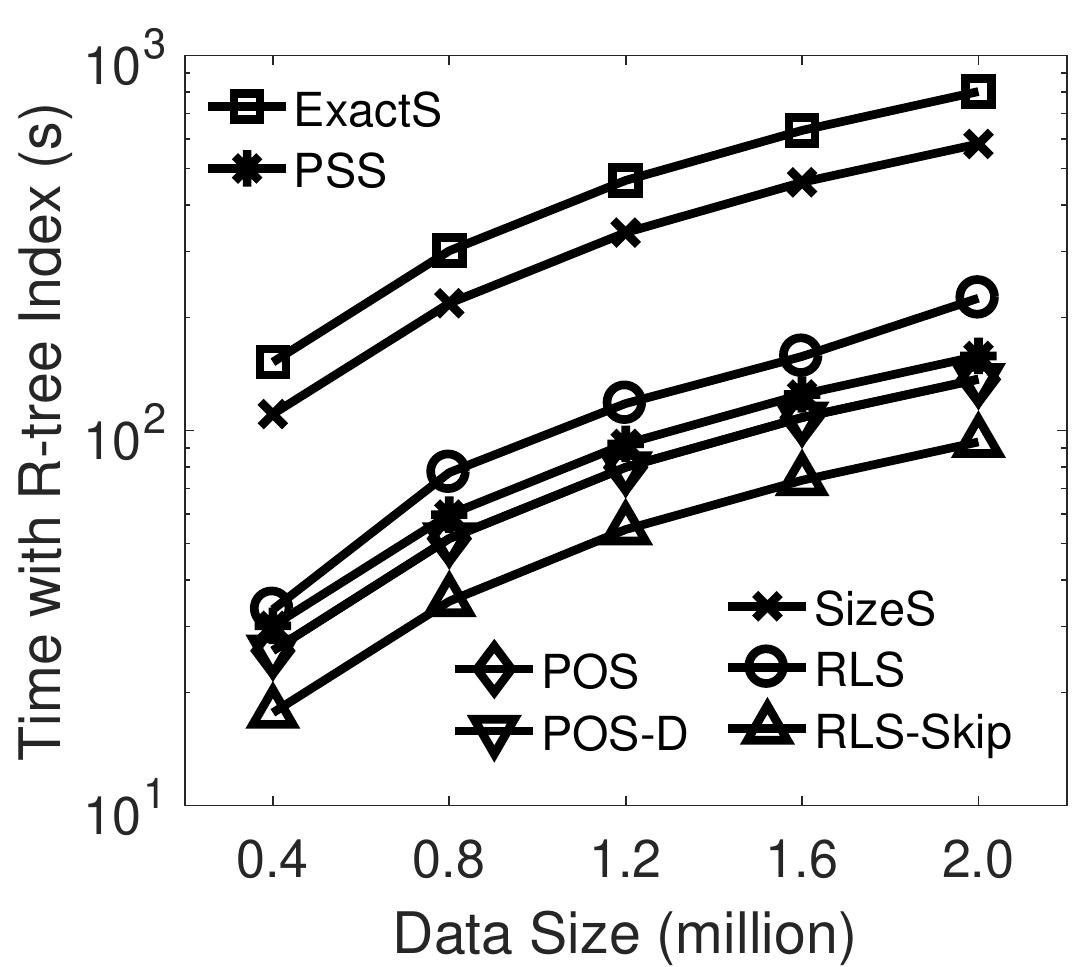}
		\end{minipage}
		&
		\begin{minipage}{2.6cm}
			\includegraphics[width=2.85cm]{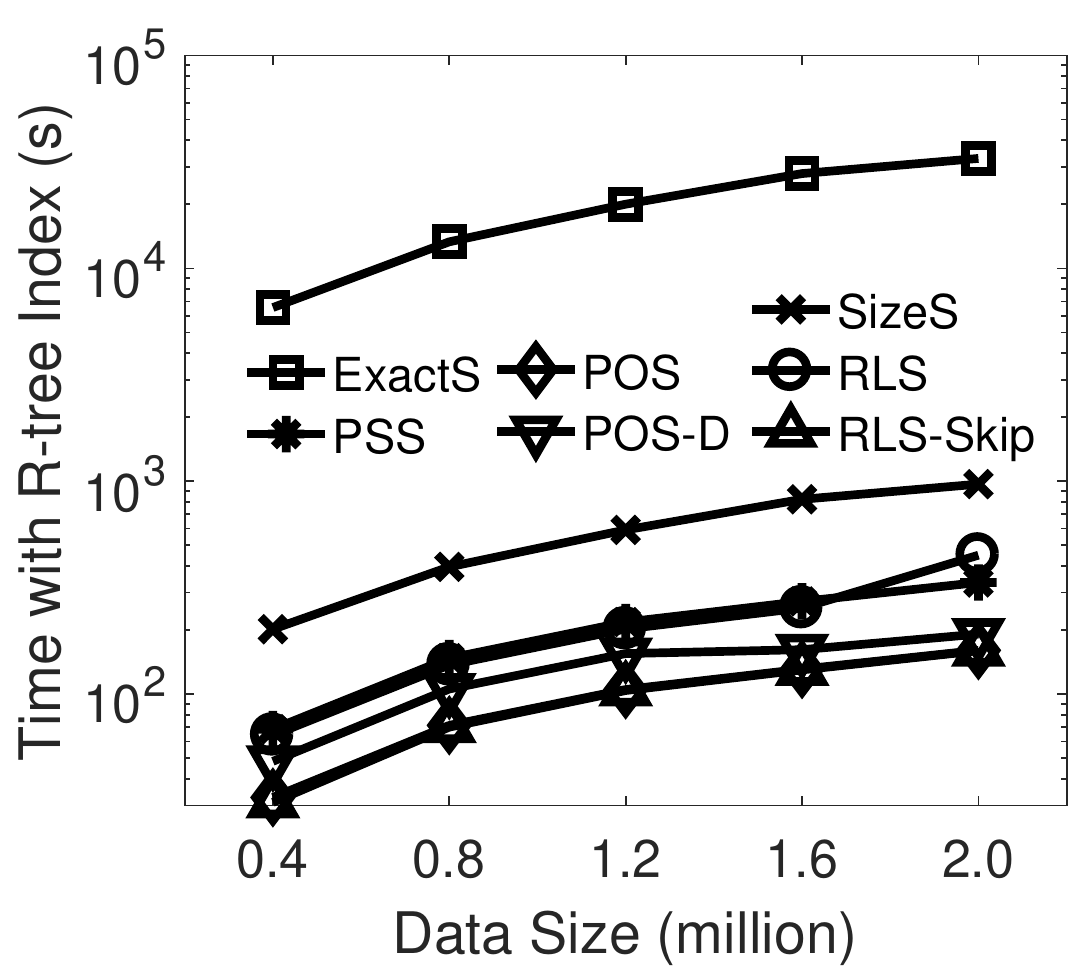}
		\end{minipage}
		&
		\begin{minipage}{2.6cm}
			\includegraphics[width=2.85cm]{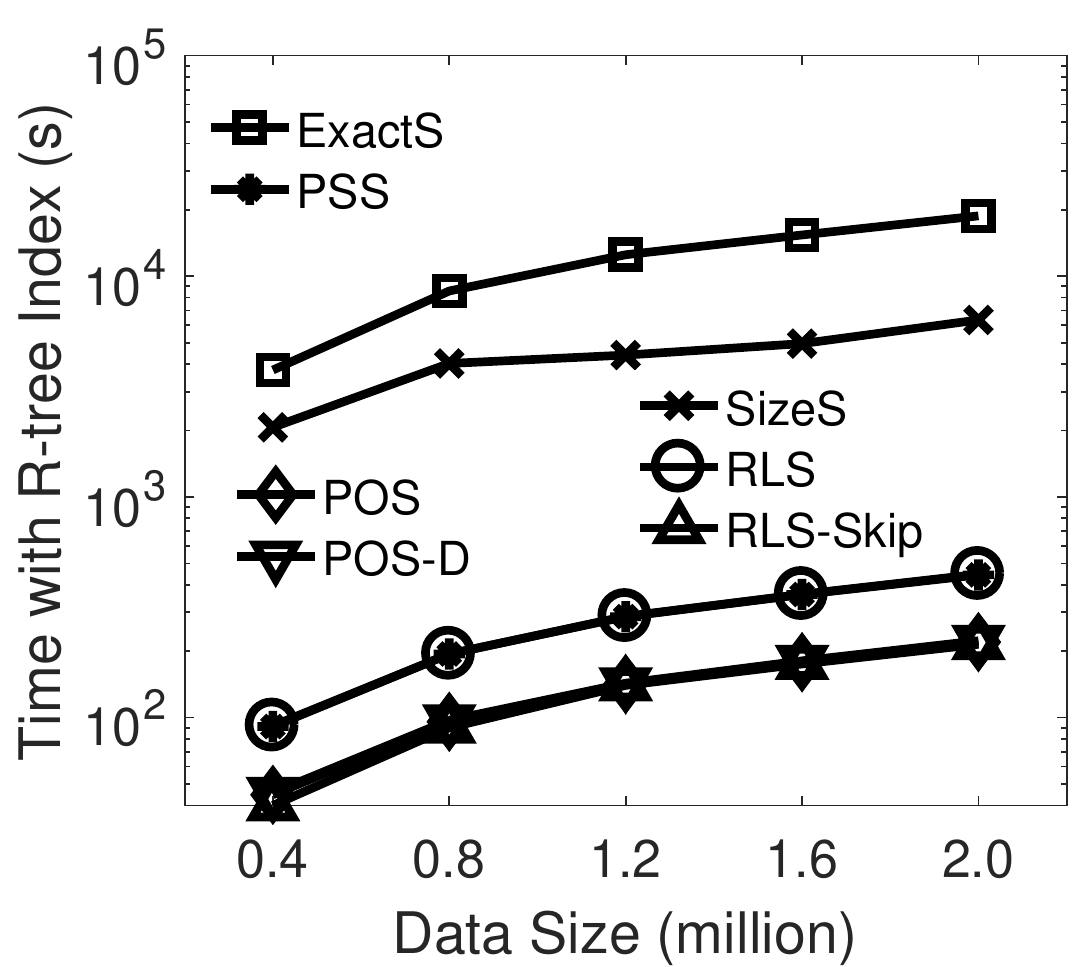}
		\end{minipage}
		\\
		\scriptsize (g) Harbin (t2vec)
		&
		\scriptsize (h) Harbin (DTW)
		&
		\scriptsize (i) Harbin (Frechet)
        &
		\scriptsize (j) Sports (t2vec)
		&
		\scriptsize (k) Sports (DTW)
		&
		\scriptsize (l) Sports (Frechet)

	\end{tabular}
	%\vspace{-4mm}
	\caption{Efficiency without index (a)-(f) and with R-tree index (g)-(l) on Harbin and Sports.}
	\label{fig:efficiencyRLS_hs}
	%\vspace{-4mm}
\end{figure*}
\begin{figure*}[!ht]
	\hspace*{-.5cm}
	\centering
	\begin{tabular}{c c c c c c}
		\begin{minipage}{2.6cm}
			\includegraphics[width=2.85cm]{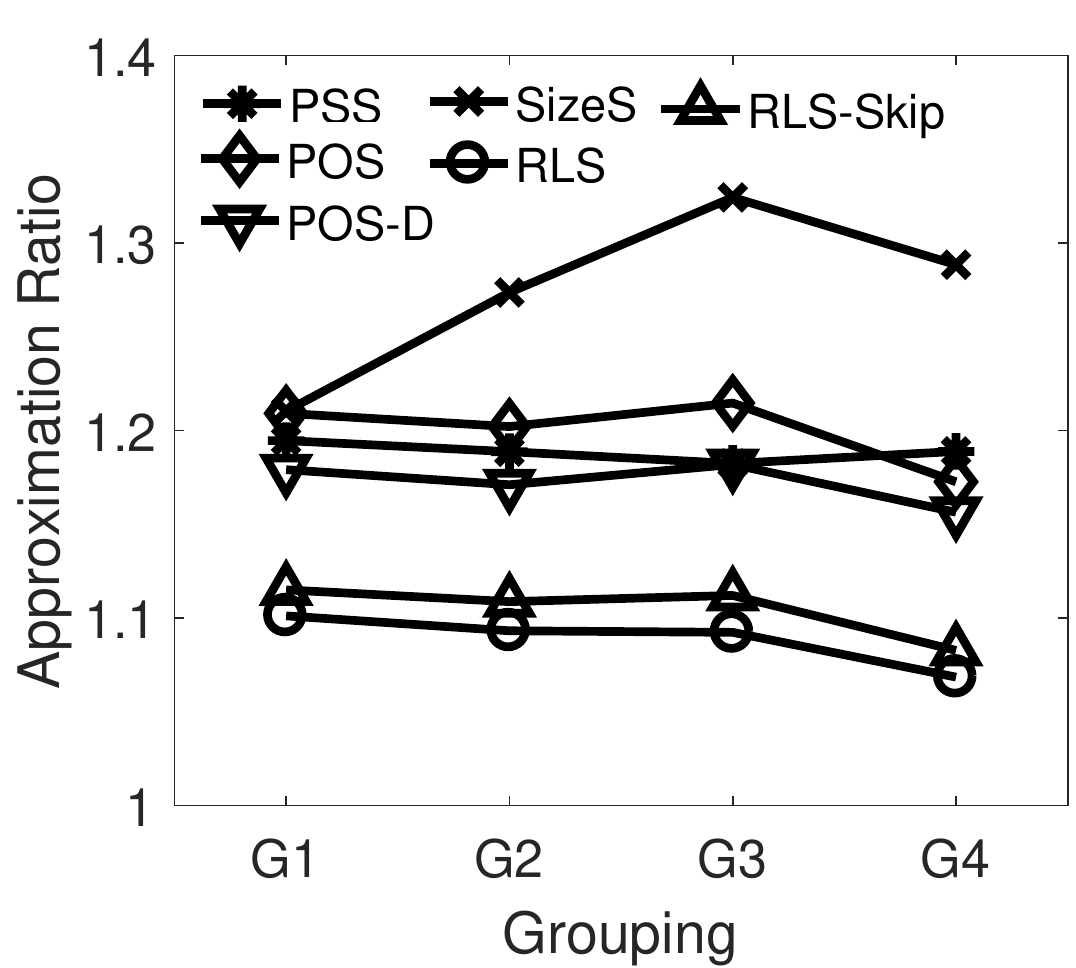}
		\end{minipage}
		&
		\begin{minipage}{2.6cm}
			\includegraphics[width=2.85cm]{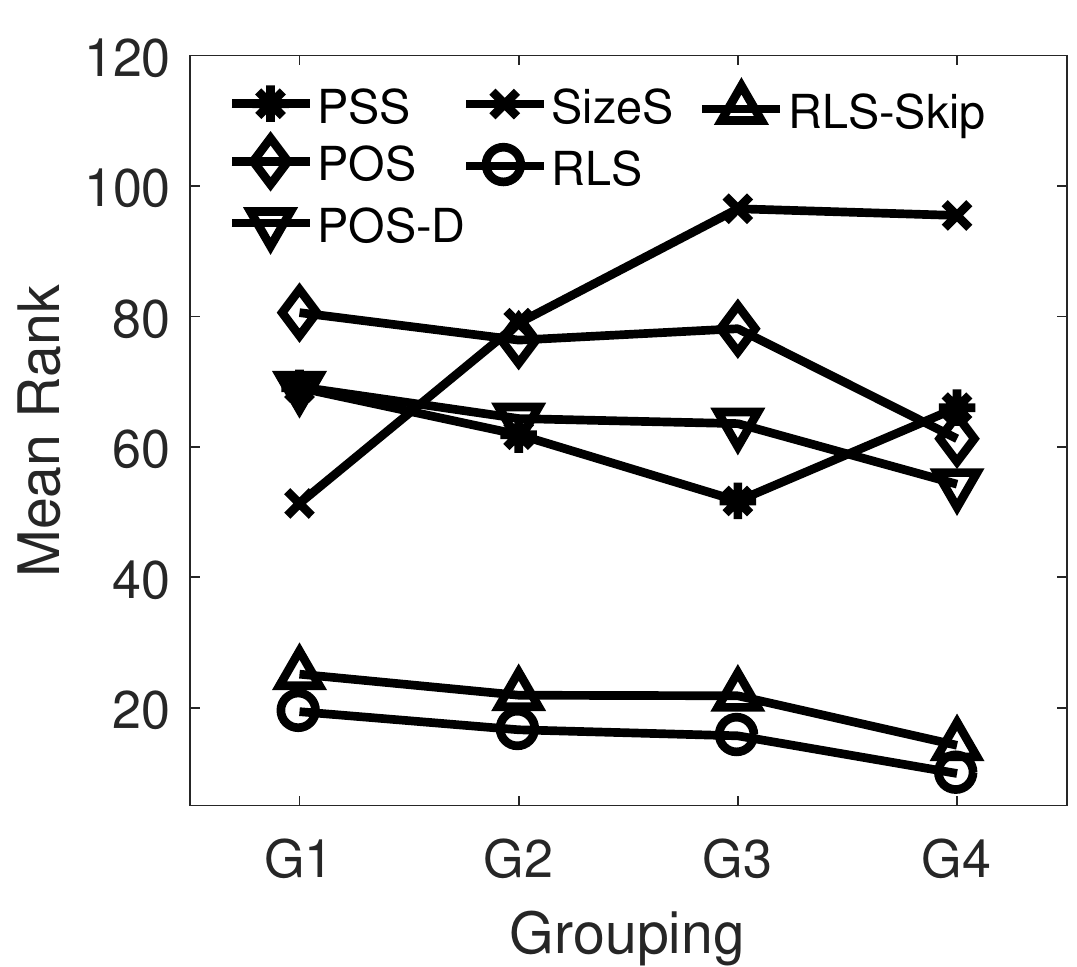}
		\end{minipage}
		&
		\begin{minipage}{2.6cm}
			\includegraphics[width=2.85cm]{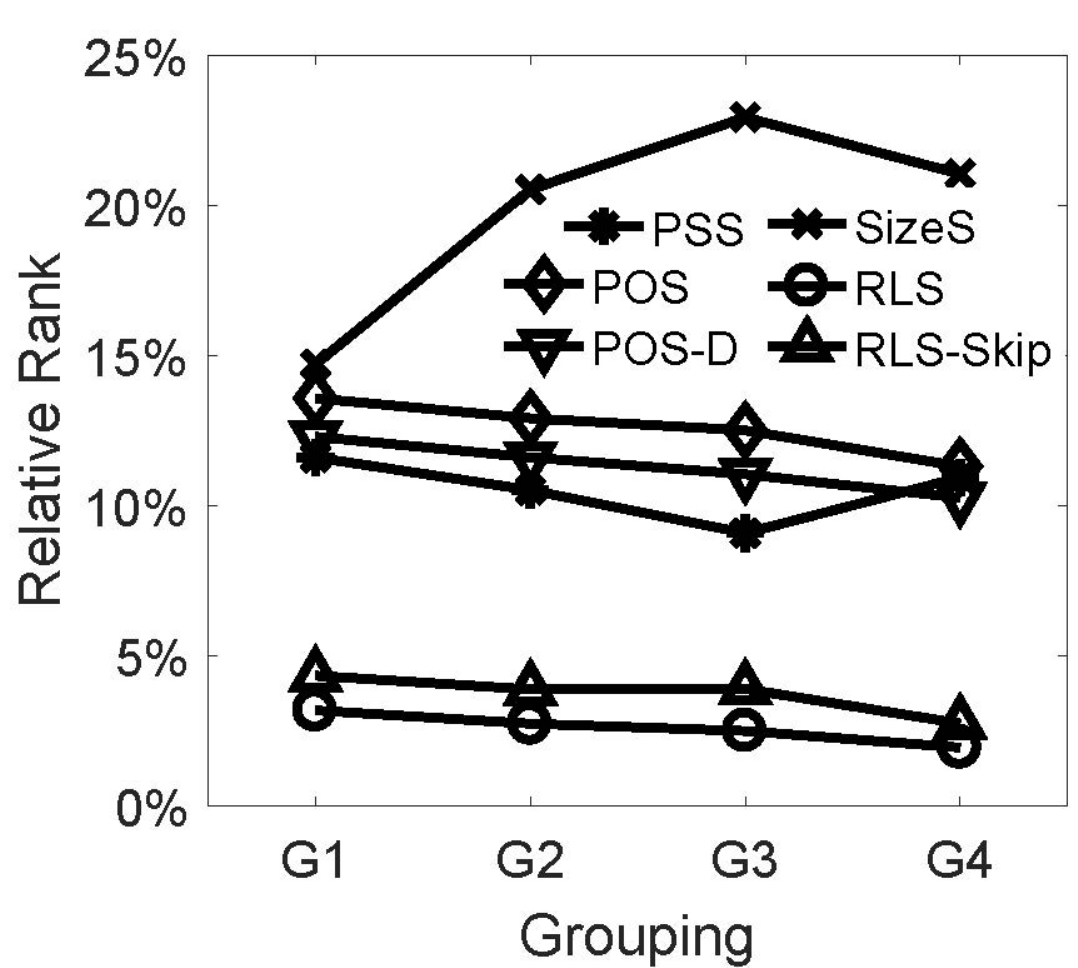}
		\end{minipage}
		&
		\begin{minipage}{2.6cm}
			\includegraphics[width=2.85cm]{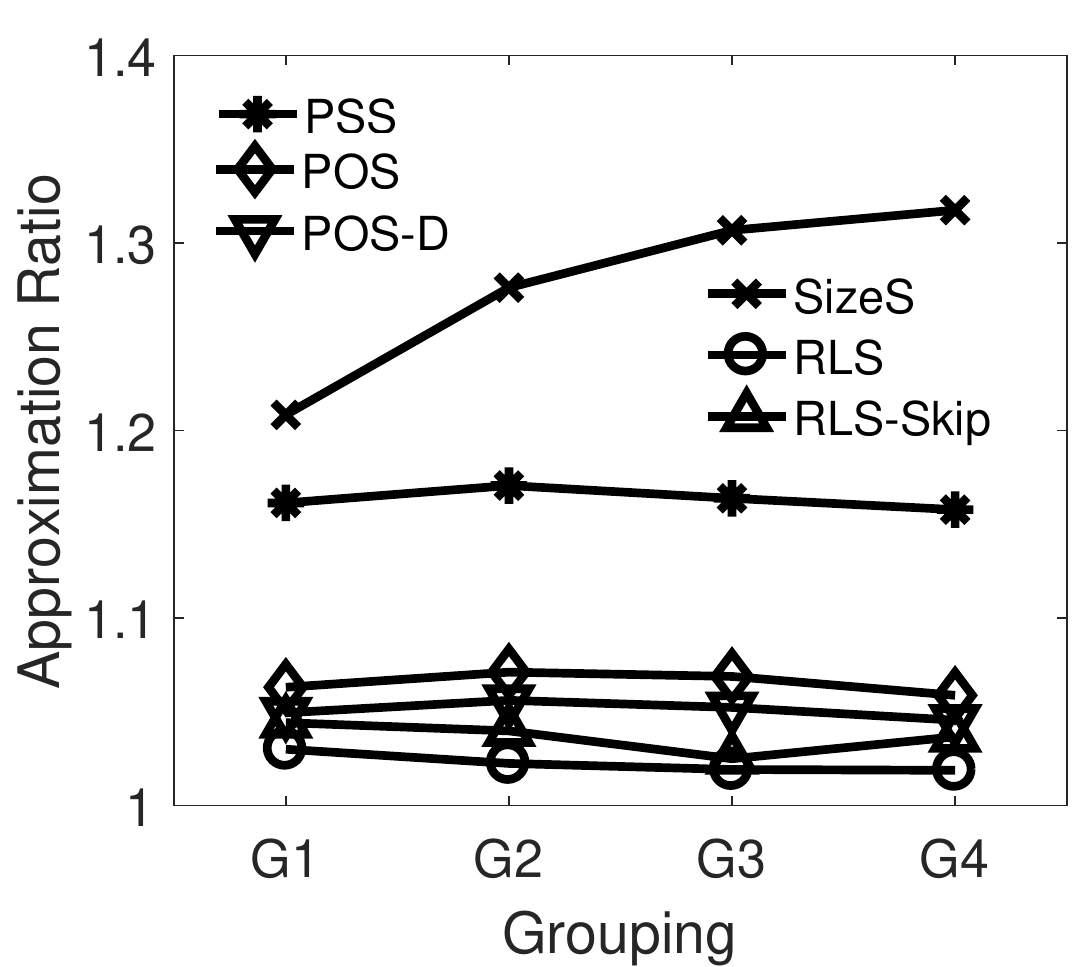}
		\end{minipage}
		&
		\begin{minipage}{2.6cm}
			\includegraphics[width=2.85cm]{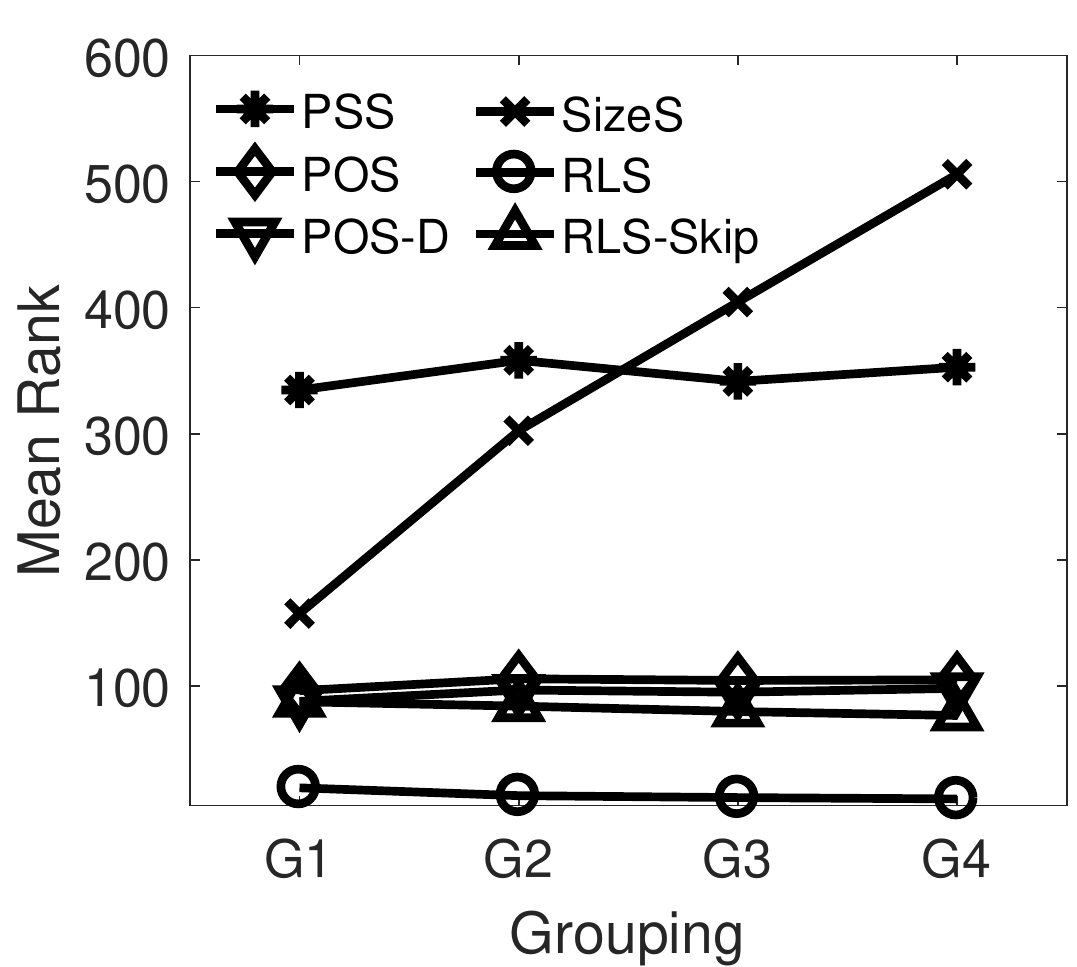}
		\end{minipage}
		&
		\begin{minipage}{2.6cm}
			\includegraphics[width=2.85cm]{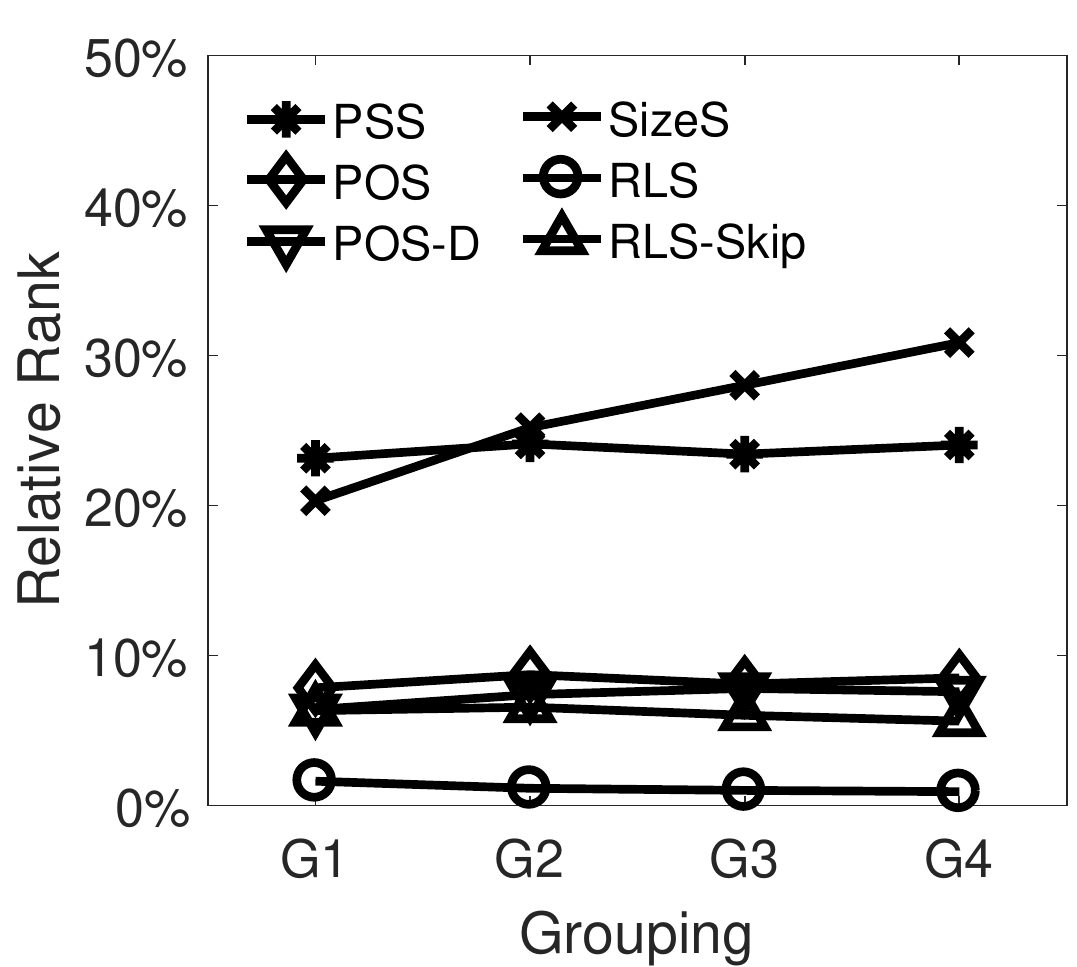}
		\end{minipage}
		\\
		\scriptsize (a) AR Porto% (t2vec)
		&
		\scriptsize (b) MR Porto% (t2vec)
		&
		\scriptsize (c) RR Porto% (t2vec)
		&
		\scriptsize (d) AR Harbin% (t2vec)
		&
		\scriptsize (e) MR Harbin% (t2vec)
		&
		\scriptsize (f) RR Harbin% (t2vec)
		\\
		
		\begin{minipage}{2.6cm}
			\includegraphics[width=2.85cm]{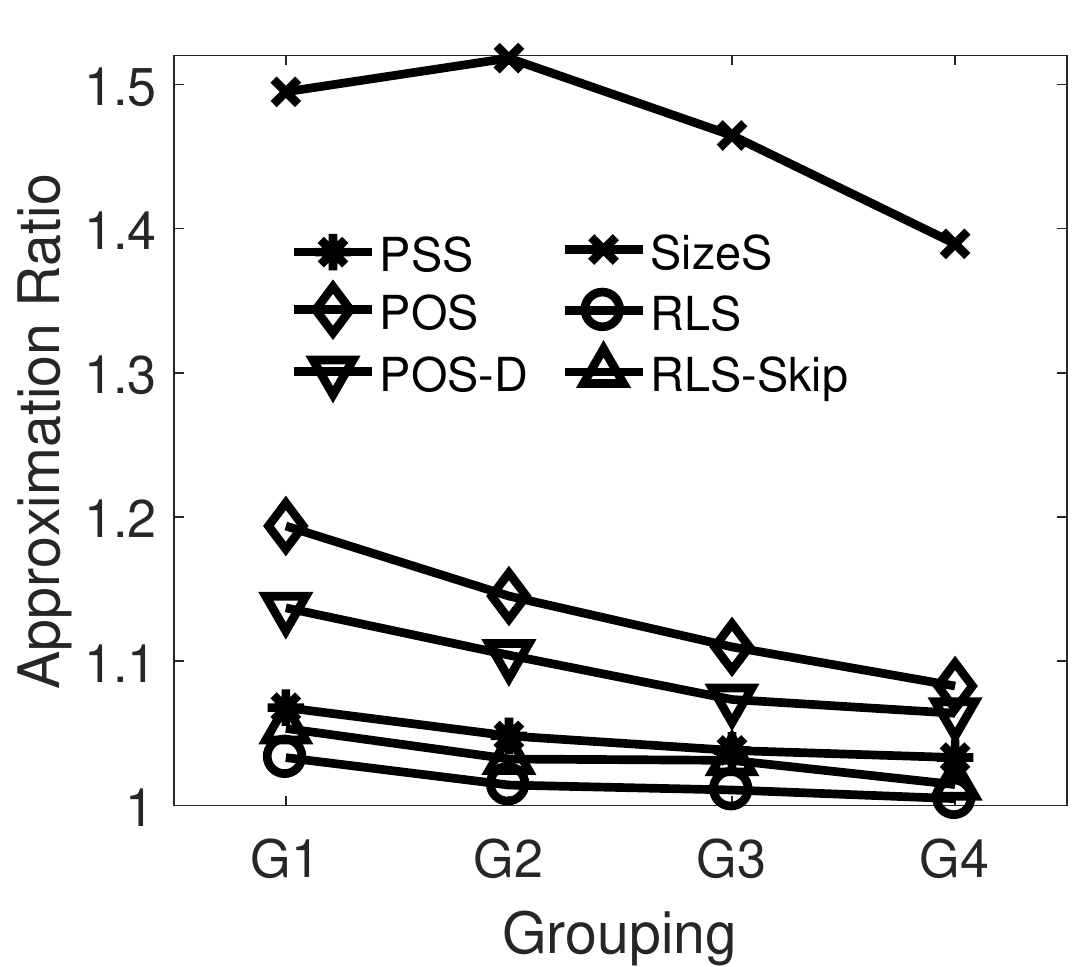}
		\end{minipage}
		&
		\begin{minipage}{2.6cm}
			\includegraphics[width=2.85cm]{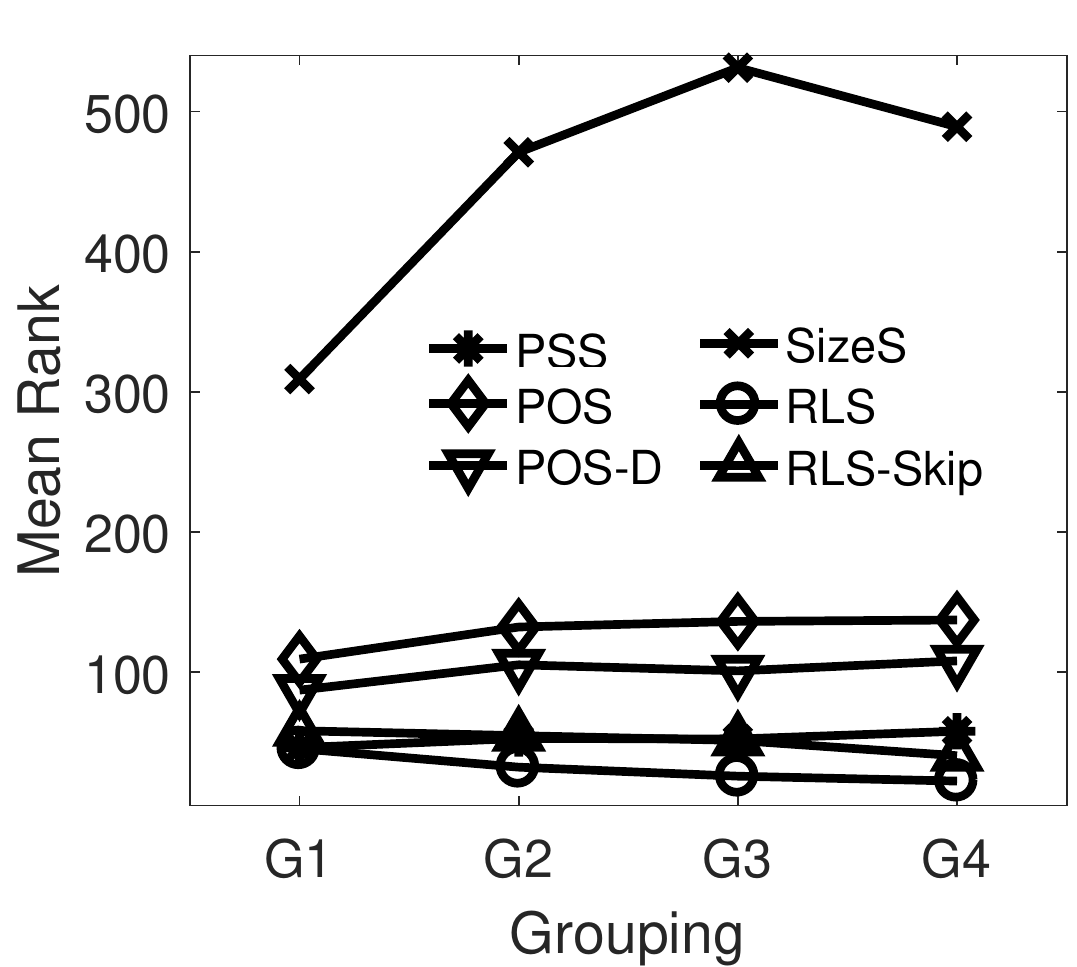}
		\end{minipage}
		&
		\begin{minipage}{2.6cm}
			\includegraphics[width=2.85cm]{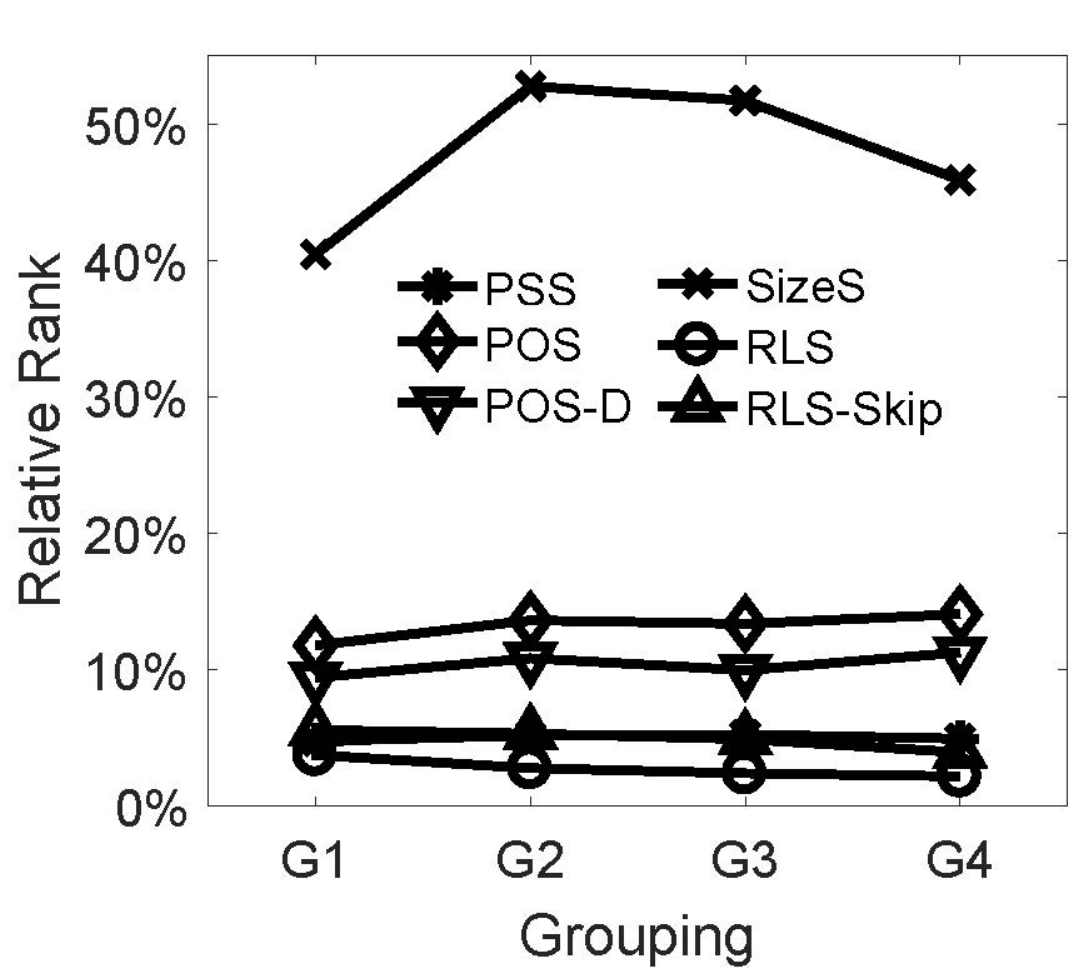}
		\end{minipage}
		&
		\begin{minipage}{2.6cm}
			\includegraphics[width=2.85cm]{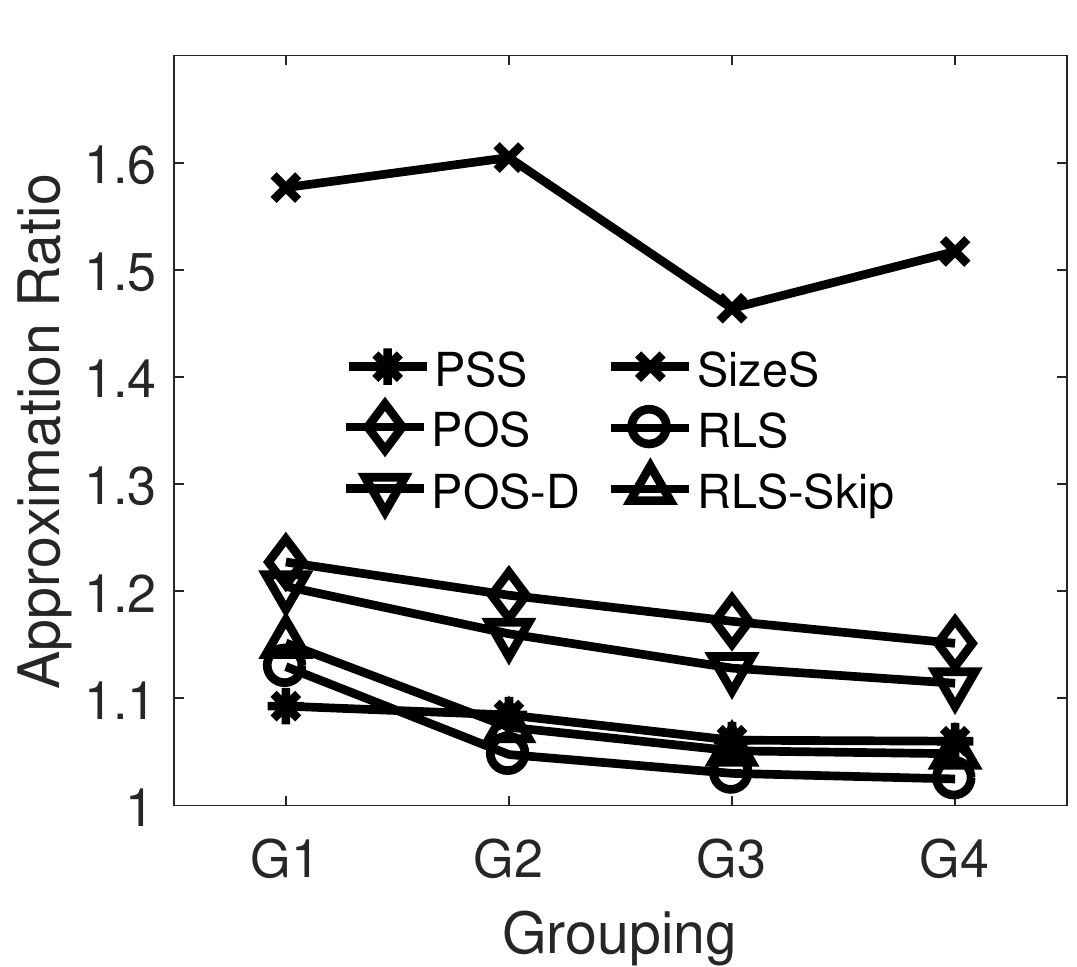}
		\end{minipage}
		&
		\begin{minipage}{2.6cm}
			\includegraphics[width=2.85cm]{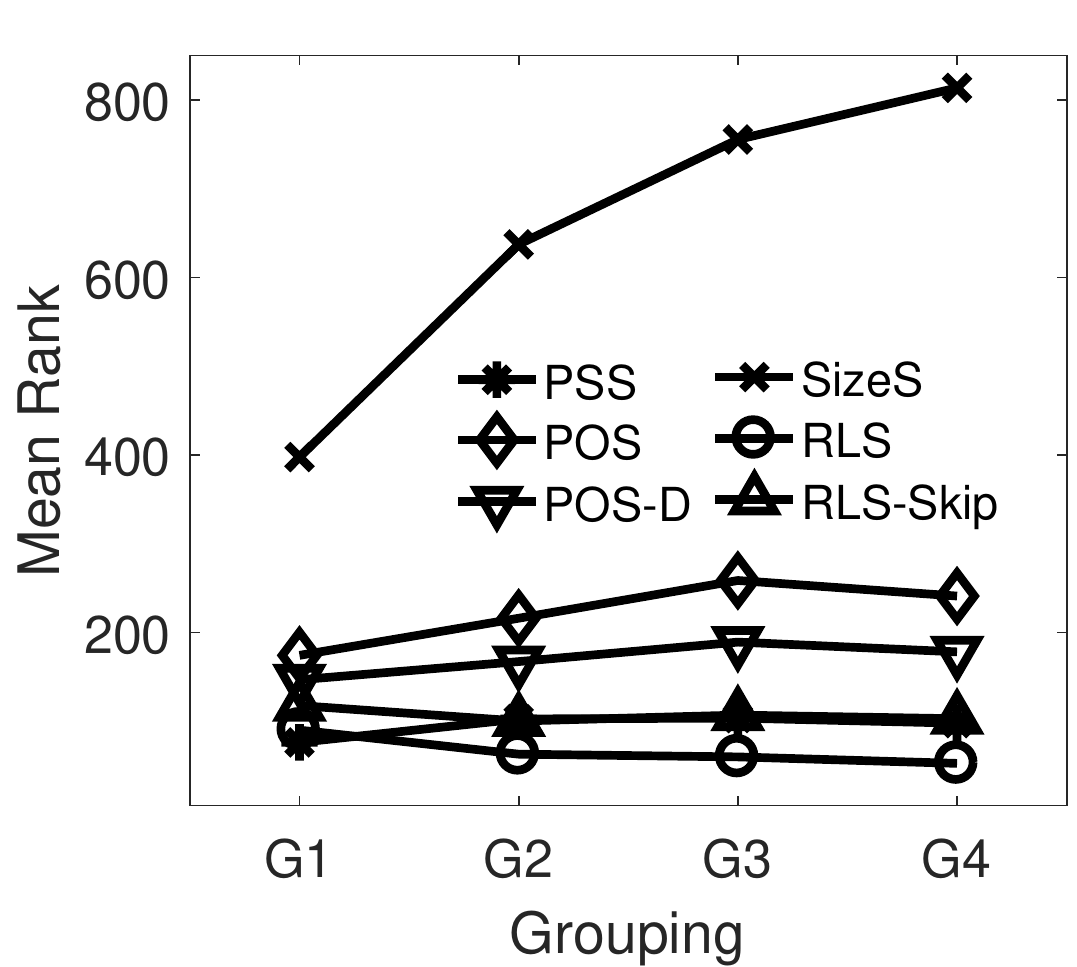}
		\end{minipage}
		&
		\begin{minipage}{2.6cm}
			\includegraphics[width=2.85cm]{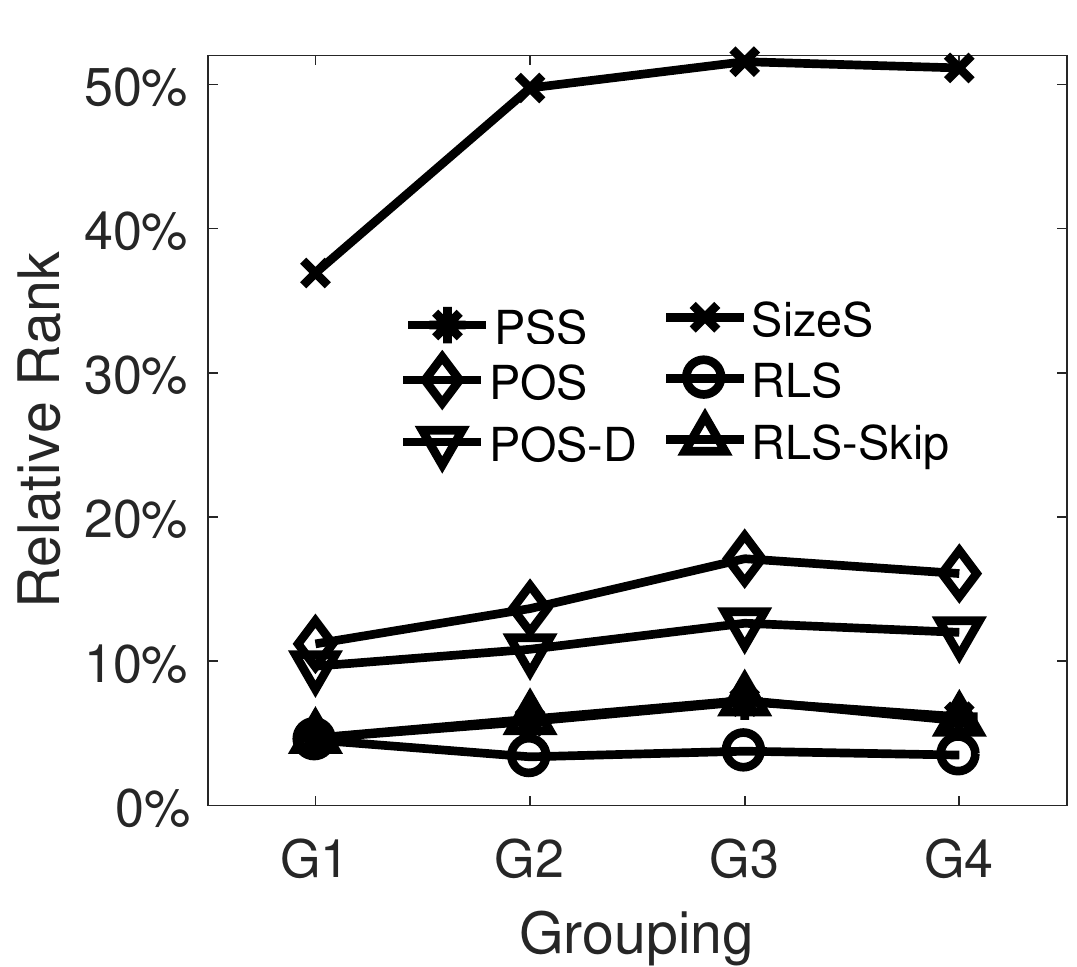}
		\end{minipage}
		\\
		\scriptsize (g) AR Porto% (DTW)
		&
		\scriptsize (h) MR Porto% (DTW)
		&
		\scriptsize (i) RR Porto% (DTW)
		&
		\scriptsize (j) AR Harbin% (DTW)
		&
		\scriptsize (k) MR Harbin% (DTW)
		&
		\scriptsize (l) RR Harbin% (DTW)
		\\
		\begin{minipage}{2.6cm}
			\includegraphics[width=2.85cm]{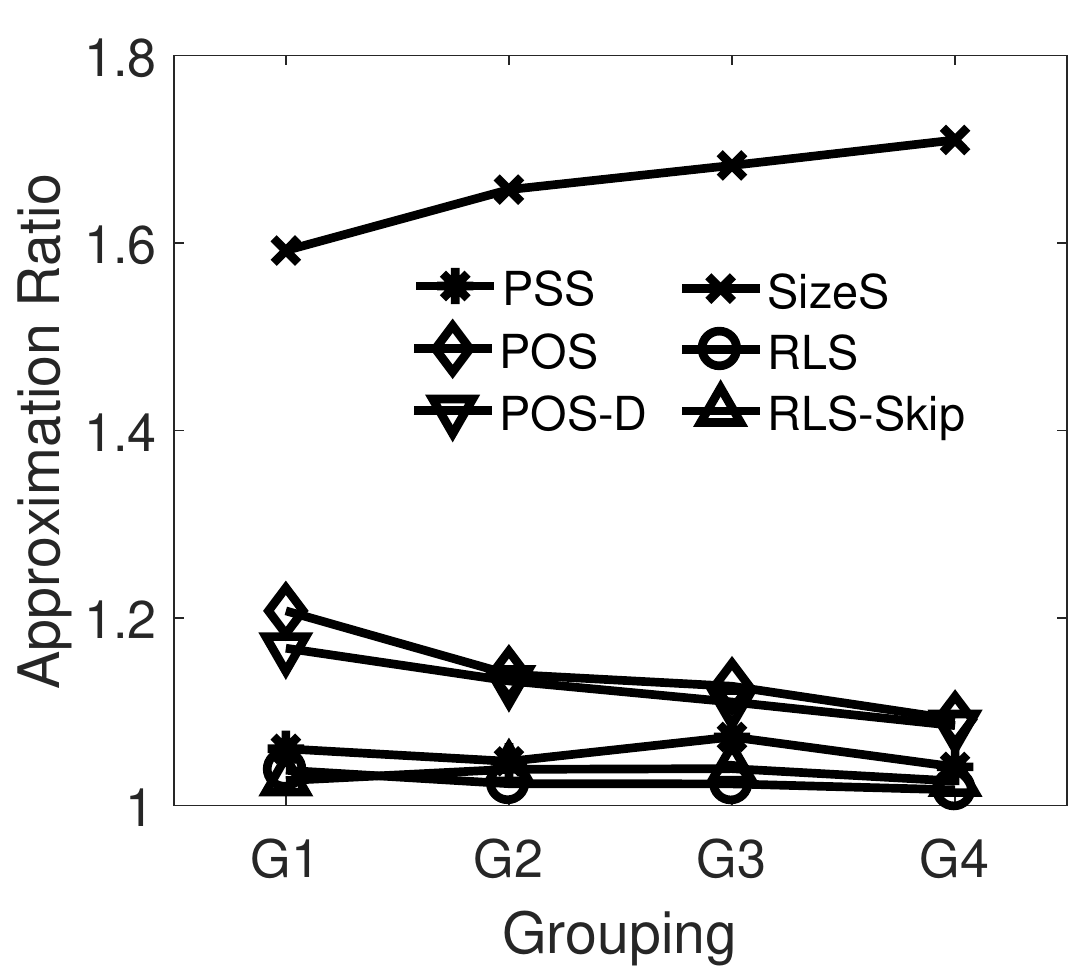}
		\end{minipage}
		&
		\begin{minipage}{2.6cm}
			\includegraphics[width=2.85cm]{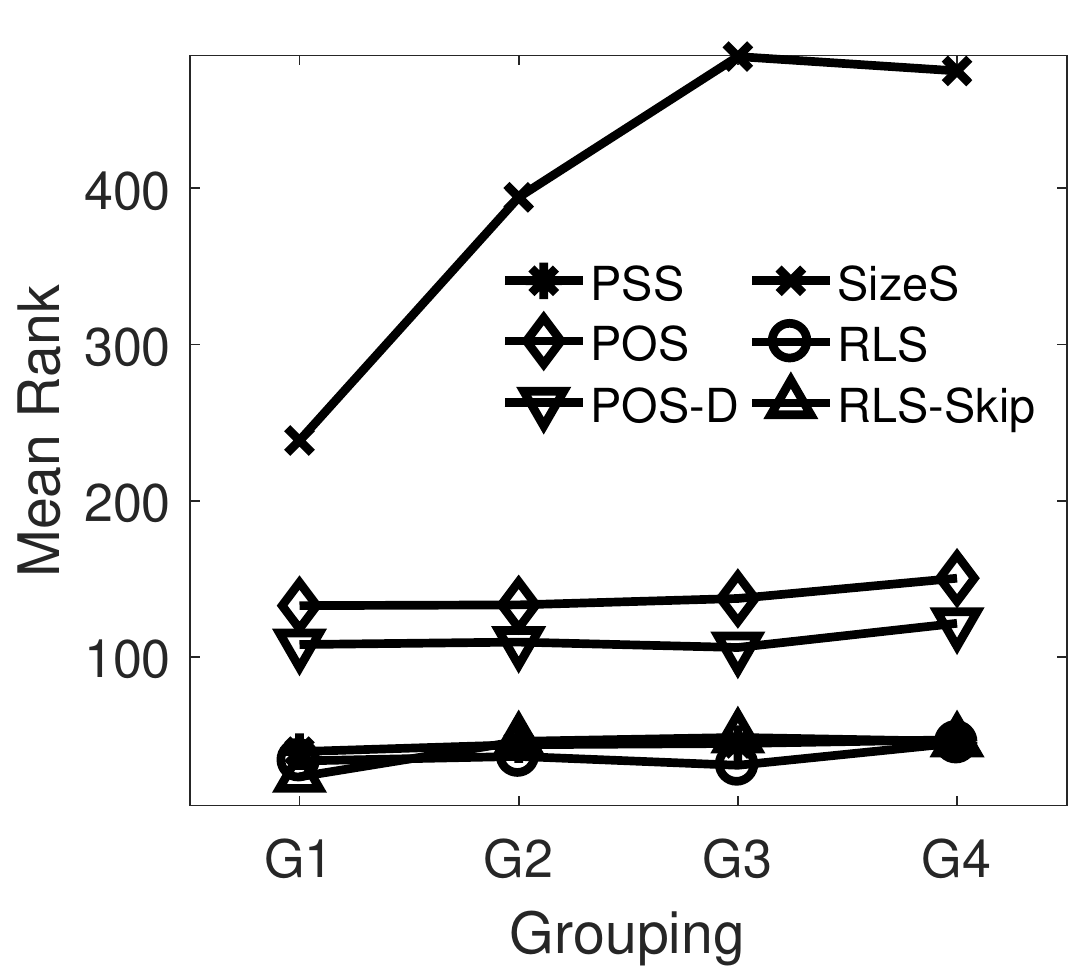}
		\end{minipage}
		&
		\begin{minipage}{2.6cm}
			\includegraphics[width=2.85cm]{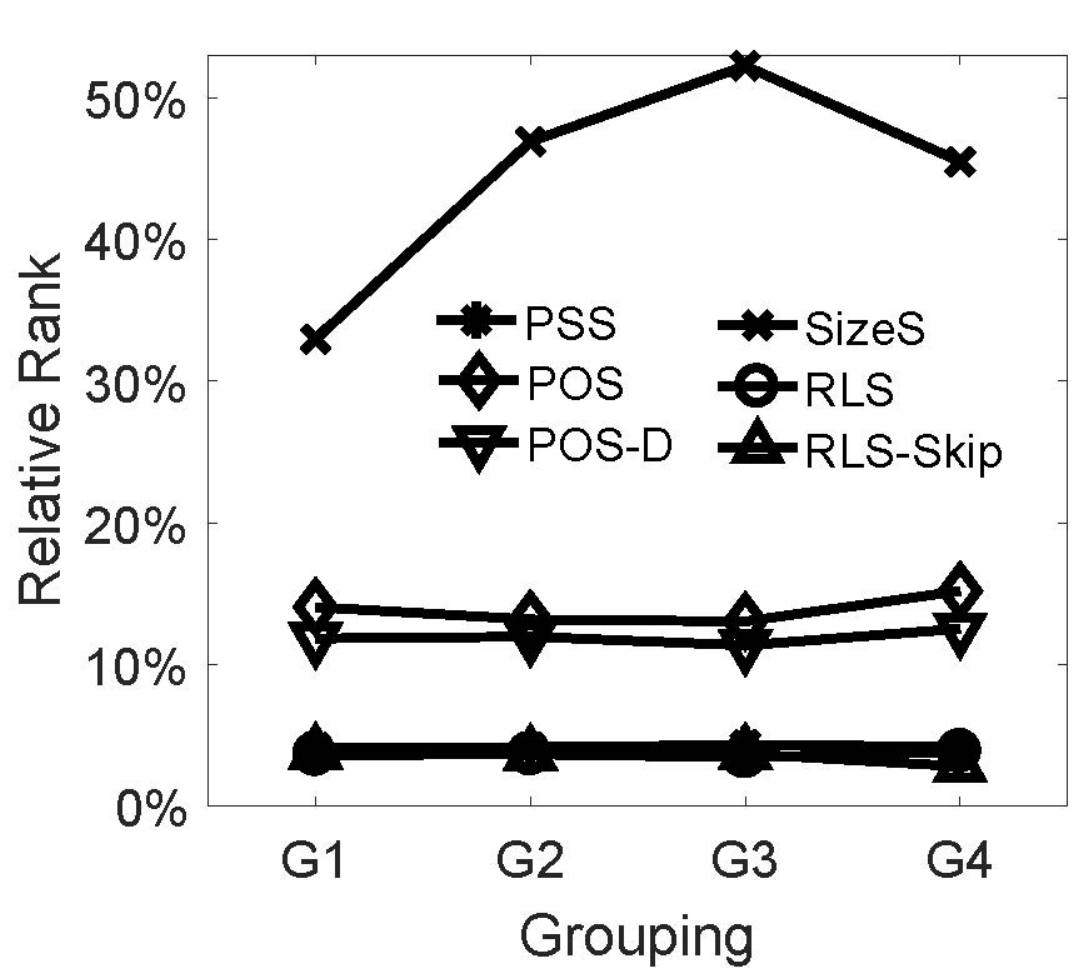}
		\end{minipage}
		&
		\begin{minipage}{2.6cm}
			\includegraphics[width=2.85cm]{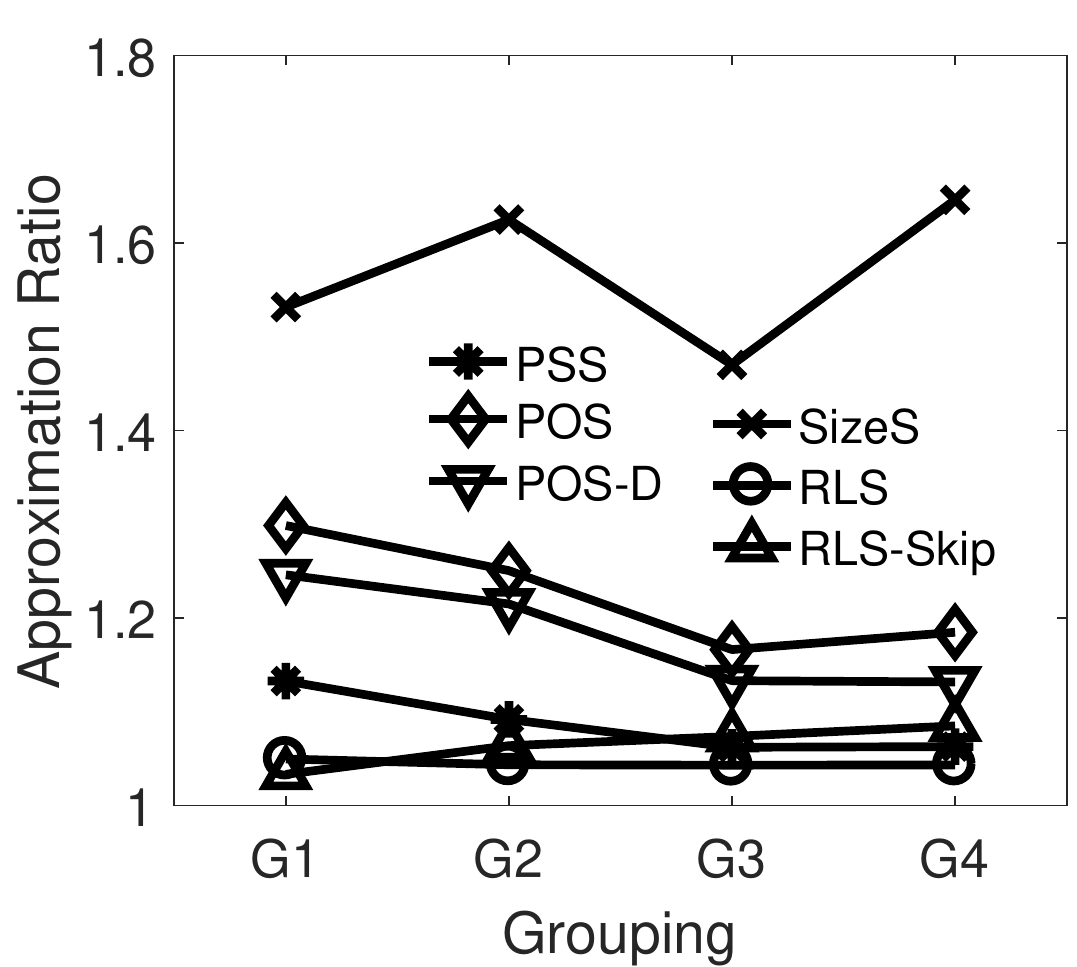}
		\end{minipage}
		&
		\begin{minipage}{2.6cm}
			\includegraphics[width=2.85cm]{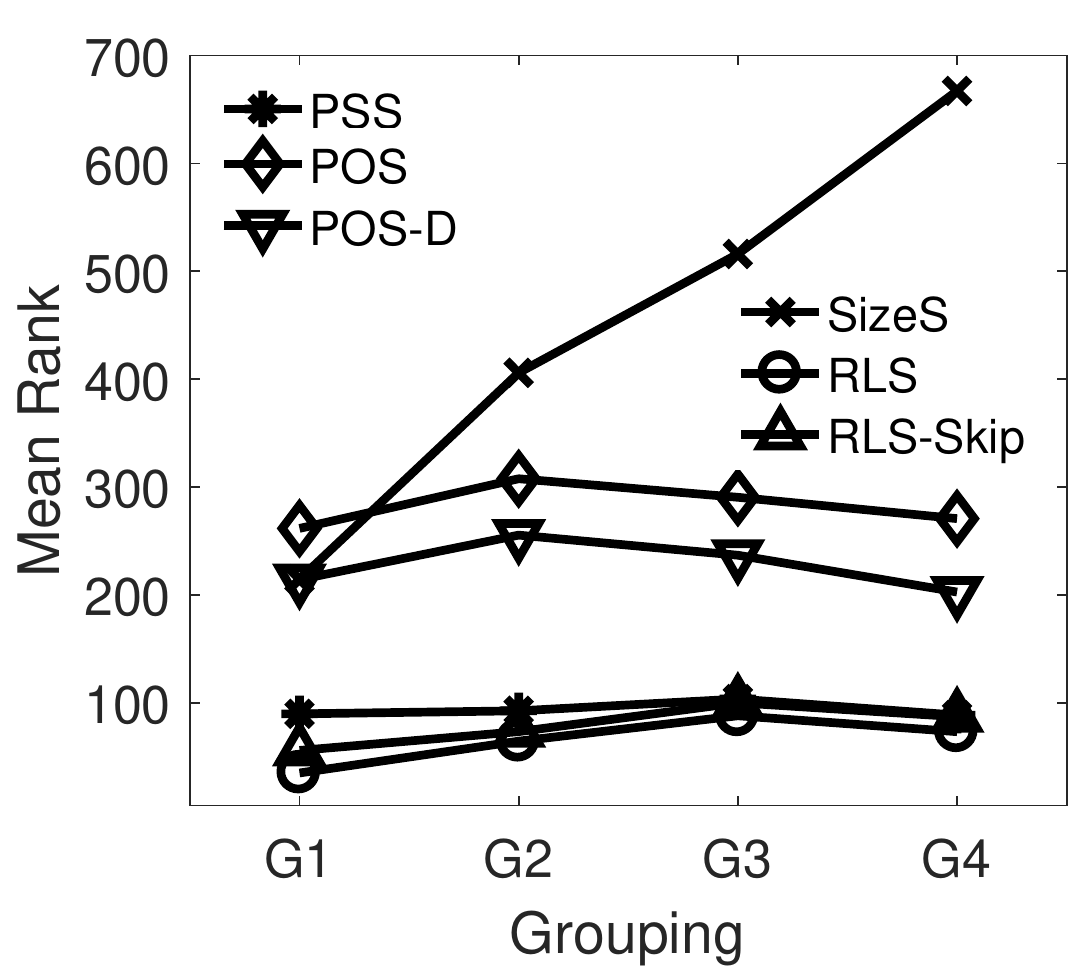}
		\end{minipage}
		&
		\begin{minipage}{2.6cm}
			\includegraphics[width=2.85cm]{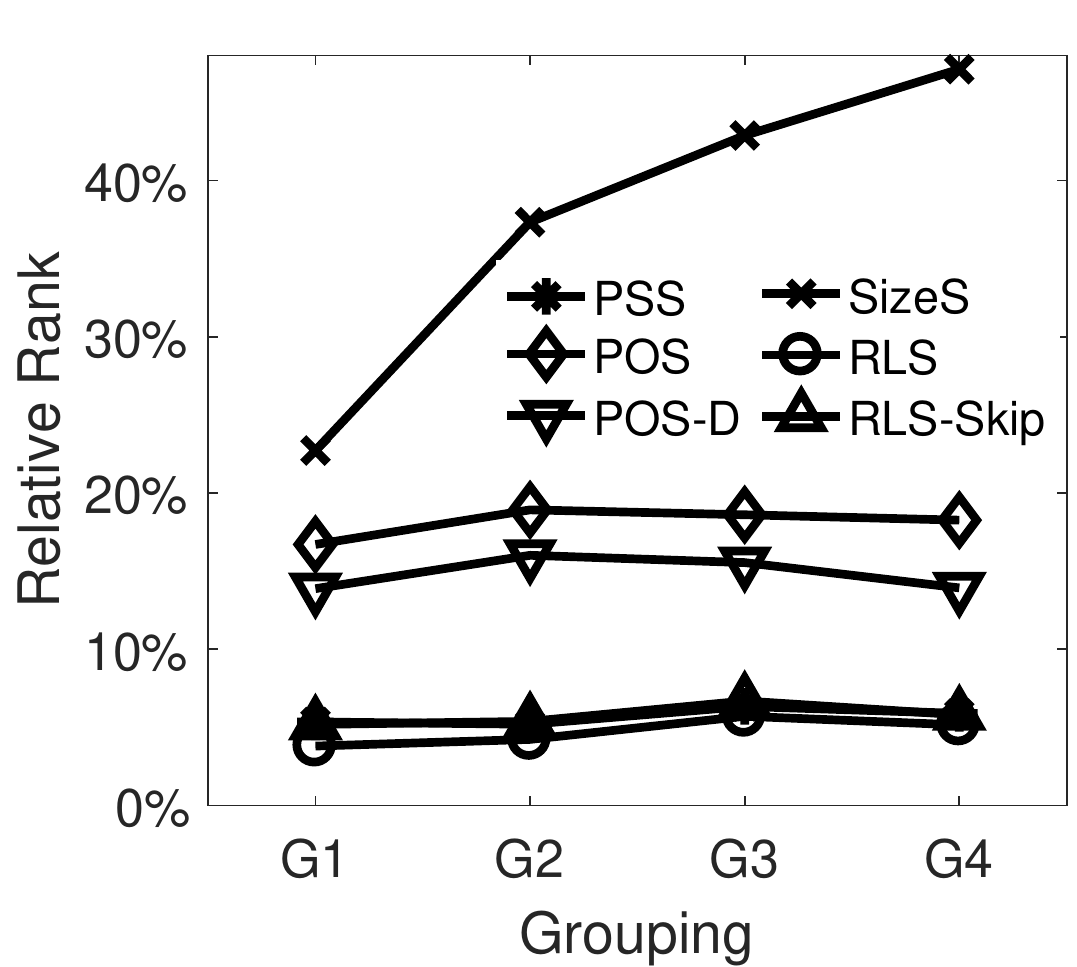}
		\end{minipage}
		\\
		\scriptsize (m) AR Porto% (Frechet)
		&
		\scriptsize (n) MR Porto% (Frechet)
		&
		\scriptsize (o) RR Porto% (Frechet)
		&
		\scriptsize (p) AR Harbin% (Frechet)
		&
		\scriptsize (q) MR Harbin% (Frechet)
		&
		\scriptsize (r) RR Harbin% (Frechet)
	\end{tabular}
	\caption{Results of grouping evaluation for t2vec (a)-(f), DTW (g)-(l) and Frechet (m)-(r).}
	\label{fig:groupingRLS_ph}
	%\vspace*{-2mm}
\end{figure*}

\begin{figure*}
	\hspace*{-.5cm}
	\centering
	\begin{tabular}{c c c c}
		%  \begin{minipage}{4cm}
		%  \includegraphics[width=4.15cm]{t2v_ar}
		%  \end{minipage}
		%  &
		%  \begin{minipage}{4cm}
		%    \includegraphics[width=4.15cm]{t2v_mr}
		%  \end{minipage}
		%  &
		%  \begin{minipage}{4cm}
		%  \includegraphics[width=4.15cm]{t2v_rr}
		%  \end{minipage}
		%  &
		%  \begin{minipage}{4cm}
		%    \includegraphics[width=4.15cm]{t2v_time}
		%  \end{minipage}
		%  \\
		%  \small (a) Approximation Ratio (t2vec)
		%  &
		%  \small (b) Mean Rank (t2vec)
		%  &
		%  \small (c) Relative Rank (t2vec)
		%  &
		%  \small (d) Time Cost (t2vec)
		%  \\
		\begin{minipage}{4cm}
			\includegraphics[width=4.15cm]{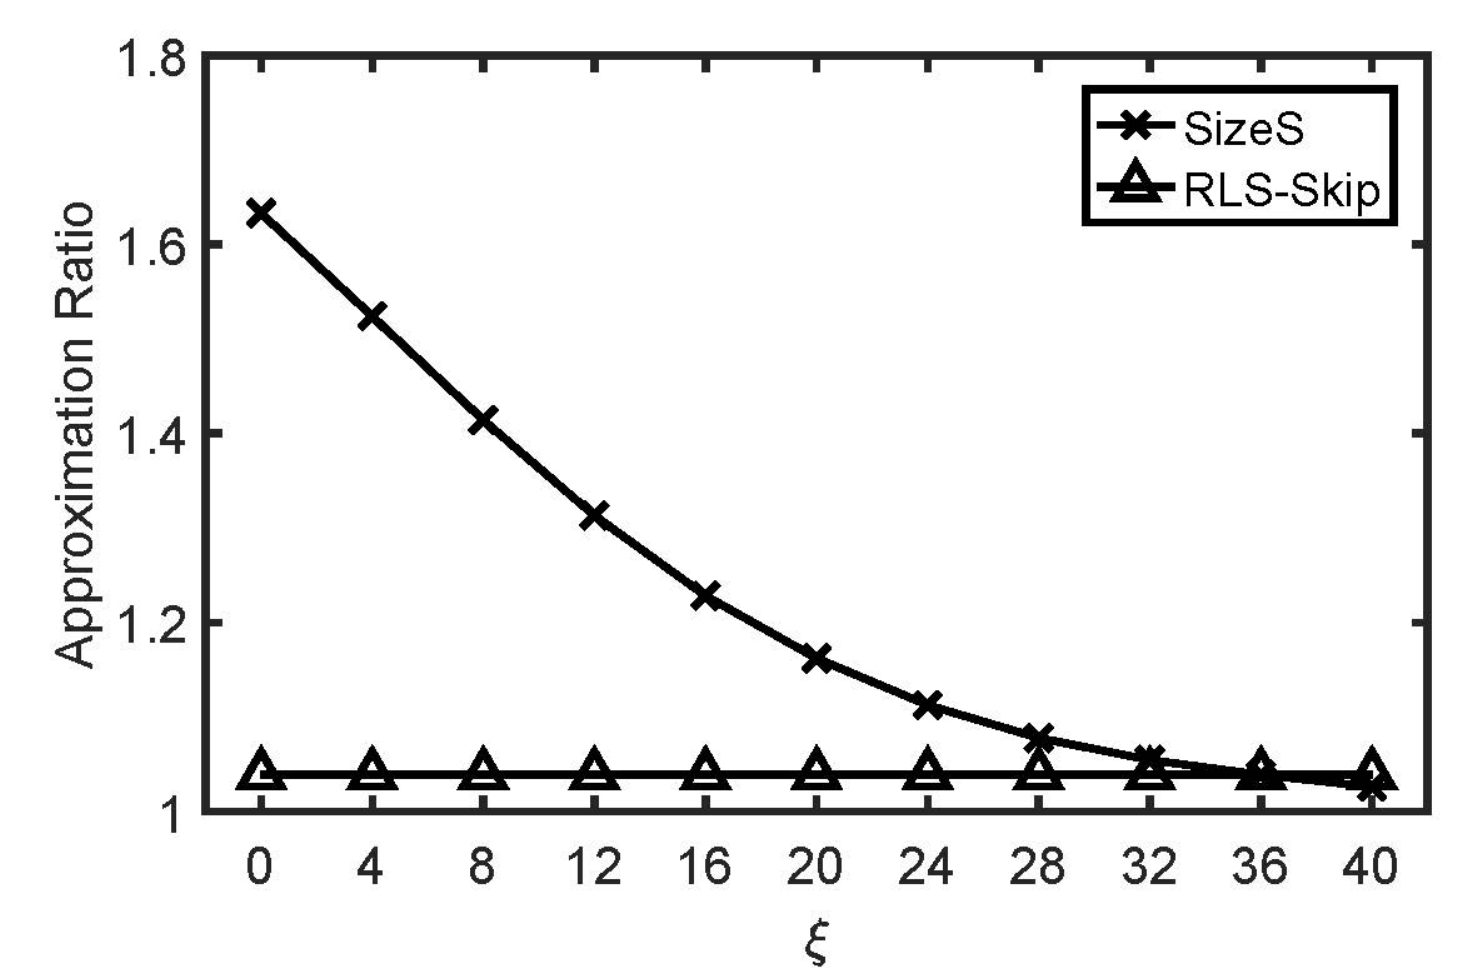}
		\end{minipage}
		&
		\begin{minipage}{4cm}
			\includegraphics[width=4.15cm]{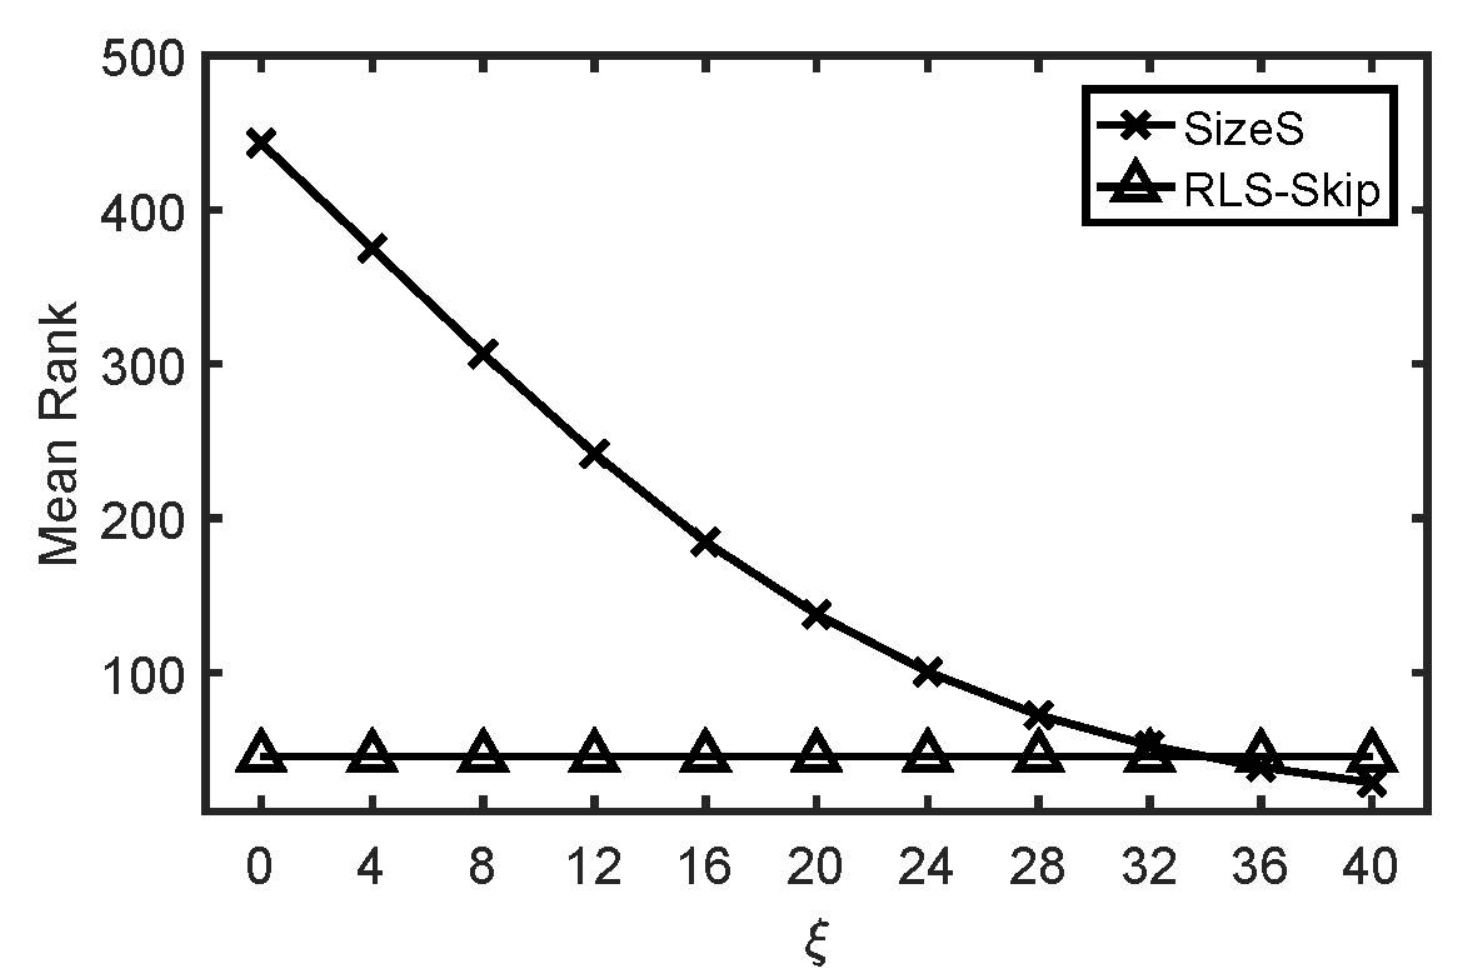}
		\end{minipage}
		&
		\begin{minipage}{4cm}
			\includegraphics[width=4.15cm]{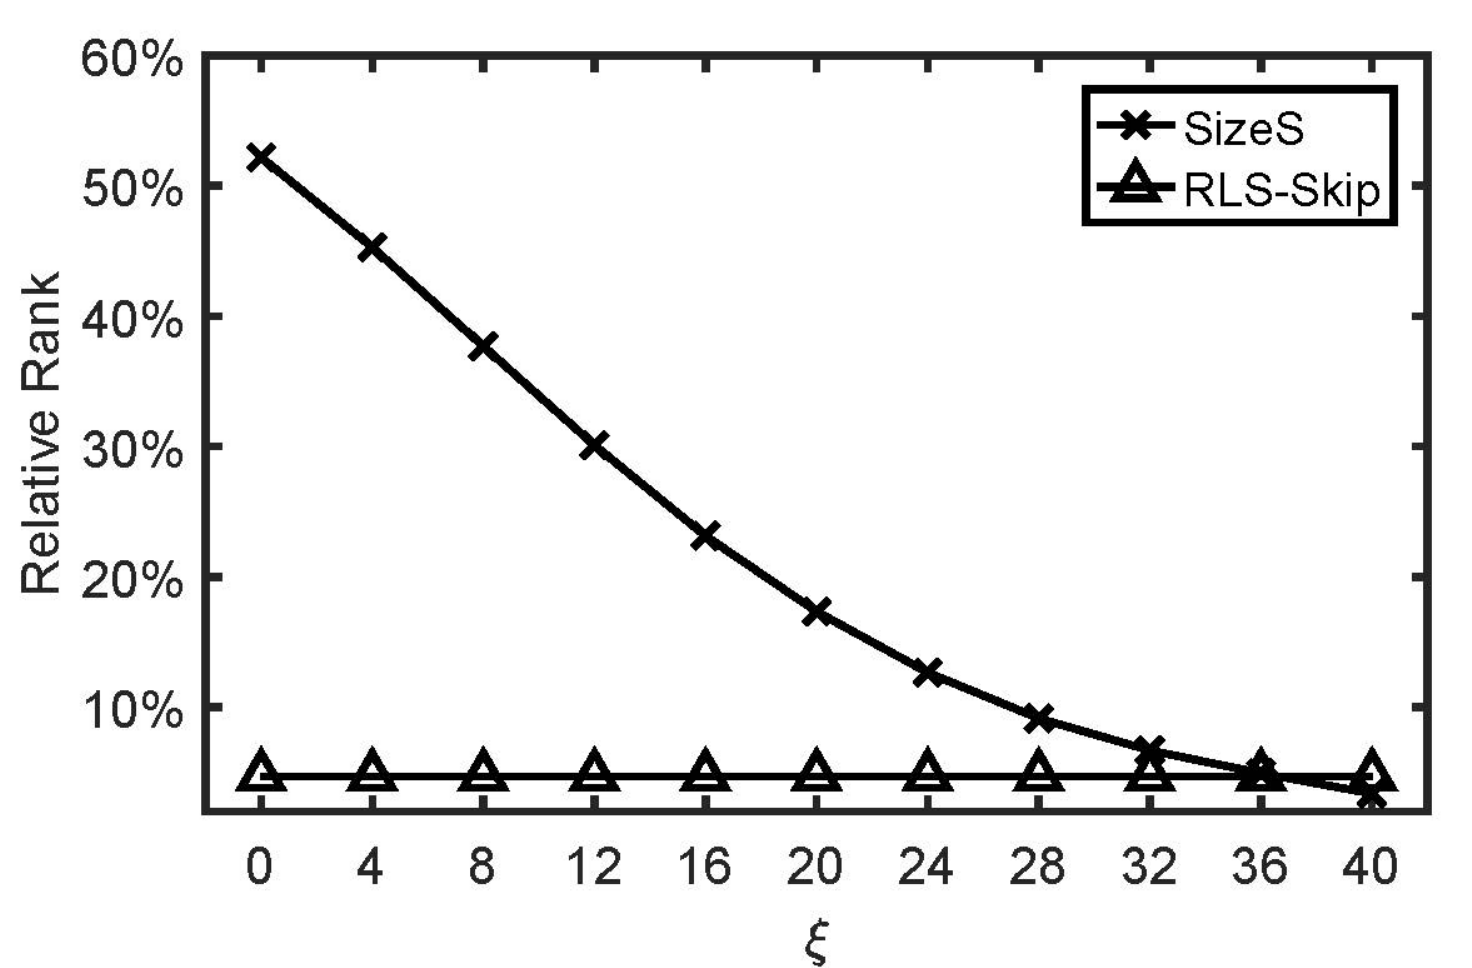}
		\end{minipage}
		&
		\begin{minipage}{4cm}
			\includegraphics[width=4.15cm]{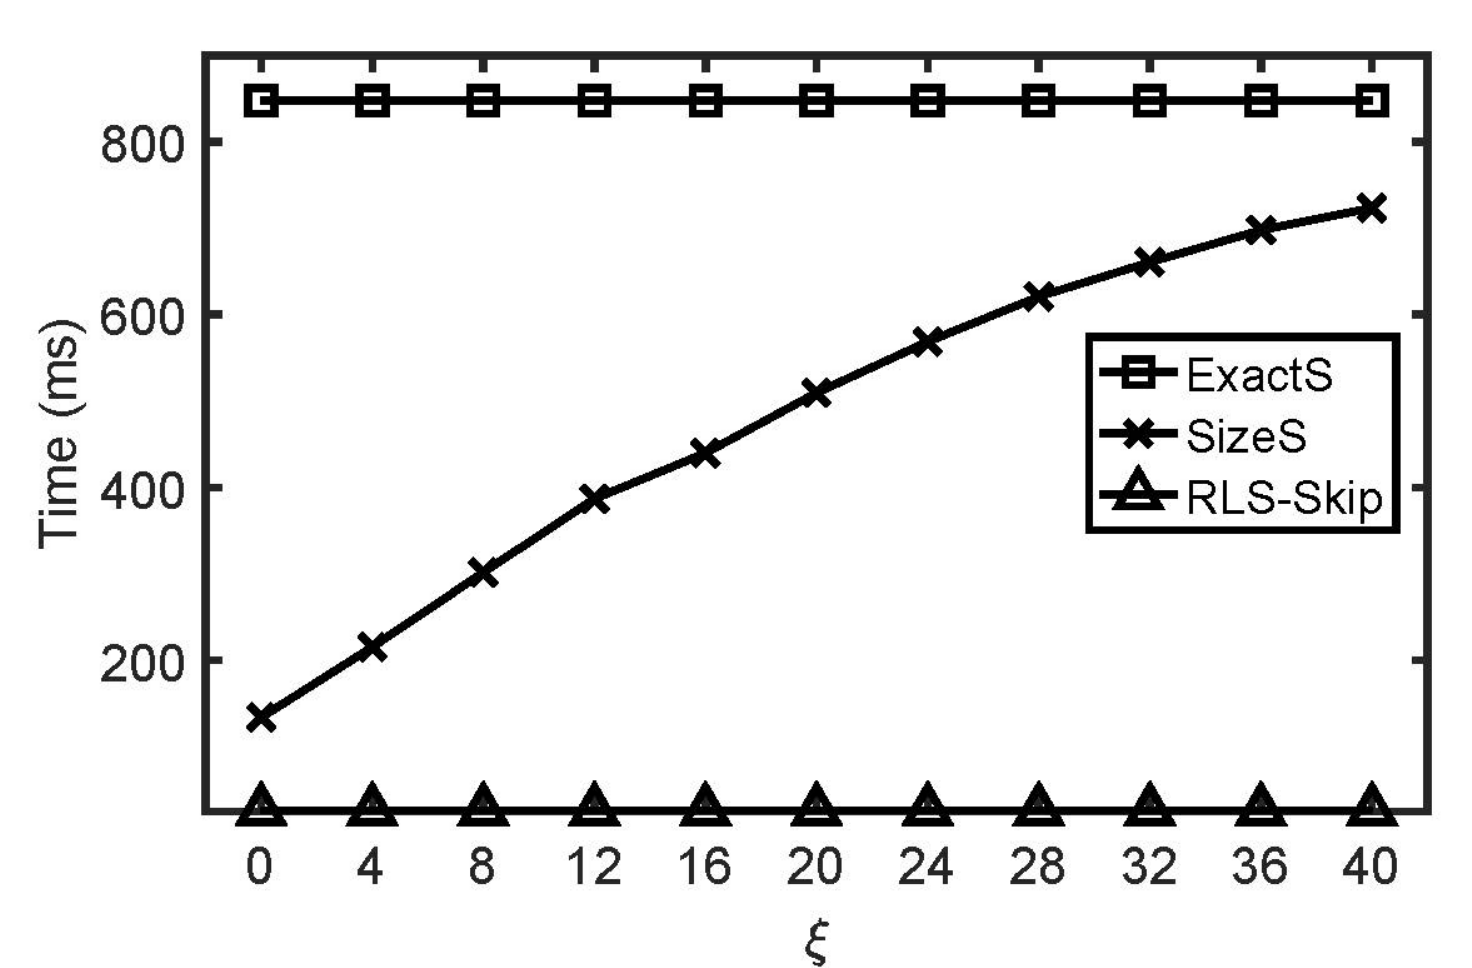}
		\end{minipage}
		\\
		\small (a) Approximation Ratio (DTW)
		&
		\small (b) Mean Rank (DTW)
		&
		\small (c) Relative Rank (DTW)
		&
		\small (d) Time Cost (DTW)
		\\
		%  \begin{minipage}{4cm}
		%  \includegraphics[width=4.15cm]{fre_ar}
		%  \end{minipage}
		%  &
		%  \begin{minipage}{4cm}
		%    \includegraphics[width=4.15cm]{fre_mr}
		%  \end{minipage}
		%  &
		%  \begin{minipage}{4cm}
		%  \includegraphics[width=4.15cm]{fre_rr}
		%  \end{minipage}
		%  &
		%  \begin{minipage}{4cm}
		%    \includegraphics[width=4.15cm]{fre_time}
		%  \end{minipage}
		%  \\
		%  \small (i) Approximation Ratio (Frechet)
		%  &
		%  \small (j) Mean Rank (Frechet)
		%  &
		%  \small (k) Relative Rank (Frechet)
		%  &
		%  \small (l) Time Cost (Frechet)
	\end{tabular}
	%\vspace*{-2mm}
	\caption{The effect of soft margin $\xi$ for SizeS.}
	%\vspace*{-3mm}
	\label{para_fls_sizes}
	%\vspace*{-0.5mm}
\end{figure*}

\begin{figure*}[!th]
\centering
\begin{tabular}{c c c}
  \begin{minipage}{4.5cm}%5.5
	\includegraphics[width=4.5cm]{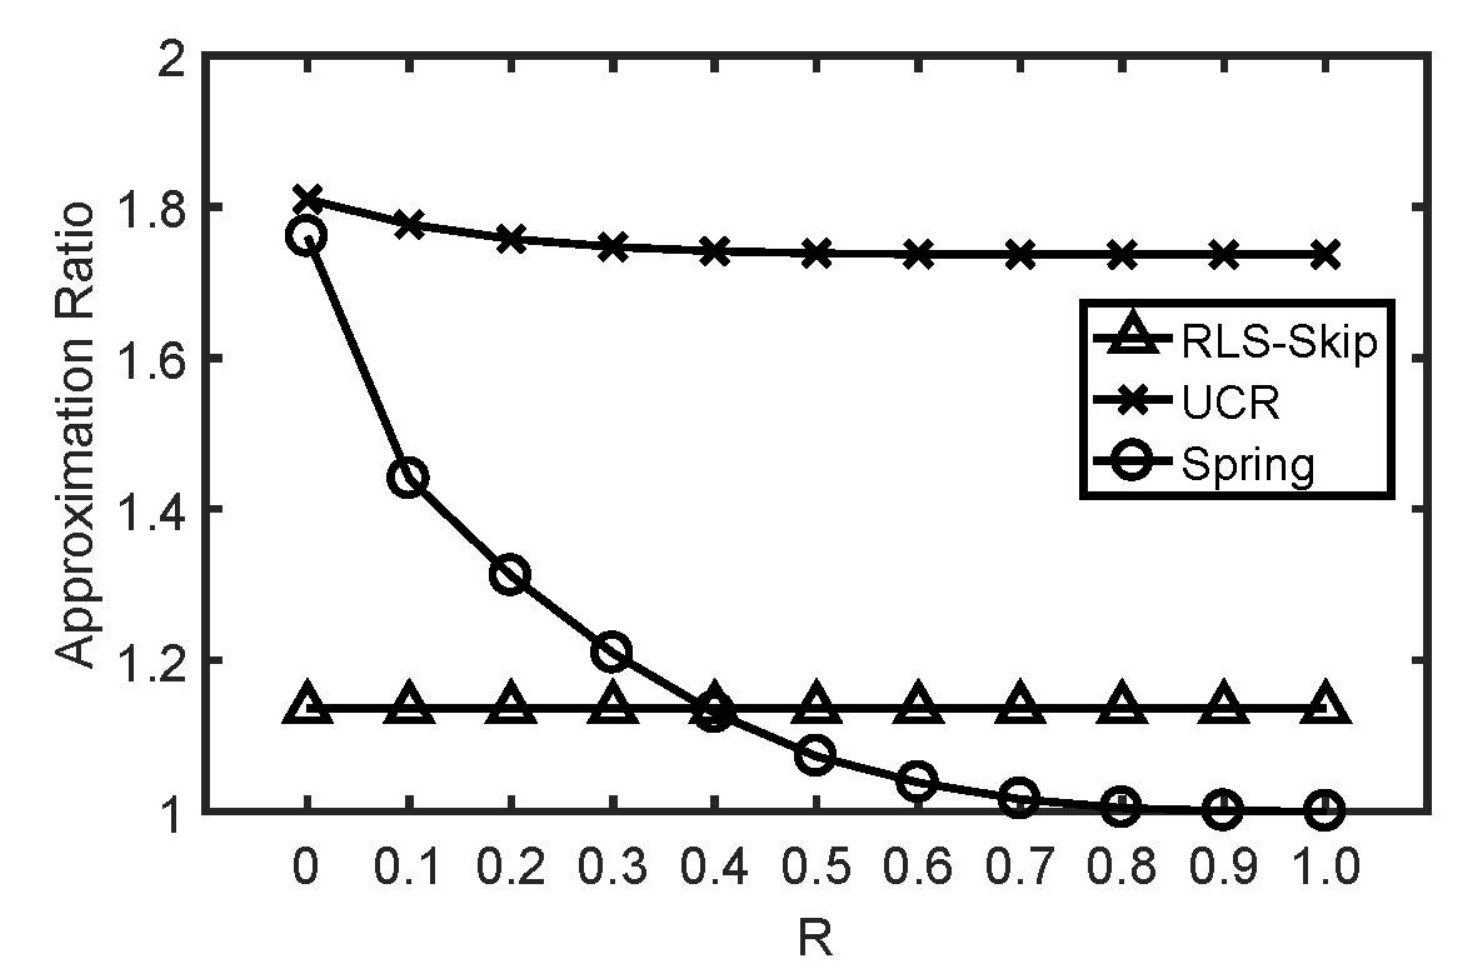}
  \end{minipage}
  &
  \begin{minipage}{4.5cm}
	\includegraphics[width=4.5cm]{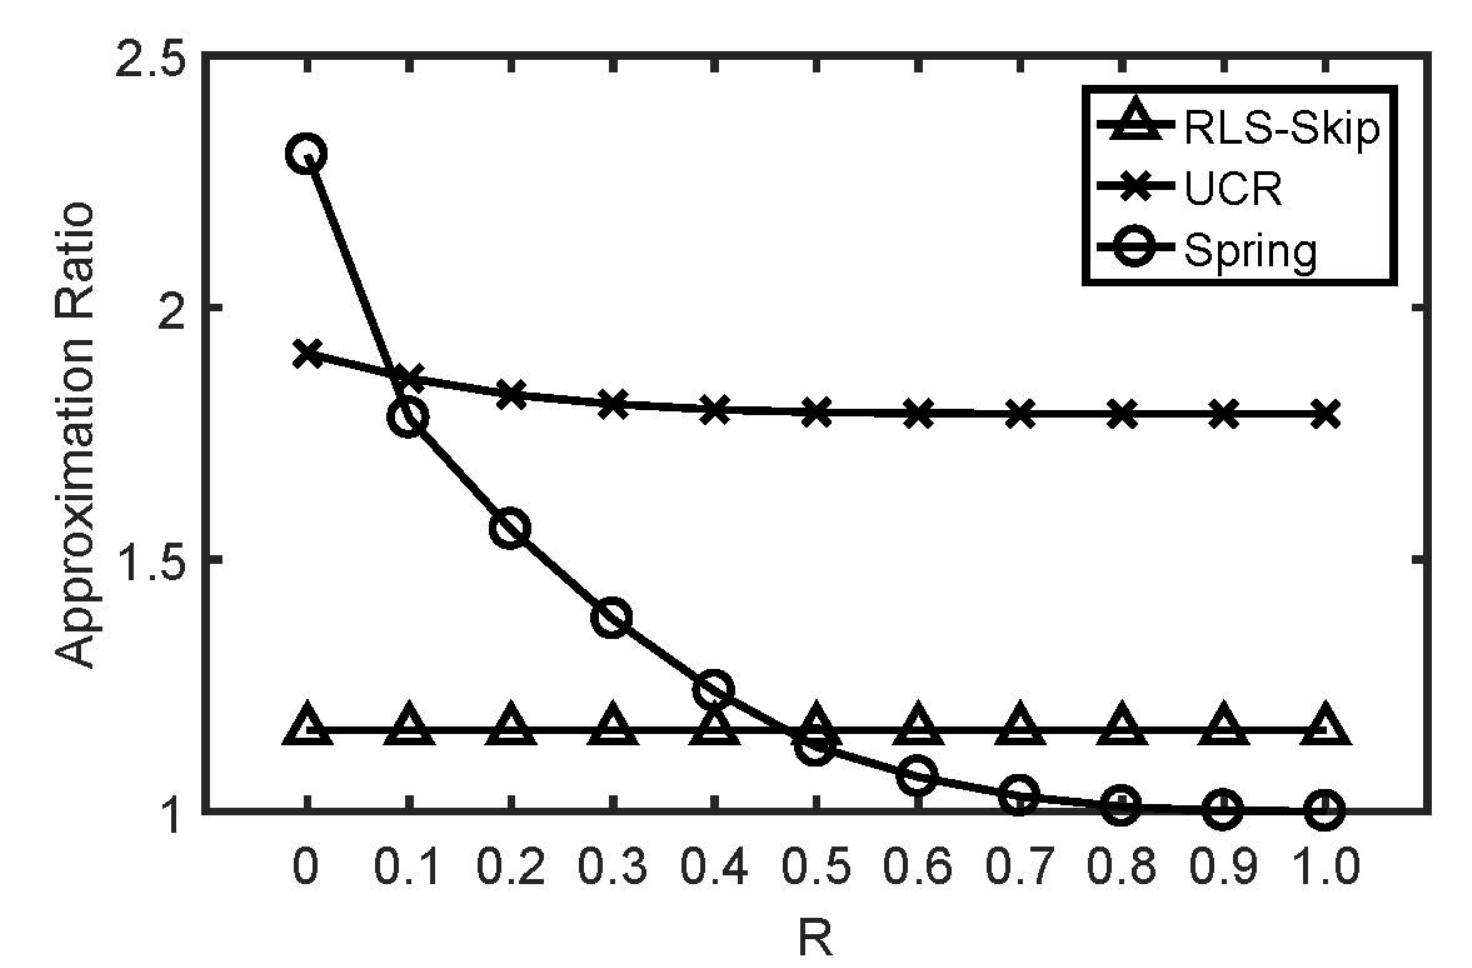}
  \end{minipage}
  &
  \begin{minipage}{4.5cm}
	\includegraphics[width=4.5cm]{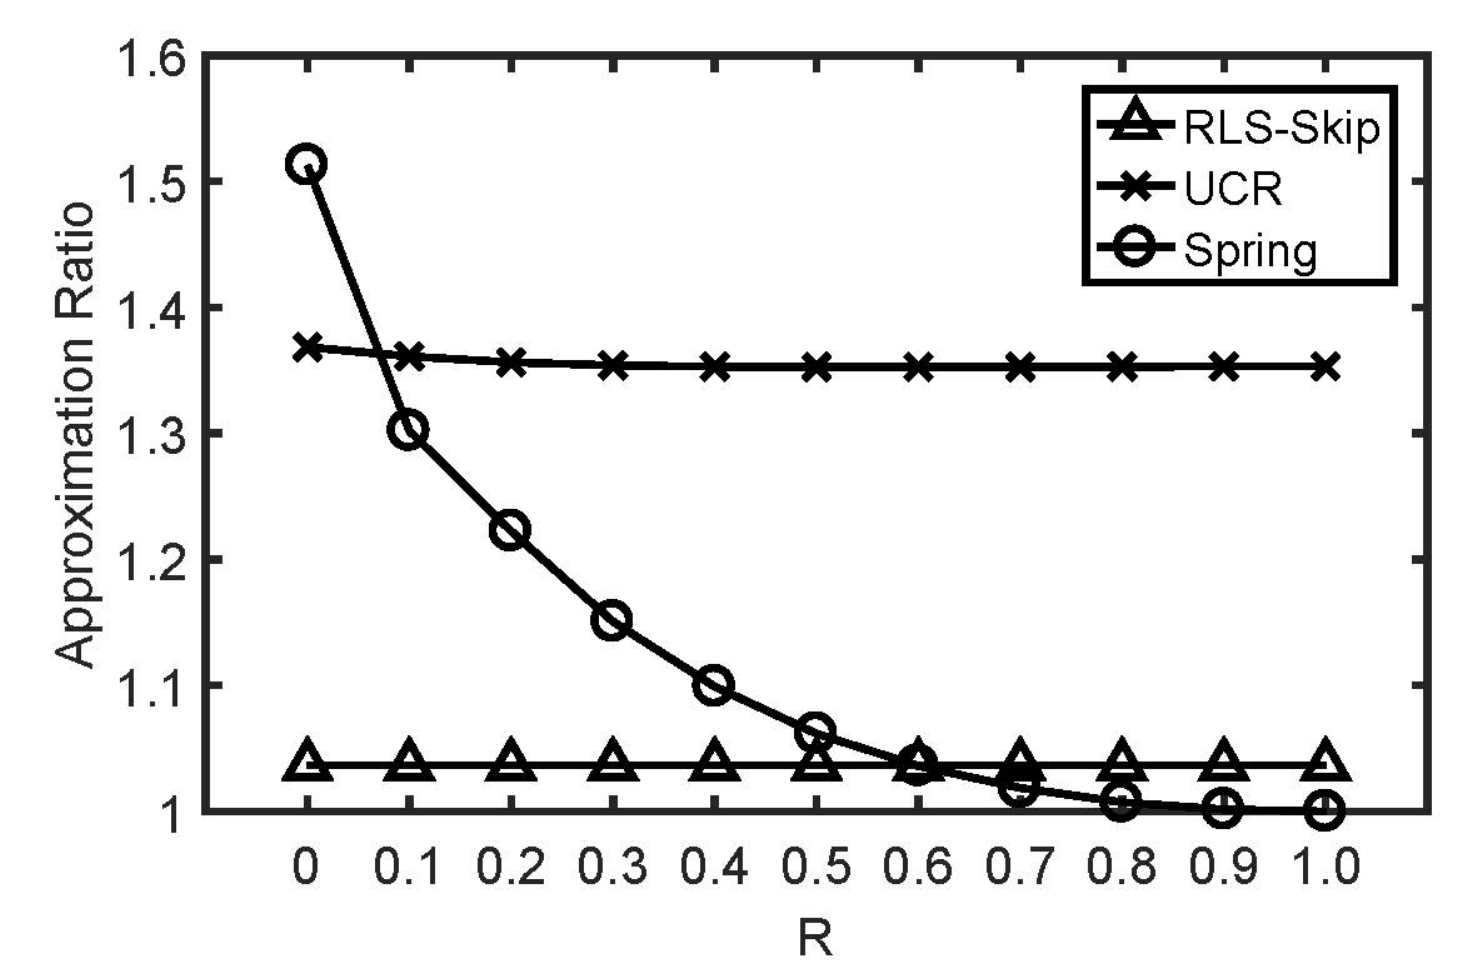}
  \end{minipage}
  \\
  \scriptsize{(a) Approximation Ratio (Porto)}
  &
  \scriptsize{(b) Approximation Ratio (Harbin)}
  &
  \scriptsize{(c) Approximation Ratio (Sports)}
  \\
  \begin{minipage}{4.5cm}%5.5
	\includegraphics[width=4.5cm]{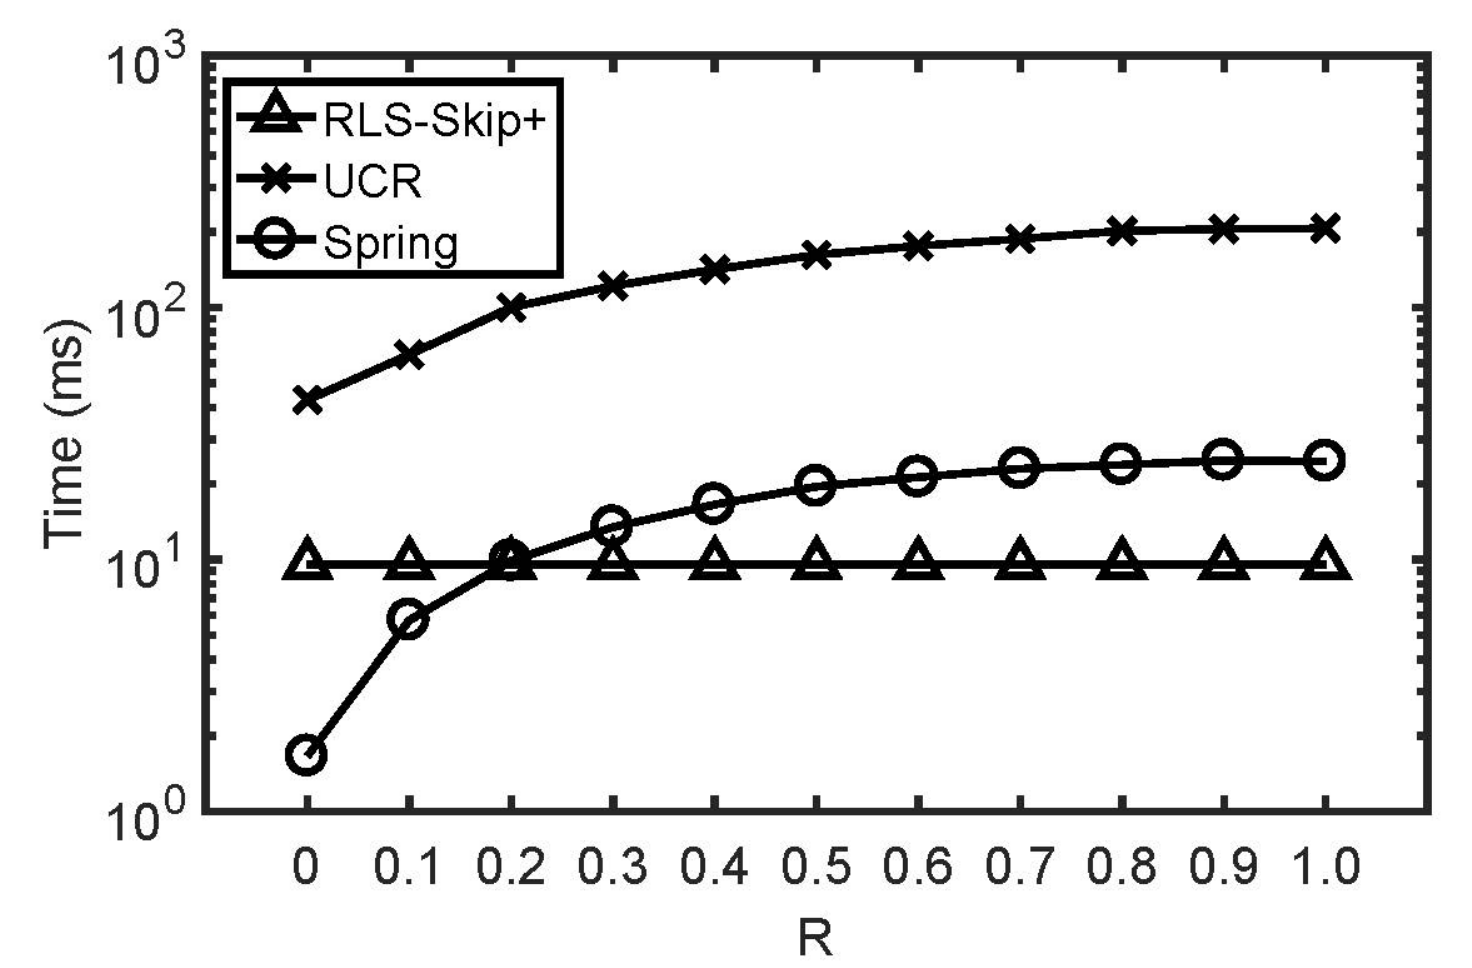}
  \end{minipage}
  &
  \begin{minipage}{4.5cm}%5.5
	\includegraphics[width=4.5cm]{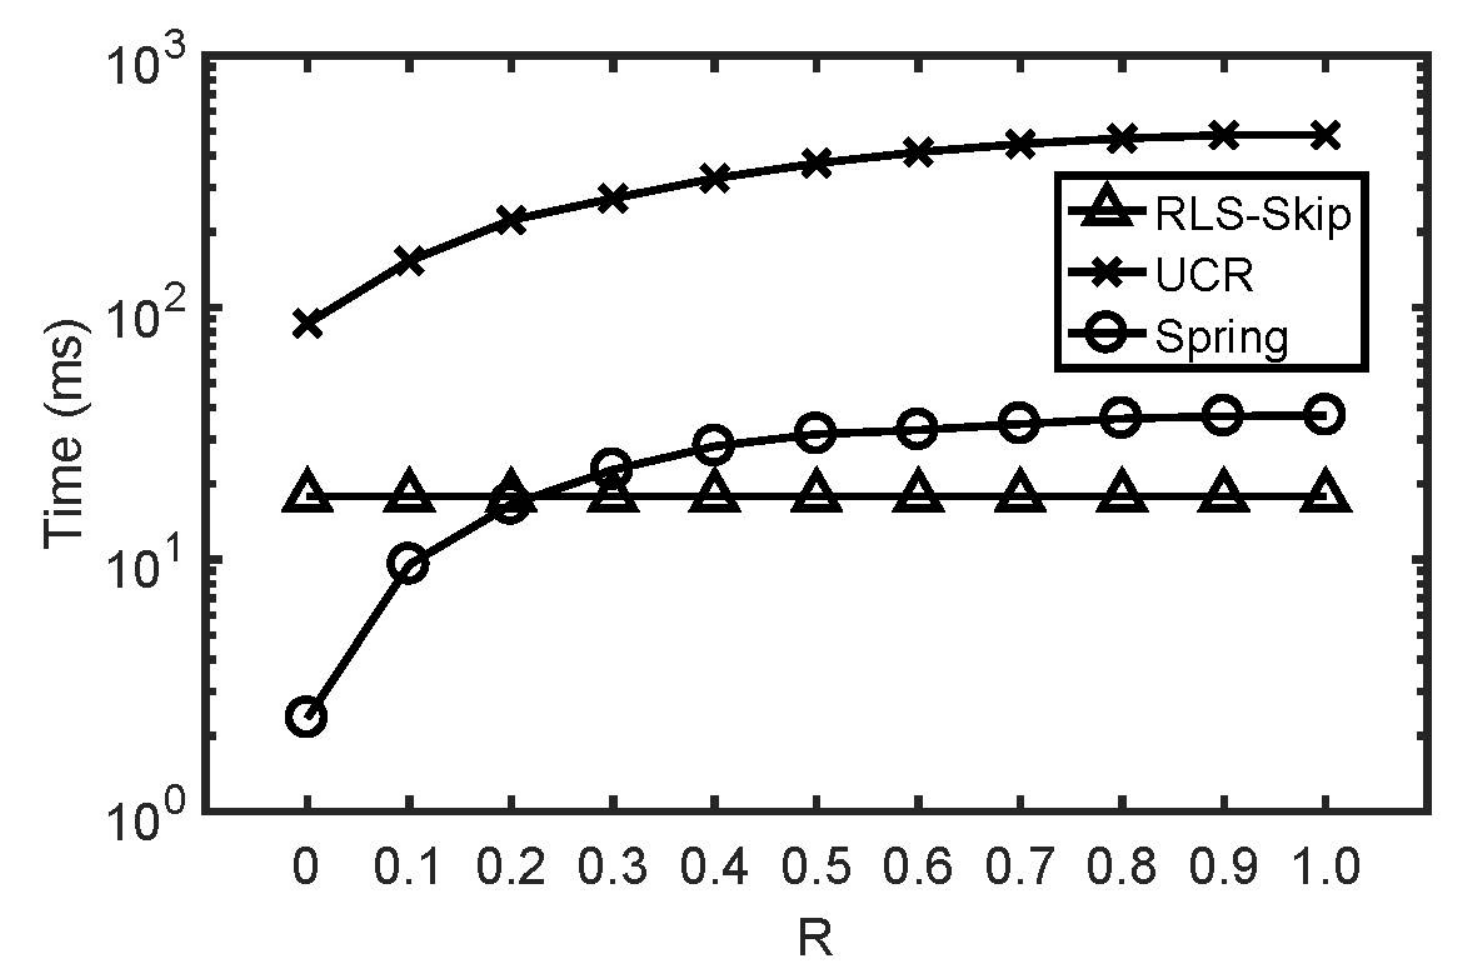}
  \end{minipage}
  &
  \begin{minipage}{4.5cm}%5.5
	\includegraphics[width=4.5cm]{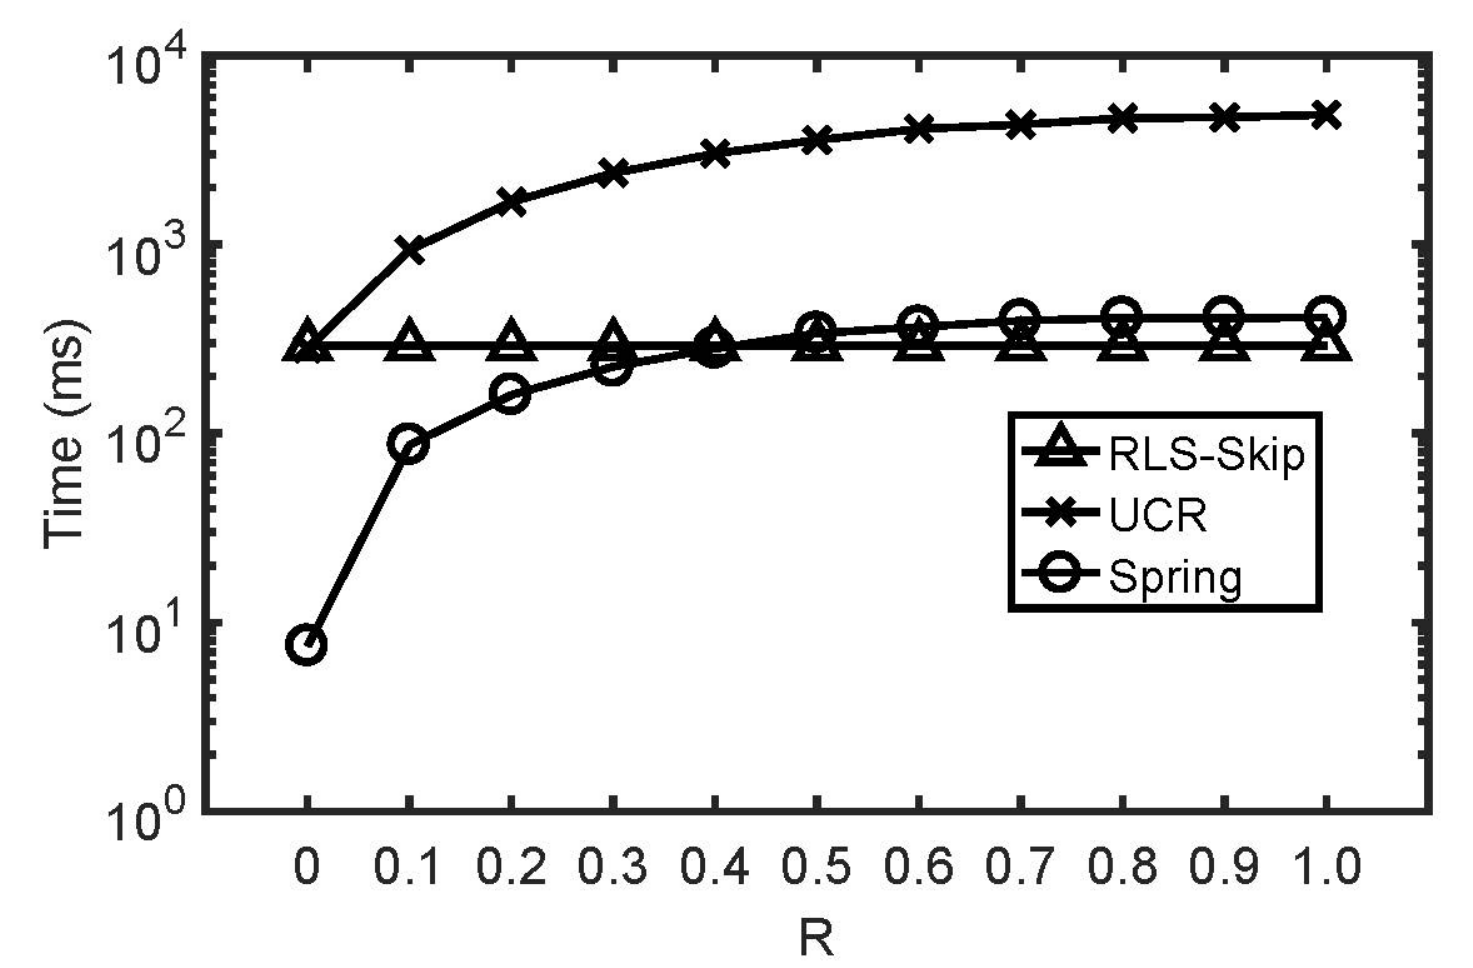}
  \end{minipage}
  \\
  \scriptsize{(d) Time Cost (Porto)}
  &
  \scriptsize{(e) Time Cost (Harbin)}
  &
  \scriptsize{(f) Time Cost (Sports)}
  \end{tabular}
\caption{Comparison with UCR and Spring.}
\label{ucr_result_full}
%\vspace*{-2mm}
\end{figure*}

\if 0
\begin{figure*}
	\hspace*{-.5cm}
	\centering
	\begin{tabular}{c c c c}
		\begin{minipage}{4cm}
			\includegraphics[width=4.15cm]{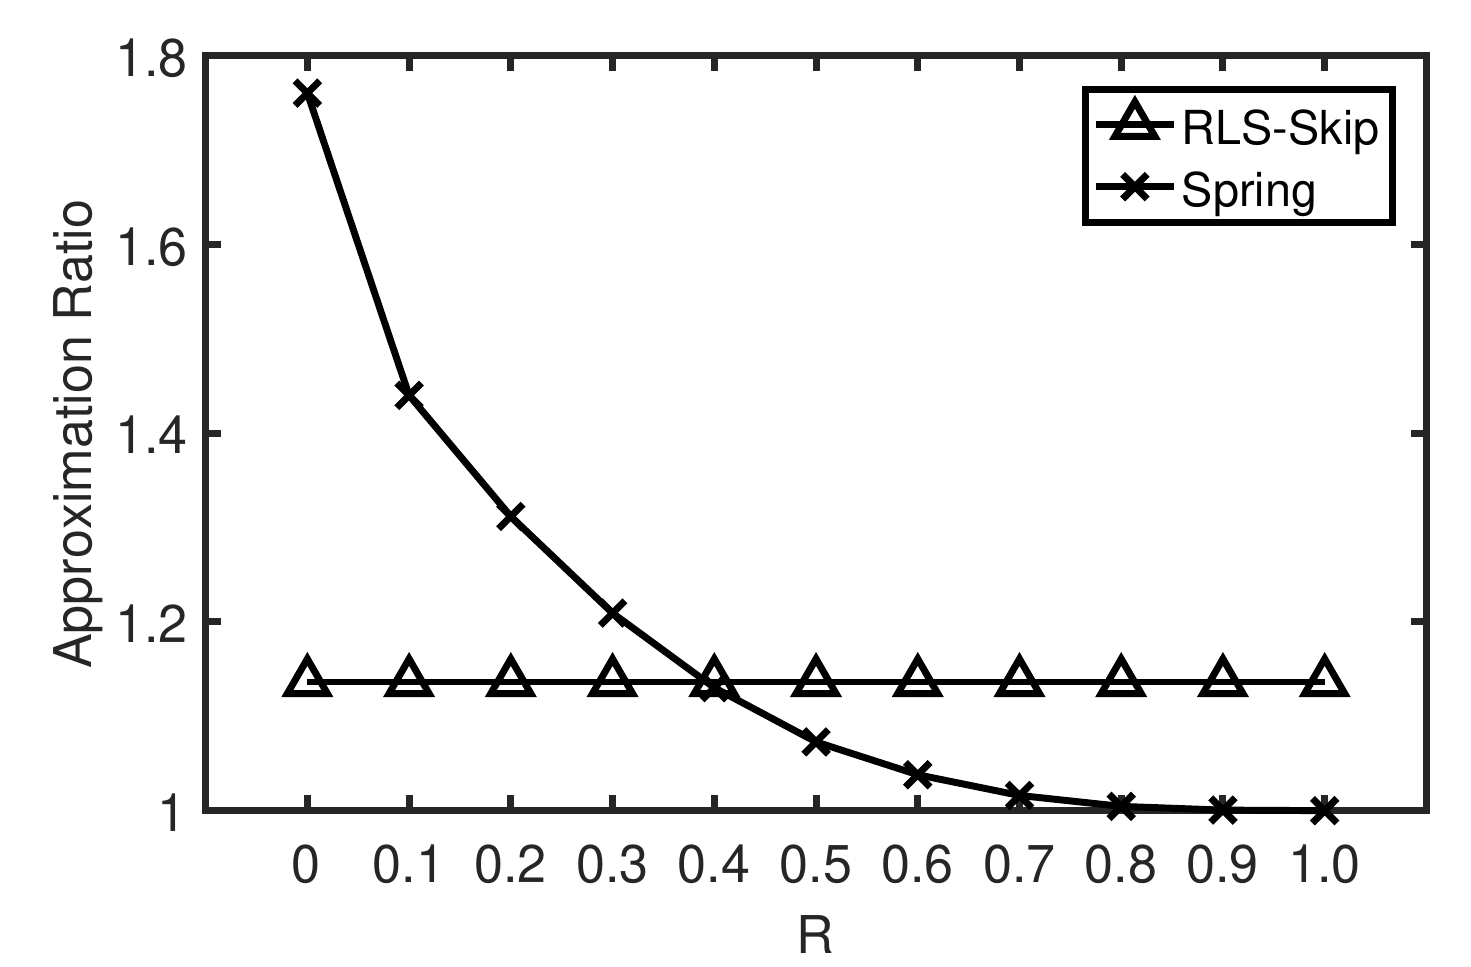}
		\end{minipage}
		&
		\begin{minipage}{4cm}
			\includegraphics[width=4.15cm]{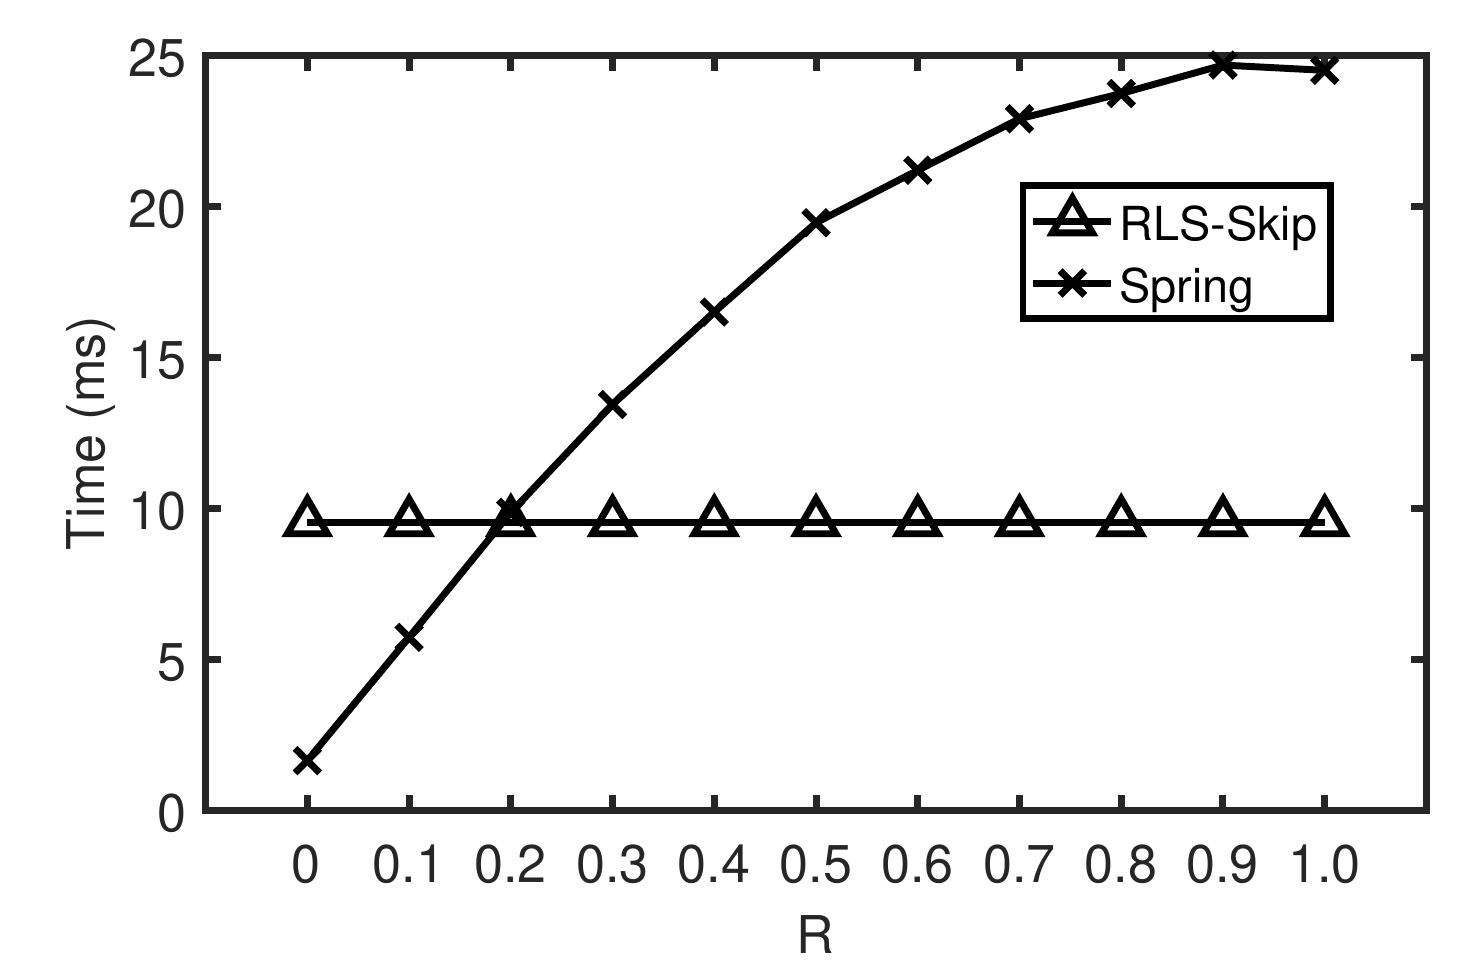}
		\end{minipage}
		&
		\begin{minipage}{4cm}
			\includegraphics[width=4.15cm]{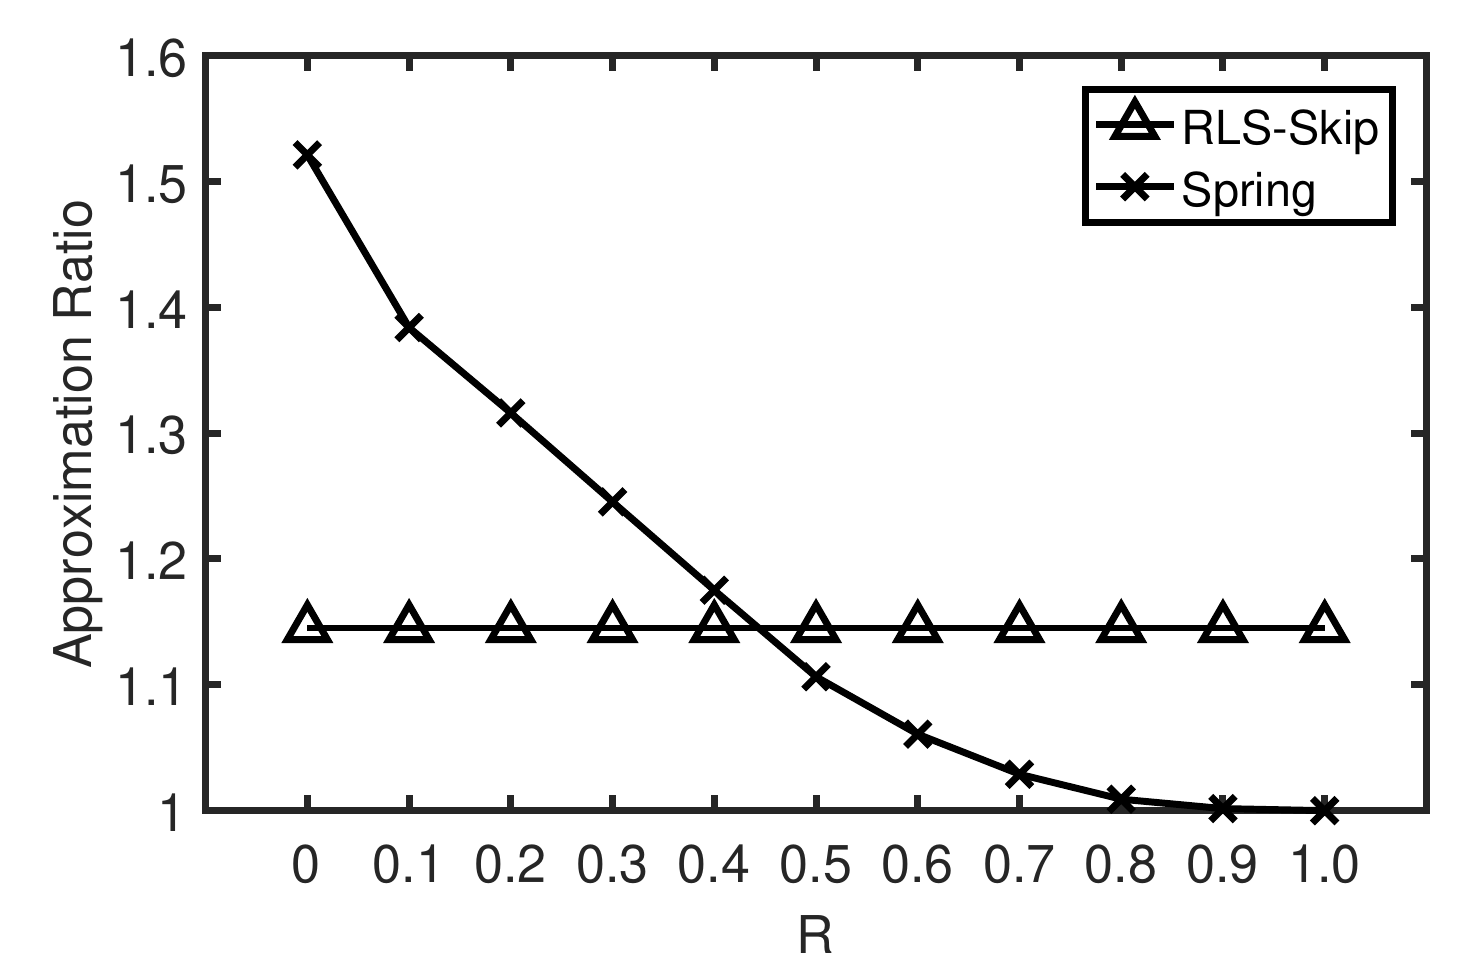}
		\end{minipage}
		&
		\begin{minipage}{4cm}
			\includegraphics[width=4.15cm]{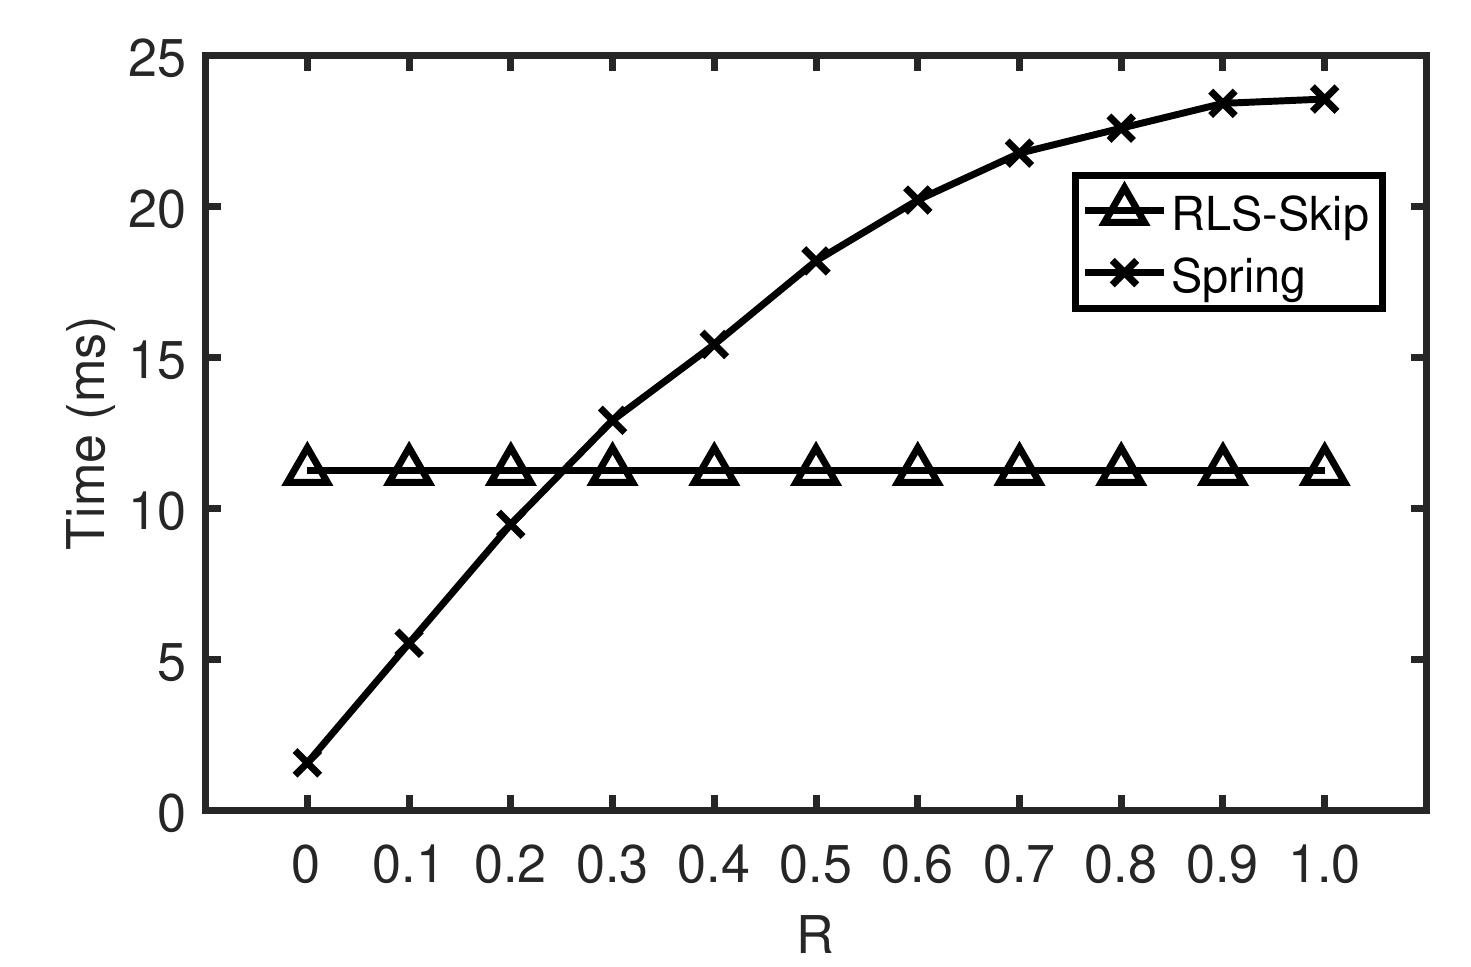}
		\end{minipage}
		\\
		\small (a) Approximation Ratio (DTW)
		&
		\small (b) Time Cost (DTW)
		&
		\small (c) Approximation Ratio (Frechet)
		&
		\small (d) Time Cost (Frechet)
		\\
		\begin{minipage}{4cm}
			\includegraphics[width=4.15cm]{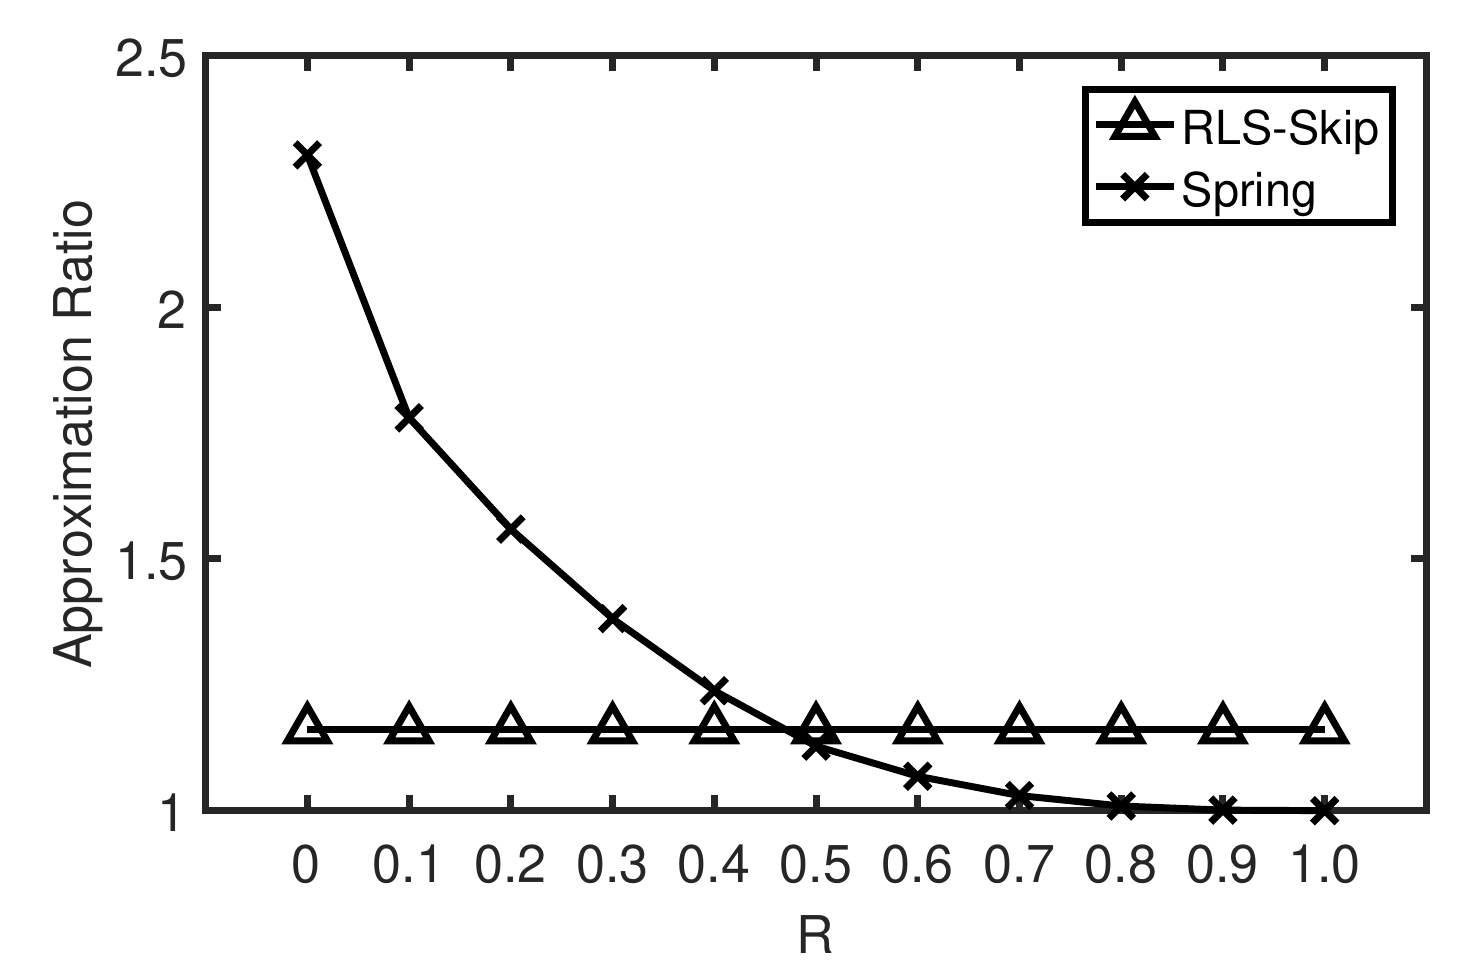}
		\end{minipage}
		&
		\begin{minipage}{4cm}
			\includegraphics[width=4.15cm]{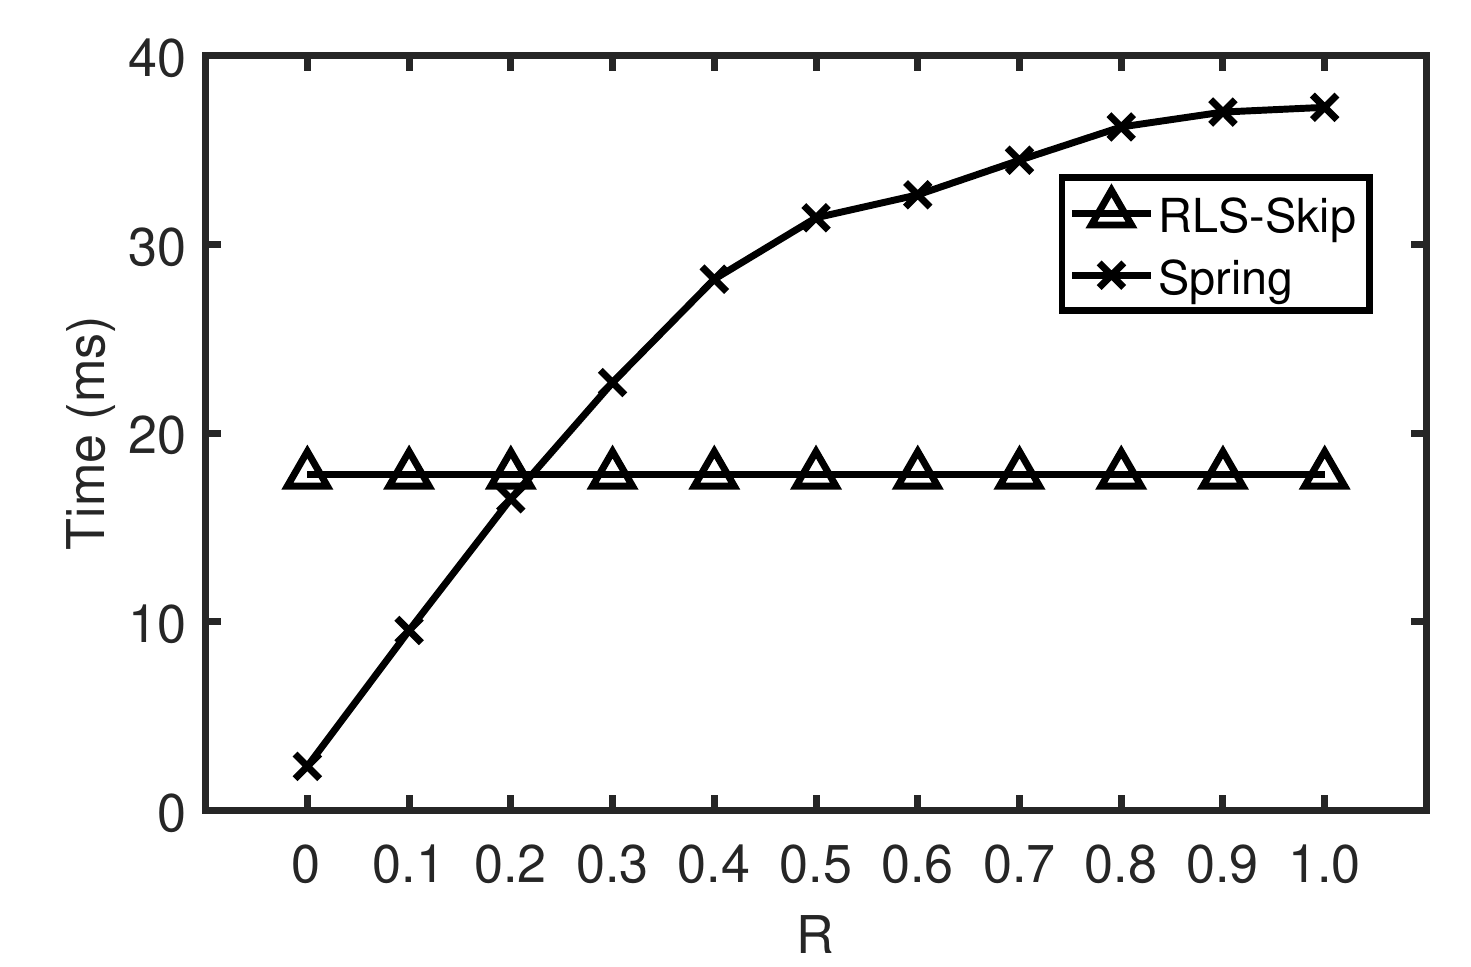}
		\end{minipage}
		&
		\begin{minipage}{4cm}
			\includegraphics[width=4.15cm]{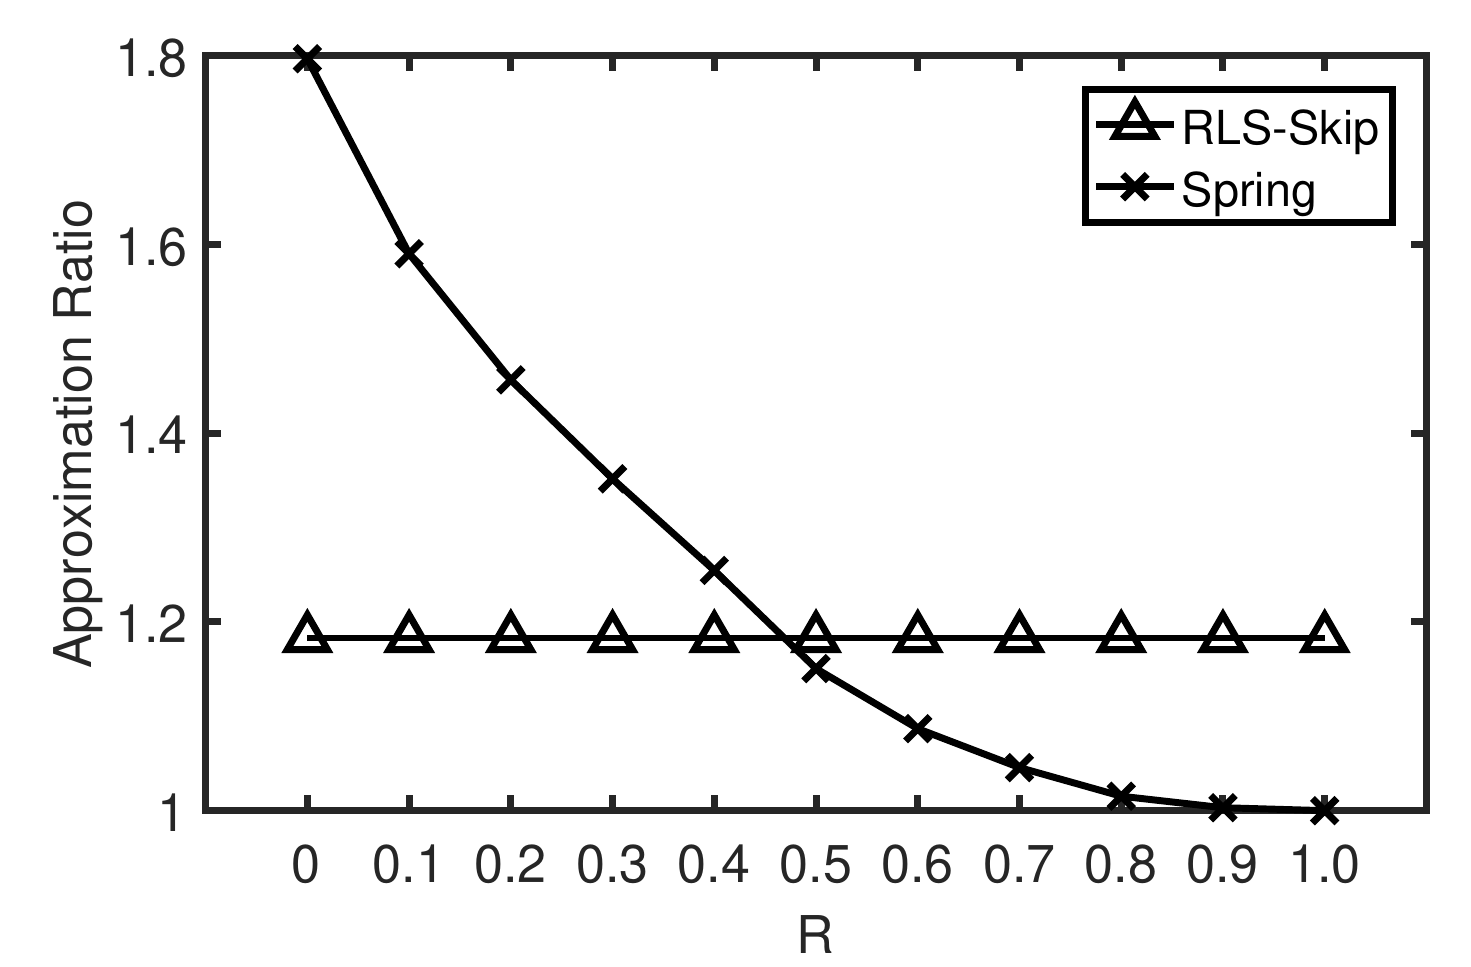}
		\end{minipage}
		&
		\begin{minipage}{4cm}
			\includegraphics[width=4.15cm]{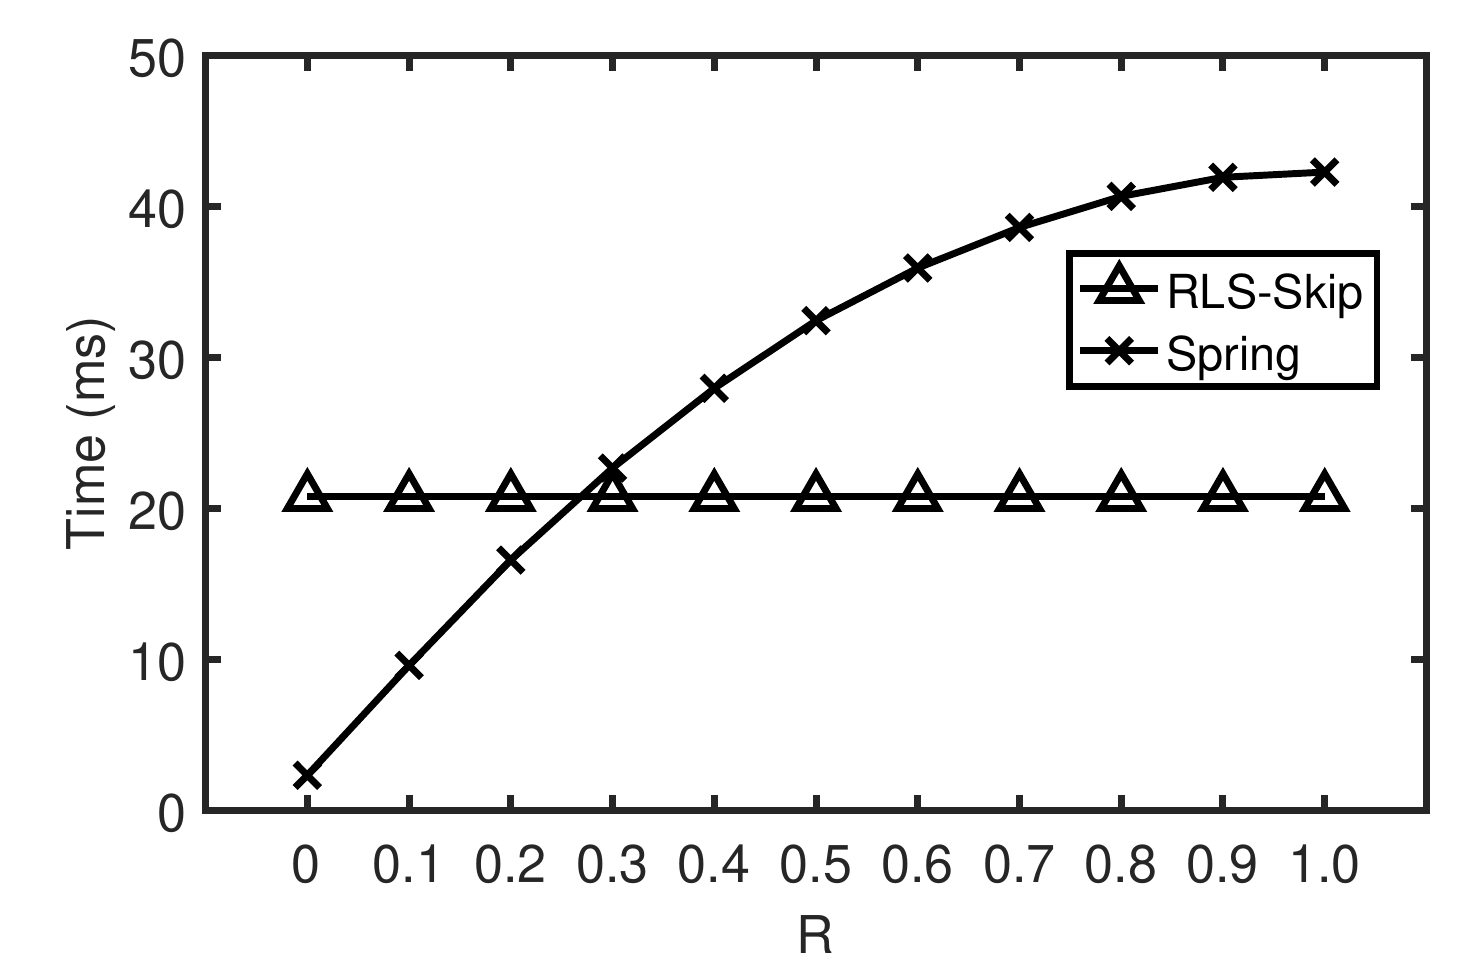}
		\end{minipage}
		\\
		\small (e) Approximation Ratio (DTW)
		&
		\small (f) Time Cost (DTW)
		&
		\small (g) Approximation Ratio (Frechet)
		&
		\small (h) Time Cost (Frechet)
		\\
		\begin{minipage}{4cm}
			\includegraphics[width=4.15cm]{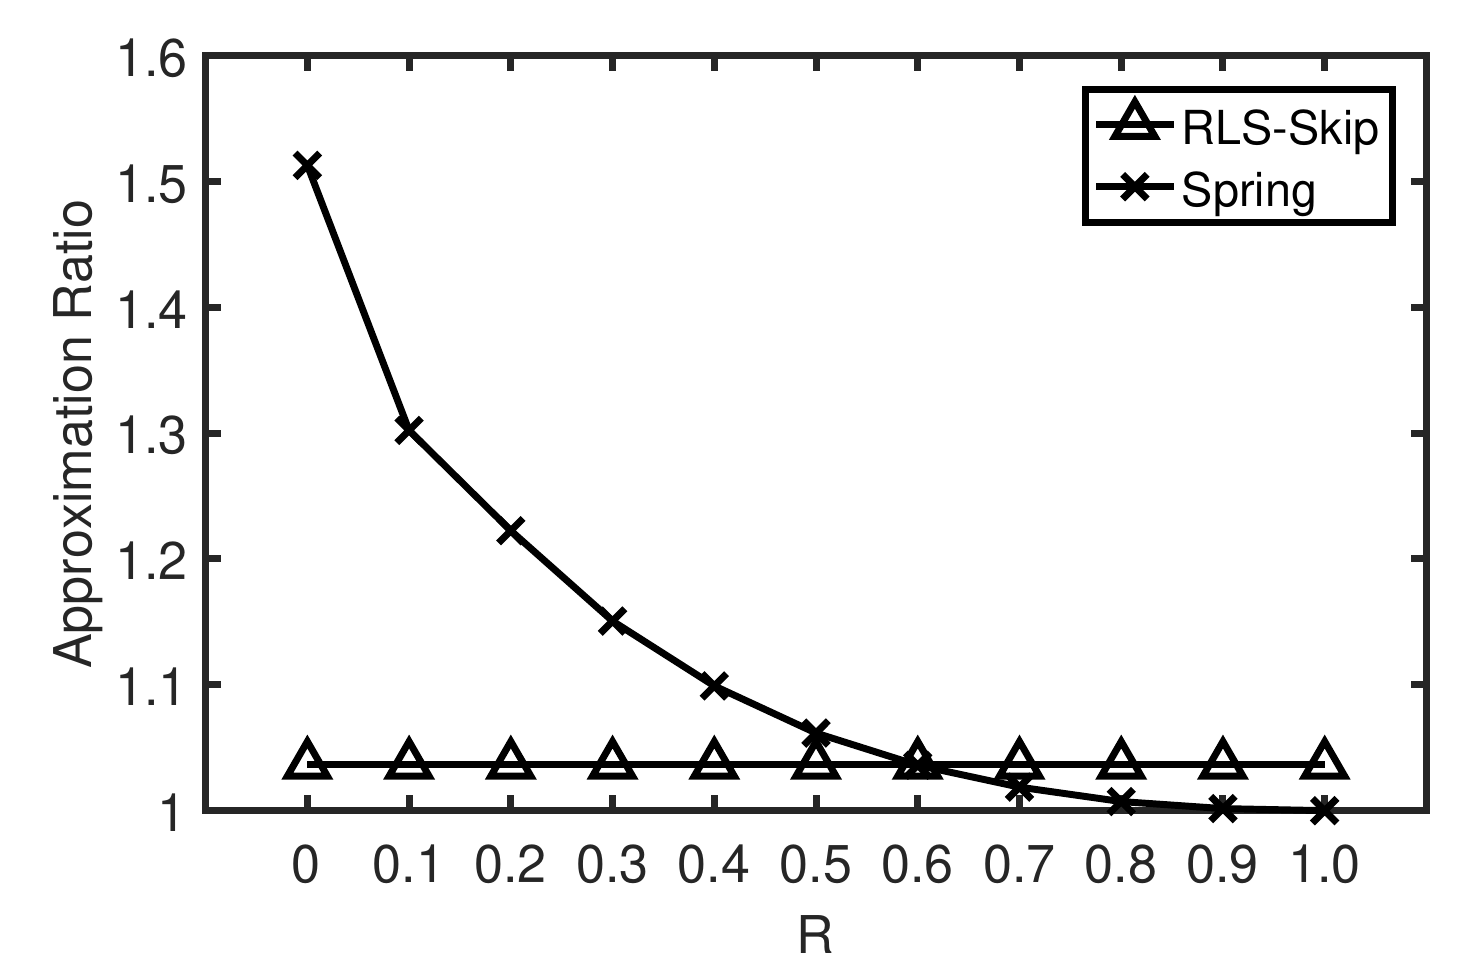}
		\end{minipage}
		&
		\begin{minipage}{4cm}
			\includegraphics[width=4.15cm]{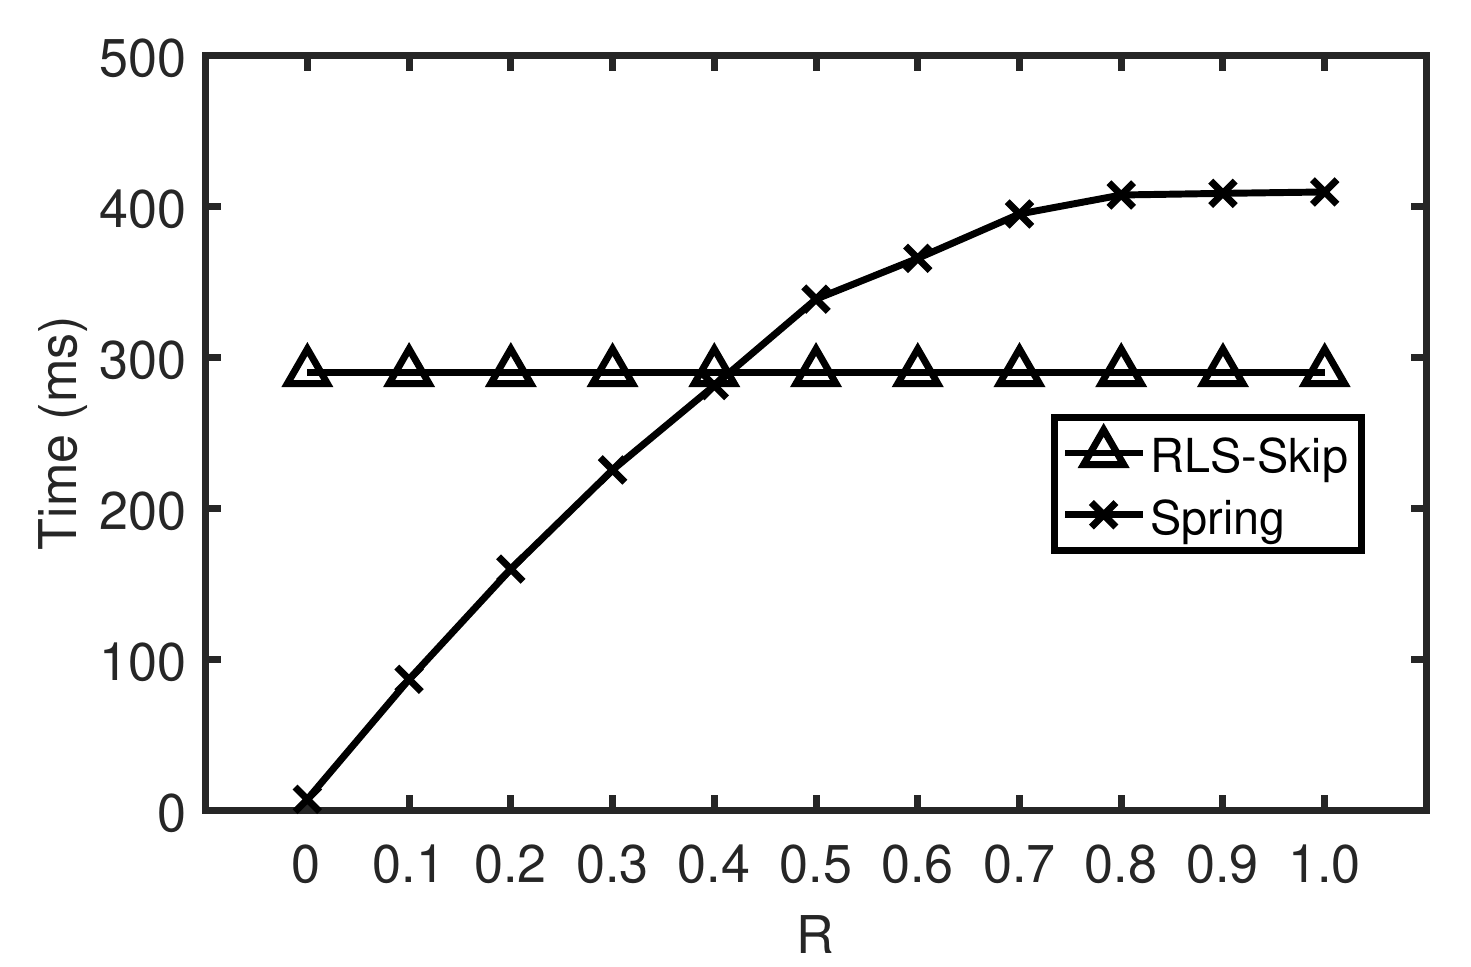}
		\end{minipage}
		&
		\begin{minipage}{4cm}
			\includegraphics[width=4.15cm]{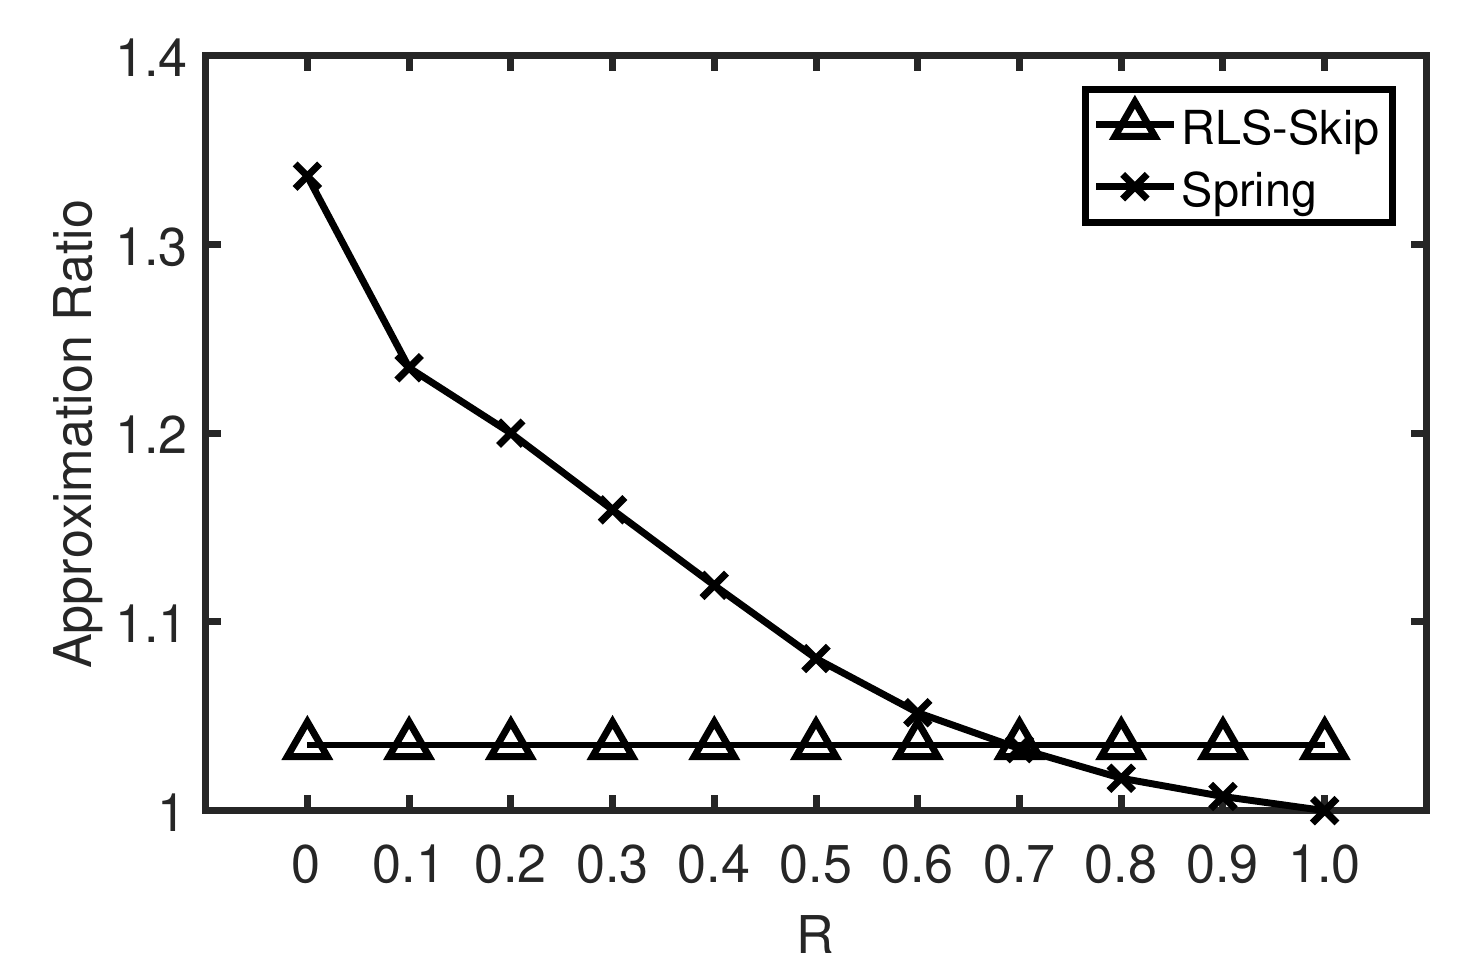}
		\end{minipage}
		&
		\begin{minipage}{4cm}
			\includegraphics[width=4.15cm]{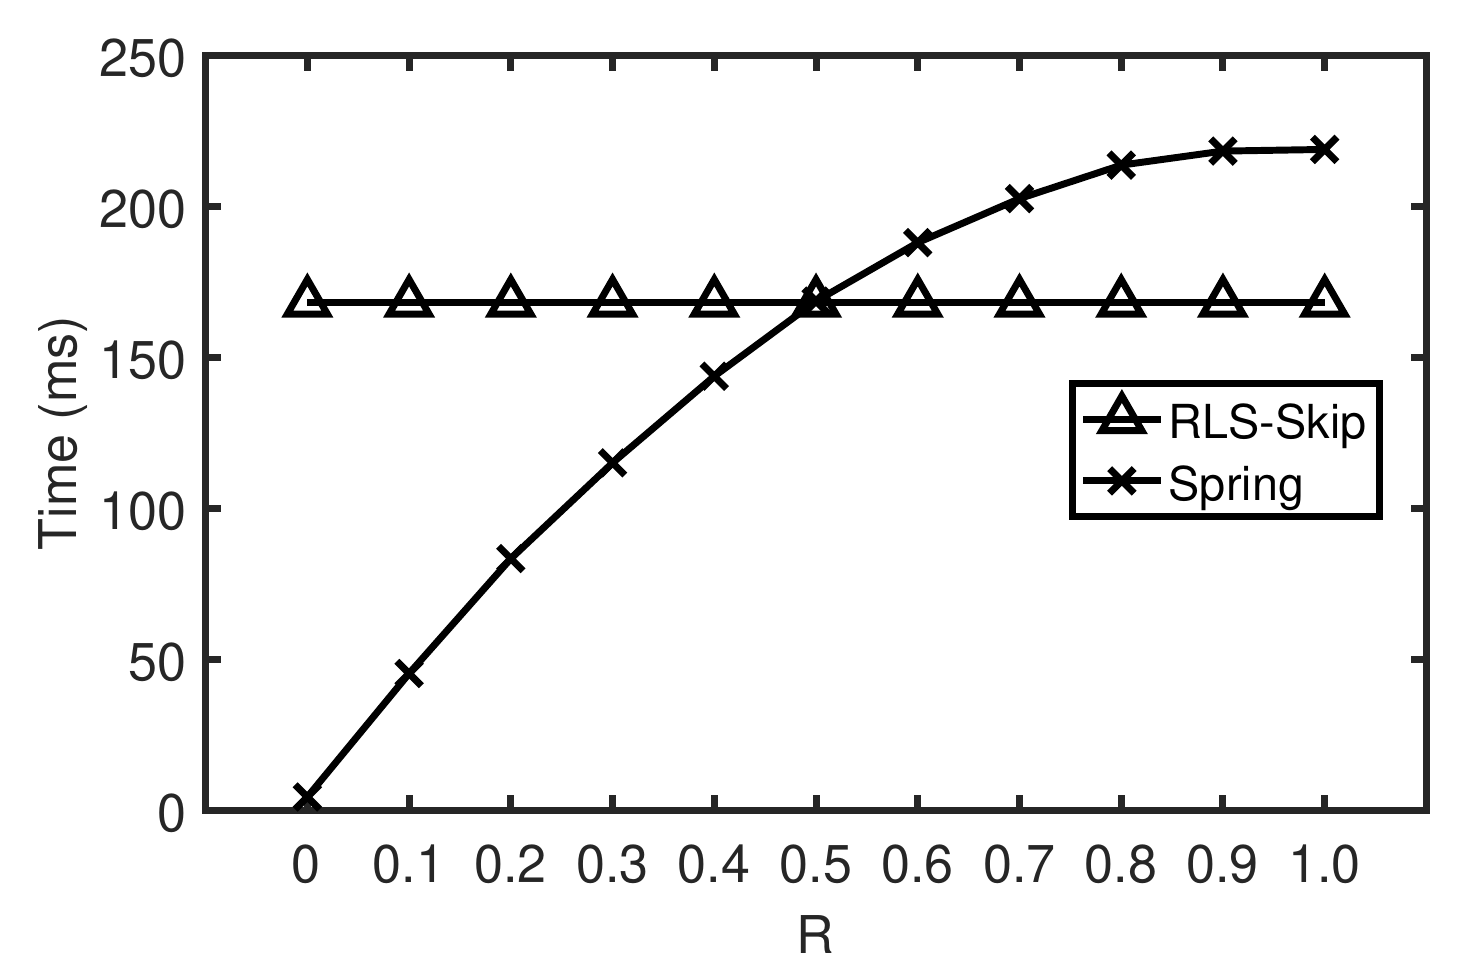}
		\end{minipage}
		\\
		\small (i) Approximation Ratio (DTW)
		&
		\small (j) Time Cost (DTW)
		&
		\small (k) Approximation Ratio (Frechet)
		&
		\small (l) Time Cost (Frechet)
	\end{tabular}
	%\vspace*{-2mm}
	\caption{Comparison with Spring on Porto (a)-(d), Harbin (e)-(h) and Sports (i)-(l).}
	%\vspace*{-3mm}
	\label{spring_result_full}
	%\vspace*{-0.5mm}
\end{figure*}
\fi

\begin{figure*}
	\hspace*{-.5cm}
	\centering
	\begin{tabular}{c c c c}
		\begin{minipage}{4cm}
			\includegraphics[width=4.15cm]{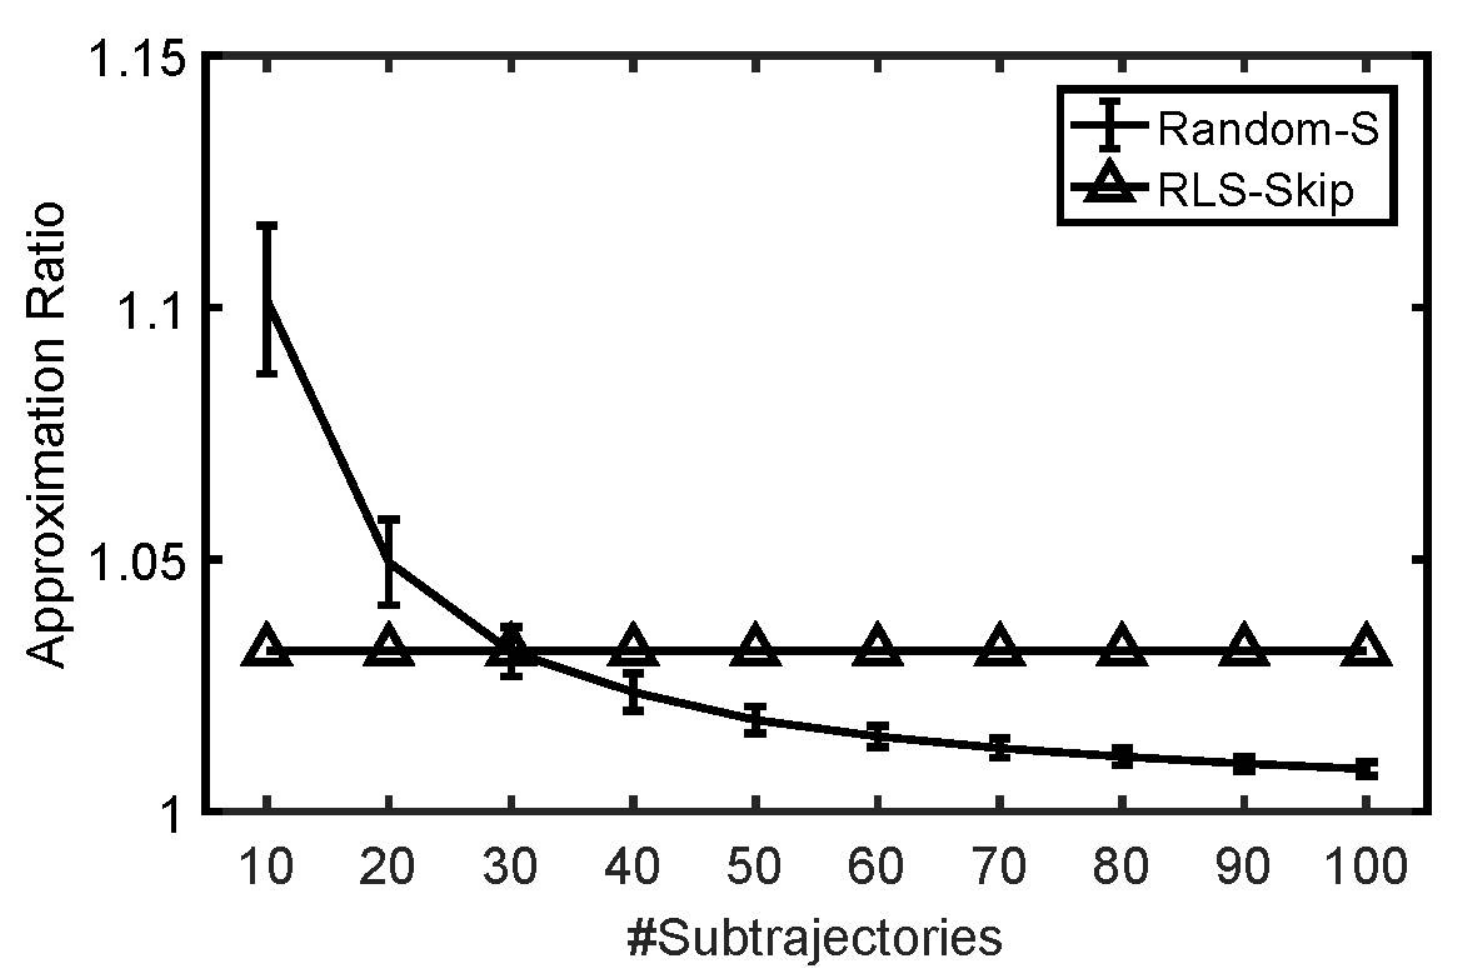}
		\end{minipage}
		&
		\begin{minipage}{4cm}
			\includegraphics[width=4.15cm]{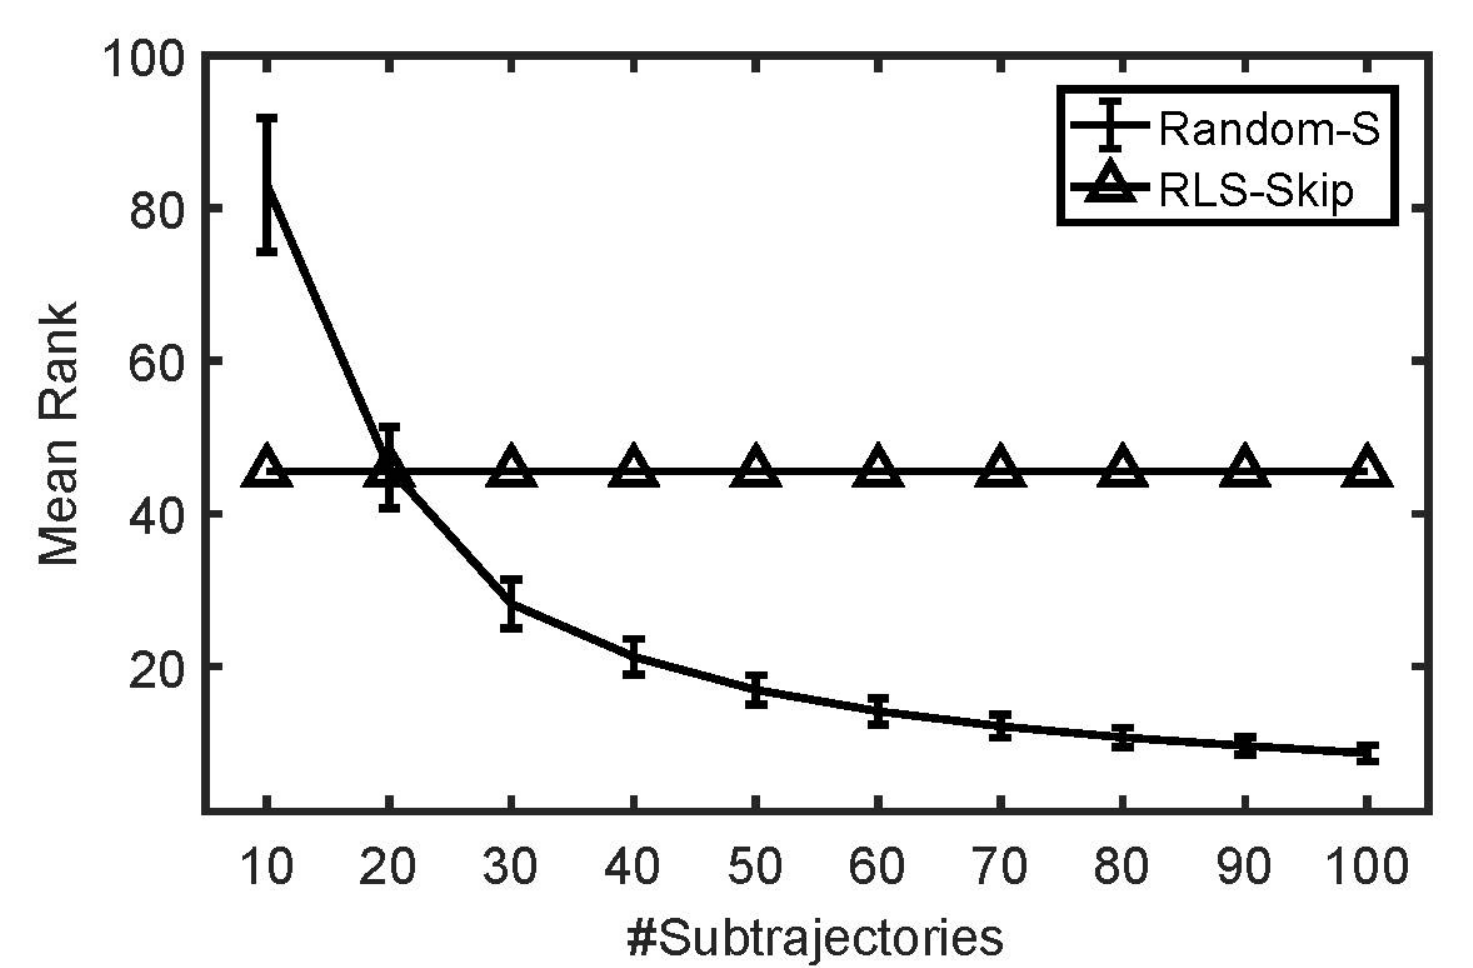}
		\end{minipage}
		&
		\begin{minipage}{4cm}
			\includegraphics[width=4.15cm]{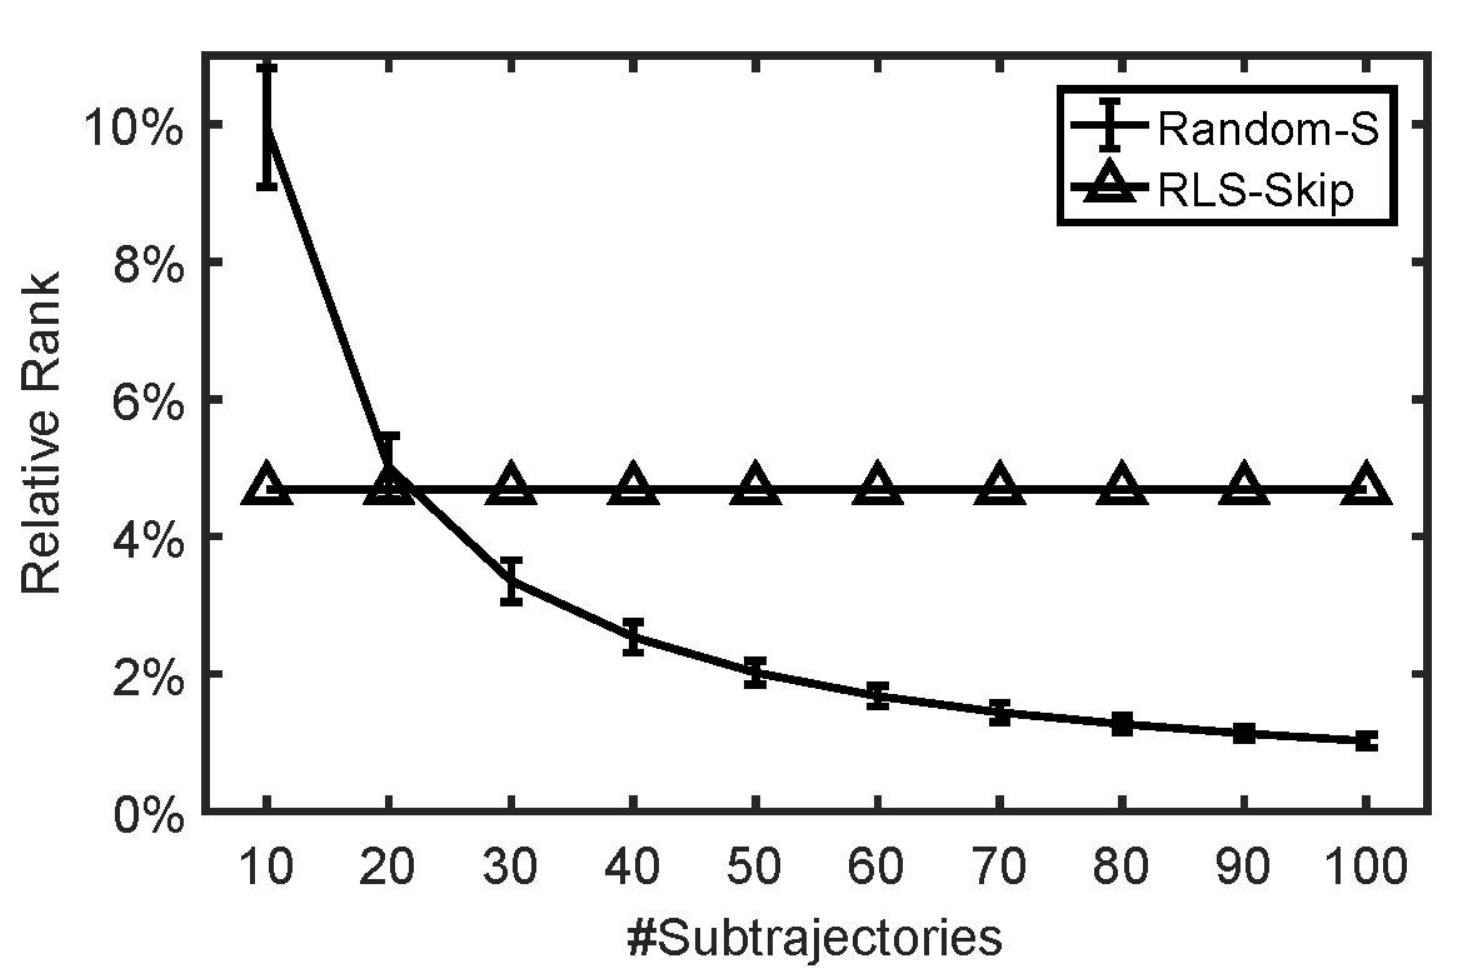}
		\end{minipage}
		&
		\begin{minipage}{4cm}
			\includegraphics[width=4.15cm]{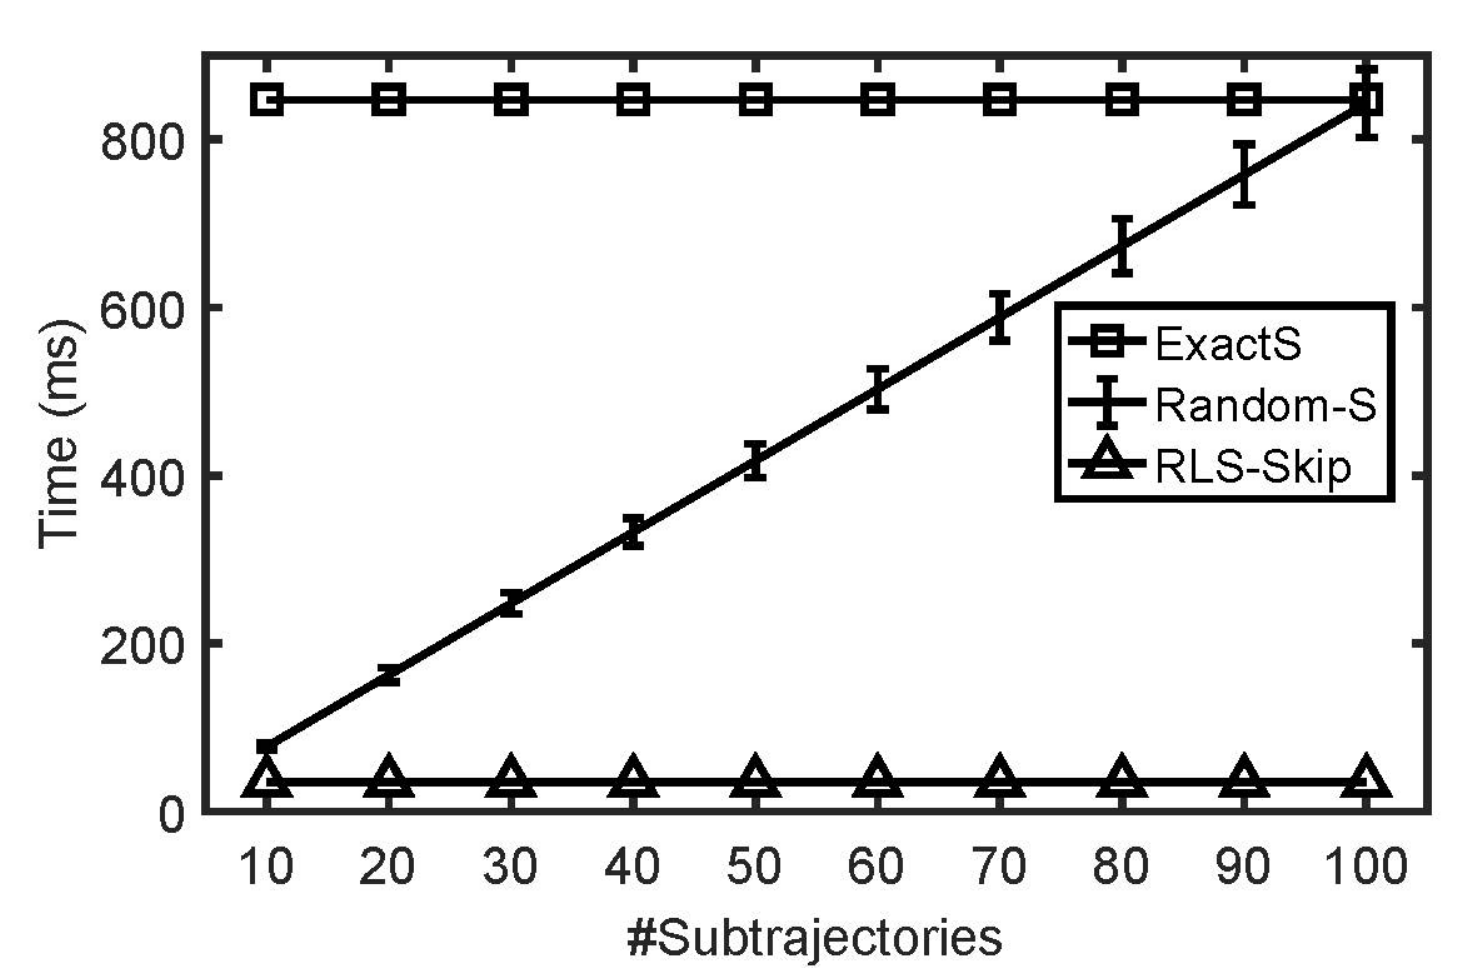}
		\end{minipage}
		\\
		\small (a) Approximation Ratio (DTW)
		&
		\small (b) Mean Rank (DTW)
		&
		\small (c) Relative Rank (DTW)
		&
		\small (d) Time Cost (DTW)
	\end{tabular}
	%\vspace*{-2mm}
	\caption{Comparison with Random-S.}
	%\vspace*{-3mm}
	\label{sampling-full}
	%\vspace*{-2mm}
\end{figure*}
